# Supplementary material for: LLM Unlearning Reveals a Stronger-Than-Expected Coreset Effect in Current Benchmarks
Source: arXiv:2504.10185 source file (2025-04-16)
Supplement: Supplementary file 1 [file appendix.tex]

\appendix

\setcounter{section}{0}
\setcounter{figure}{0}
\makeatletter

\section{Details of NPO and RMU}
\label{app: npormu}

\makeatother
\setcounter{table}{0}
\setcounter{equation}{0}

In this section, we provide details explaining the two main unlearning methods we consider in this paper.

\paragraph{Negative Preference Optimization (NPO).}

NPO \citep{zhang2024negative} reduces the model’s preference for the forget set $\Df$ by treating it analogously to negative responses in preference optimization, but omitting the positive response term. This yields the following loss function, which has been shown to achieve lower divergence rates compared to various other unlearning approaches:
\begin{align}
  & \ell_{\mathrm{NPO}}(\boldsymbol{\theta}) =  \mathbb E_{(x,y) \in \Df} \underbrace{\left [    - \frac{2}{\beta} \log \sigma  \left ( - \beta \log \left ( \frac{\pi_{\btheta} (y | x) }{\pi_{\mathrm{ref}} (y | x)}\right ) \right ) 
    \right ]}_{\lf \  \text{specified in}  \ \eqref{eq: LLM_MU}}
\label{eq:NPO}
\end{align}
where $\sigma (t) = 1/(1+e^{-t})$ is the sigmoid function, $\beta > 0 $ is a hyperparameter. Minimizing the above forget loss drives  the model to be unlearned $\pi_{\btheta}$ \textit{away} from the reference model $\pi_{\mathrm{ref}}$ for the samples from the forget set. In NPO, the retain loss $\lr$ is simply the prediction loss \textit{i.e.} the cross entropy loss between $x$ and $y$, which are obtained from $\Dr$.

\paragraph{Representation Misdirection Unlearning (RMU).}
RMU \citep{li2024wmdp} seeks to degrade the model's internal representations for the forget set, thereby reducing its ability to recall or generate undesired knowledge. Specifically, it aligns the hidden state activations of the unlearned model at a given layer $l$ (denoted $\pi_{\btheta}^l$) with a random unit vector $\mathrm{u}$, where each component of $\mathrm{u}$ is sampled independently and uniformly from $[0,1)$. In contrast to NPO, RMU also includes a retain loss that ensures the model’s representations on the retain dataset remain consistent with those of the reference (pre-unlearned) model. Considering $z_f$ and $z_r$ to be samples from the forget and retain set respectively,this is formalized as follows:
% \SL{[In the above, $z_f$ and $z_r$ were not defined.]}
%
% RMU \citep{li2024wmdp} which aims to degrade the representation of the unlearned model for the forget set. This degradation is mainly done by making the hidden state activations of the unlearned model at some layer $l$ (denoted by $\pi_{\btheta}^l$) to be similar to a random unit vector $\mathrm{u}$, where each value is independently and uniformly sampled from $[0,1)$.
% Unlike NPO, the retain loss here enforces alignment of the unlearned model representation with that of the reference model for the retain dataset. This is obtained in the following way:
\begin{align}
  & \ell_{\mathrm{RMU}}(\boldsymbol{\theta}) =  
  \mathbb E_{z_f \in \Df} \underbrace{\left [ \frac{1}{\mathrm{L_f}}\sum_{\text{token} \ t\in z_f} \|  \pi_{\btheta}^l (t) - c \cdot \mathrm{u}\|_2^2
    \right ]}_{\lf \  \text{specified in}  \ \eqref{eq: LLM_MU}} + \lambda
  \mathbb E_{z_r \in \Dr} \underbrace{\left [ \frac{1}{\mathrm{L_r}}\sum_{\text{token} \ t\in z_r} \|  \pi_{\btheta}^l (t) -\pi_{\mathrm{ref}}^l (t)\|_2^2
    \right ]}_{\lr \  \text{specified in}  \ \eqref{eq: LLM_MU}}
\label{eq:RMU}
\end{align}
where $\mathrm{L_f}$, $\mathrm{L_r}$ are the number of tokens in $z_f$, $z_r$ respectively and  $c$ controls the strength of $\mathbf u$.

\section{Detailed Unlearning Setup}
\label{app: epochs}

% \setcounter{section}{0}
% \setcounter{figure}{0}
% \makeatletter 

\makeatother
\setcounter{table}{0}
\setcounter{equation}{0}

% Note that this does not use the full forget set and thus
We present the detailed unlearning setups for different settings in \reftab{tab: app_setting}.
It is worth noting that 
the first 600 samples of WMDP-Bio and WMDP-Cyber are used as the \textit{full} forget set following \citep{li2024wmdp}. 
% We perform unlearning for NPO and RMU over these 600 samples with a batch size of 4, consistent with the original setting. 
For NPO, we perform unlearning for 140 steps with a batch size of 4, which is approximately $(140 \times 4 )/600 = 0.93$ epochs.

\begin{table}[htb]
\begin{center}
%\vspace{-2mm}
\caption{\small{Full forget set unlearning settings across different unlearning methods and benchmarks. 
% \SL{[talk to me on coreset setting.]}
%Here WMDP refers to both WMDP-Bio and WMDP-Cyber.
}}
\vspace{2mm}
\label{tab: app_setting}
\resizebox{0.6\textwidth}{!}{
\begin{tabular}{c|c|c|c|c}

\toprule[1pt]
% \midrule

\multicolumn{1}{c|}{\multirow{2}{*}{
\begin{tabular}{c}
   \textbf{Unlearning}
   \\
    \textbf{Benchmark} 
\end{tabular}
}} 
& 
\multicolumn{1}{c|}{\multirow{2}{*}{
\begin{tabular}{c}
   \textbf{Unlearning} \\
     \textbf{Method} 
\end{tabular}
}} 
& 
\multicolumn{1}{c|}{\multirow{2}{*}{
\begin{tabular}{c}
   \textbf{Model} 
\end{tabular}
}}
& 
\multicolumn{1}{c}{\multirow{2}{*}{
\begin{tabular}{c}
   \textbf{Epochs} 
\end{tabular}
}} 
& 
\multicolumn{1}{c}{\multirow{2}{*}{
\begin{tabular}{c}
      \textbf{Learning} \\
     \textbf{Rate} 
\end{tabular}
}}
\\
&&&\\
\midrule
\multicolumn{1}{c|}{\multirow{2}{*}{
\begin{tabular}{c}
  WMDP-Bio/Cyber
\end{tabular}
}} 
& 
RMU
&
\multicolumn{1}{c|}{\multirow{2}{*}{
\begin{tabular}{c}
   Zephyr-7B-$\beta$
\end{tabular}
}}
&
1
&
$5e-5$
\\
& 
NPO
&
&
0.93
&
$7e-6$
\\
\midrule
\multicolumn{1}{c|}{\multirow{2}{*}{
\begin{tabular}{c}
   MUSE-Books
\end{tabular}
}}
&
RMU
&
\multicolumn{1}{c|}{\multirow{2}{*}{
\begin{tabular}{c}
ICLM-7B
\end{tabular}
}}
&
\multicolumn{1}{c|}{\multirow{2}{*}{
\begin{tabular}{c}
1
\end{tabular}
}}
&
$1e-3$
\\
& 
NPO
&
&
&
$1e-5$

\\
\midrule
\multicolumn{1}{c|}{\multirow{2}{*}{
\begin{tabular}{c}
   MUSE-News 
\end{tabular}
}}
&
RMU
&
\multicolumn{1}{c|}{\multirow{2}{*}{
\begin{tabular}{c}
   LLaMA2-7B
\end{tabular}
}}
&
\multicolumn{1}{c}{\multirow{2}{*}{
\begin{tabular}{c}
10
\end{tabular}
}}
&

$1e-3$

\\
& 
NPO
&
&
&
$1e-5$
\\
% \midrule
\bottomrule[1pt]
\end{tabular}
}
% \vspace*{2mm}
\end{center}
\end{table}

Unless otherwise mentioned, we follow the standard hyperparameters in the above benchmarks. For MUSE-Books \citep{shi2024muse}, the reference model ICLM-7B is finetuned on Harry Potter books, while for MUSE-News, the reference model LLaMA2-7B is finetuned on BBC News articles. These reference models are available in the MUSE benchmark.  

 As mentioned in Sec.\,\ref{sec: problemstmnt}, the coreset effect emerges with a higher number of unlearning epochs. In \reftab{tab: app_setting_coreset}, we present the epoch numbers for each coreset setting. All other unlearning settings are the same as the full forget set unlearning.

\begin{table}[htb]
\begin{center}
%\vspace{-2mm}
\caption{\small{Coreset unlearning settings across different unlearning methods and benchmarks. 
% \SL{[talk to me on coreset setting.]}
%Here WMDP refers to both WMDP-Bio and WMDP-Cyber.
}}
\vspace{2mm}
\label{tab: app_setting_coreset}
\resizebox{0.6\textwidth}{!}{
\begin{tabular}{c|c|c|c}

\toprule[1pt]
% \midrule

\multicolumn{1}{c|}{\multirow{2}{*}{
\begin{tabular}{c}
   \textbf{Unlearning}
   \\
    \textbf{Benchmark} 
\end{tabular}
}} 
& 
\multicolumn{1}{c|}{\multirow{2}{*}{
\begin{tabular}{c}
   \textbf{Unlearning} \\
     \textbf{Method} 
\end{tabular}
}} 
& 
\multicolumn{1}{c|}{\multirow{2}{*}{
\begin{tabular}{c}
   \textbf{Coreset} \\
     \textbf{Ratio} 
\end{tabular}
}}
& 
\multicolumn{1}{c}{\multirow{2}{*}{
\begin{tabular}{c}
   \textbf{Epochs} 
\end{tabular}
}} 
% & 
% \multicolumn{1}{c}{\multirow{2}{*}{
% \begin{tabular}{c}
%       \textbf{Learning} \\
%      \textbf{Rate} 
% \end{tabular}
% }}
\\
&&&\\
\midrule
\multicolumn{1}{c|}{\multirow{3}{*}{
\begin{tabular}{c}
  WMDP-Bio/Cyber
\end{tabular}
}} 
& 
\multicolumn{1}{c|}{\multirow{3}{*}{
\begin{tabular}{c}
  RMU
\end{tabular}
}} 
&
10\%
&
10
% &
% $5e-5$
\\
& 
&
5\%
&
20
% &
% $7e-6$
\\
&&
1\%
&
100
\\
\midrule

\multicolumn{1}{c|}{\multirow{3}{*}{
\begin{tabular}{c}
  WMDP-Bio/Cyber
\end{tabular}
}} 
& 
\multicolumn{1}{c|}{\multirow{3}{*}{
\begin{tabular}{c}
  NPO
\end{tabular}
}} 
&
10\%
&
9.33
% &
% $5e-5$
\\
& 
&
5\%
&
18.67
% &
% $7e-6$
\\
&&
1\%
&
93.33
\\
\midrule

\multicolumn{1}{c|}{\multirow{2}{*}{
\begin{tabular}{c}
   MUSE-Books
\end{tabular}
}}
&
\multicolumn{1}{c|}{\multirow{2}{*}{
\begin{tabular}{c}
   RMU
\end{tabular}
}}
&
10\%
&
10
% &
% $1e-3$
\\
& 
&
5\%
&
20
\\
\midrule

\multicolumn{1}{c|}{\multirow{2}{*}{
\begin{tabular}{c}
   MUSE-Books
\end{tabular}
}}
&
\multicolumn{1}{c|}{\multirow{2}{*}{
\begin{tabular}{c}
   NPO
\end{tabular}
}}
&
10\%
&
7
% &
% $1e-3$
\\
& 
&
5\%
&
8
\\
\midrule

\multicolumn{1}{c|}{\multirow{2}{*}{
\begin{tabular}{c}
   MUSE-News
\end{tabular}
}}
&
\multicolumn{1}{c|}{\multirow{2}{*}{
\begin{tabular}{c}
   RMU
\end{tabular}
}}
&
10\%
&
100
% &
% $1e-3$
\\
& 
&
5\%
&
200
\\
\midrule

\multicolumn{1}{c|}{\multirow{2}{*}{
\begin{tabular}{c}
   MUSE-News
\end{tabular}
}}
&
\multicolumn{1}{c|}{\multirow{2}{*}{
\begin{tabular}{c}
   NPO
\end{tabular}
}}
&
10\%
&
5
% &
% $1e-3$
\\
& 
&
5\%
&
12
\\
% \midrule
\bottomrule[1pt]
\end{tabular}
}
% \vspace*{2mm}
\end{center}
\end{table}

\section{Details of Coreset Selection Methods}
\label{app: coreset_selection}

\makeatother
\setcounter{table}{0}
\setcounter{equation}{0}

In this section, we present additional details of the heuristic data selection methods as presented in Sec.\,\ref{sec: consistency}.
Though these methods were primarily developed for non-LLMs, we adapt them to our unlearning process as detailed below.

\paragraph{\grand{}.} 
The main rationale behind this method \citep{paul2021deep} is that the importance of each sample $z_f$ from the forget set is captured by the expected gradient norm of the loss associated with that sample, where the expectation is taken over the unlearning trajectory. Thus the \grand{} score is given by:
\begin{align}
\begin{array}{l}
  \chi(z_f) =  \mathbb E_{\btheta_t} \| \nabla_{\btheta_t} [\lf(z_f; \btheta_t) + \lambda \lr( z_r; \btheta_t) ] \|_2 \ ; \ \text{where} \ z_f \sim \Df, ~~z_r \sim \Dr
\end{array}
\label{eq:grand}
\end{align}
Here $\lf$ and $\lr$ are specified in \eqref{eq: LLM_MU}, where $\lf$ changes according to the unlearning method as specified before. In our experiments, we consider the trajectory of unlearning for 10 epochs for the purpose of computing the above expectation.
% \SP{I will check if their theorems hold here. I will check and update the above later. But if anyone has time, kindly check.}

\paragraph{Moderate.}   
The moderate coreset selection method \citep{xia2022moderate} was developed in the classification setting where samples were divided into clusters according to their classes. Using a well-trained model, the class center of each class is calculated using the hidden state representations of the penultimate layer of the corresponding samples.
Since our setting does not involve class labels, we cluster the forget samples into four groups using K-means, based on their penultimate-layer representations extracted from the reference (pre-unlearned) model. For each cluster, we compute its centroid and rank the samples by their distance to the respective centroid. To select representative data points, we choose those whose distances are closest to the median within their cluster.

\paragraph{\mink{}.}
The \mink{} method \citep{shi2024detecting} was developed to ascertain whether a given text appears in the original pretraining dataset. We use this metric as a data selection method for unlearning under the notion that data points not encountered during training are less influential in the unlearning process. In fact, in  \citep{shi2024detecting}, the authors demonstrated that the \textsc{Min-K\%} metric can be used as an effective indicator for assessing removal of knowledge after unlearning. 

For a given datapoint $z$, we calculate the log-likelihood of each token and choose a set of top $40\% (\text{K} = 40)$ of tokens with lowest value, called $\text{Min-K\%}(z)$. Then the score for $z$ is calculated as:
\begin{align}
\begin{array}{l}
  \mink{}(z) = \frac{1}{|\text{Min-K\%}(z)|} \sum_{z_i \in \text{Min-K\%}(z)}{ \log p(z_i | z_1, ..., z_{i-1}; \btheta)}
\end{array}
\label{eq:mink}
\end{align}

After computing the above scores for each sample $z$ in $\Df$, we choose samples with the top $\mathrm{p}$ scores to obtain our coresets. 
Thus, if we want to choose a 5\% coreset, then $\mathrm{p} = 0.05\times|\Df|$.

\section{Coreset Unlearning Performance on MUSE}
\label{app: muse_consistent}
\vspace*{-24mm}

\reftab{tab: muse} presents the coreset unlearning performance ofor MUSE across different coreset selection methods. Here we observe that performance of \random{}-based coresets are highly comparable to the full forget set performance, while also strongly outperforming the full forget set in many instances. 
For example, we observe a significant utility (UT) improvement for MUSE-Books using RMU for coresets as seen in Table \ref{tab: muse}, col.6. In fact, for \moderate-based 10\% coreset we see $\sim 12\%$ improvement in utility over the full forget set.

Additionally, we observe that for MUSE-News, the heuristic based 5\% coreset selection methods have UE (Knowmem) similar to that of the full forget set (as evidenced by Table \ref{tab: muse}, col.3). However, this is worse than the average performance of \random{}-based selection. This coupled with the high variance of the performance \random{}-based coresets points us to the fact that coreset selection is a non-trivial problem for such cases.
Nevertheless, the performance of \random{}-based coreset supports our strong coreset observation even at 5\% coreset selection regime.

\makeatother
\setcounter{table}{0}
\setcounter{equation}{0}

\begin{table}[htb]
\begin{center}
% \vspace{-2mm}
\caption{\small{Coreset-based unlearning performance (UE and UT, consistent with Fig. 2) using RMU and NPO on MUSE evaluated using LLaMA2-7B on News and ICLM-7B on Books. The table is presented in the same format as \reftab{tab: wmdp-bio}. Here `Retrain' refers to a model finetuned only on MUSE excluding the forget set.
} 
}
\vspace*{2mm}
\resizebox{\textwidth}{!}{
\begin{tabular}{c|c|ccc|c|ccc|c}
\toprule[1pt]
\midrule

\multicolumn{1}{c|}{\multirow{4.5}{*}{
\begin{tabular}{c}
   \textbf{Coreset} \\
     \textbf{Ratio}
\end{tabular}
}} 
&\multicolumn{1}{c|}{\multirow{4.5}{*}{
\begin{tabular}{c}
     \textbf{Unlearning} \\
     \textbf{Method}
\end{tabular}
}} 
& \multicolumn{4}{c|}{\textbf{RMU}} 
&  \multicolumn{4}{c}{\textbf{NPO}} \\
\cmidrule{3-10}
&& \multicolumn{3}{c|}{\textbf{UE}} 
& \multicolumn{1}{c|}{\textbf{UT}} 
& \multicolumn{3}{c|}{\textbf{UE}} 
& \multicolumn{1}{c}{\textbf{UT}} \\
\cmidrule{3-10}
&& \begin{tabular}{c}
   \textbf{VerbMem} \\
      ($\downarrow$) 
\end{tabular}
& \begin{tabular}{c}
   \textbf{KnowMem} \\
      ($\downarrow$) 
\end{tabular}
& \begin{tabular}{c}
   \textbf{PrivLeak} \\
      ($\rightarrow$ 0)
\end{tabular} 
& \begin{tabular}{c}
   \textbf{KnowMem} \\
      ($\uparrow$) 
\end{tabular}
& \begin{tabular}{c}
   \textbf{VerbMem} \\
      ($\downarrow$) 
\end{tabular}
& \begin{tabular}{c}
   \textbf{KnowMem} \\
      ($\downarrow$) 
\end{tabular}
& \begin{tabular}{c}
   \textbf{PrivLeak} \\
      ($\rightarrow$ 0)
\end{tabular} 
& \begin{tabular}{c}
   \textbf{KnowMem} \\
      ($\uparrow$) 
\end{tabular}
\\ 
\midrule
\multicolumn{10}{c}{\textbf{MUSE-Books}}\\
\midrule
0\% & No unlearning &
99.56  & 58.32  & -56.32   & 67.01
&
99.56  & 58.32  & -56.32   & 67.01
 \\
\midrule
0\% & Retrain &
14.30 & 28.90 & 0.00   & 74.50 
&
14.30 & 28.90 & 0.00   & 74.50 
 \\
\midrule
100\% & Full forget Set
& 5.38 %$_{\pm{0.17}}$ 
& 18.72 %$_{\pm{13.49}}$ 
&  -16.98 %$_{\pm{10.41}}$ 
& 40.34 %$ %_{\pm{24.50}}$  
& 0.00 %$ %_{\pm{0.00}}$ 
& 0.00 %$_{\pm{0.00}}$ 
&  -31.02 %$_{\pm{1.04}}$ 
& 31.33 %$_{\pm{3.67}}$ 
\\
\midrule
\multirow{4}{*}{
\begin{tabular}{c}
   10\% 
\end{tabular}
}
& \random{}
& 4.34$_{\pm{1.40}}$ 
& 23.86$_{\pm{10.79}}$ 
&  -12.79$_{\pm{4.86}}$ 
& 56.67$_{\pm{7.29}}$  
& 0.00$_{\pm{0.00}}$ 
& 0.00$_{\pm{0.00}}$ 
&  -27.09$_{\pm{2.22}}$ 
& 29.12$_{\pm{3.36}}$\\
&\grand{}
& 4.96
& 21.69
& 5.07
& 57.11
& 0.00
& 0.00
&  -25.28
& 37.54\\
& \moderate{}
& 5.72
& 9.02
& -19.84
& 33.44
& 0.00
& 0.00
& -28.42
& 36.55\\
%%%  Mink for NPO 0.5
& \mink{}
& 7.53
& 20.12
& -29.17
& 56.43
& 0.00
& 0.00
& -0.24
& 33.21 \\
\midrule
\multirow{4}{*}{
\begin{tabular}{c}
   5\% 
\end{tabular}
}
%%%  random for RMU 0.5
& \random{}
& 4.01$_{\pm{1.58}}$ 
& 19.37$_{\pm{6.75}}$ 
&  -18.61$_{\pm{1.88}}$ 
& 54.62$_{\pm{5.54}}$  

%%%  random for NPO 0.5
& 0.00$_{\pm{0.00}}$ 
& 3.48$_{\pm{0.56}}$ 
&  -8.97$_{\pm{8.03}}$ 
& 36.19$_{\pm{1.35}}$\\
&\grand{}
%%%  grand for RMU 0.5
& 5.69
& 28.00
& -37.66
& 59.21

%%%  grand for NPO 0.5
& 0.00
& 3.77
&  -15.71
& 40.15 \\  
& \moderate{}
%%%  Moderate for RMU 0.5
& 4.75
& 7.08
& -18.02
& 33.92

%%%  Moderate for NPO 0.5
& 0.00
& 3.35
&  -5.63
& 36.93\\ 
%%%  Mink for RMU 0.5
& \mink{}
& 4.20
& 37.48
& -0.12
& 67.76

%%%  Mink for NPO RMU 0.5
& 0.00
&  4.33
& -32.90
& 39.18\\

%%% MUSE NEWS
\midrule
\multicolumn{10}{c}{\textbf{MUSE-News}}\\
\midrule
0\% & No unlearning &
58.29  & 62.93  & -98.71    & 54.31
&
58.29  & 62.93  & -98.71    & 54.31
 \\
\midrule
0\% & Retrain &
20.75 & 33.32 & 0.00    & 53.79
&
20.75 & 33.32 & 0.00    & 53.79
\\
 \midrule
100\% & Full forget set
%%%  Random for RMU 1
& 21.00 
& 54.68 
&  1.80 
& 44.75 

%%%  Random for NPO 1
& 0.00 
& 47.96 
&  107.40 
& 37.86 
\\
\midrule
\multirow{4}{*}{
\begin{tabular}{c}
   10\% 
\end{tabular}
}
& \random{}
%%%  Random for RMU 0.1
& 29.97$_{\pm{2.50}}$ 
& 18.85$_{\pm{21.99}}$ 
&  -38.87$_{\pm{2.78}}$ 
& 50.23$_{\pm{1.67}}$  

%%%  Random for NPO 0.1
& 20.54$_{\pm{1.71}}$ 
& 42.30$_{\pm{1.26}}$ 
&  -99.58$_{\pm{0.14}}$ 
& 38.54$_{\pm{0.61}}$\\
&\grand{}
& 28.85
& 40.50
& -45.84
& 49.50
& 21.35
& 41.97
& -99.71
& 38.59
\\
& \moderate{}
& 32.62
& 38.40
& -36.44
& 52.77
& 19.26
& 42.46
& -99.78
& 37.99
\\
%%%  Mink for NPO 0.5
& \mink{}
& 31.67
& 2.02
& -15.95
& 50.14
& 23.59
& 43.85
& -98.14
& 40.66 \\
\midrule
\multirow{4}{*}{
\begin{tabular}{c}
   5\% 
\end{tabular}
}
%%%  random for RMU 0.5
& \random{}
& 20.15$_{\pm{7.50}}$ 
& 12.95$_{\pm{17.17}}$ 
&  -16.42$_{\pm{18.70}}$ 
& 40.93$_{\pm{4.32}}$

%%%  random for NPO 0.5
& 7.36$_{\pm{0.79}}$ 
& 34.28$_{\pm{1.92}}$ 
&  -76.38$_{\pm{7.46}}$ 
& 32.75$_{\pm{1.75}}$ \\
&\grand{}
%%%  grand for RMU 0.5
& 24.15
& 50.26
& -33.27
& 47.11

%%%  grand for NPO 0.5
& 3.51
& 32.71
& -1.85
& 31.65 \\  
& \moderate{}
%%%  Moderate for RMU 0.5
& 19.37
& 52.21
& -8.53
& 47.00

%%%  Moderate for NPO 0.5
& 3.19
& 38.24
& 16.50
& 35.57 \\ 
%%%  Mink for RMU 0.5
& \mink{}
& 28.83
& 49.21
& -33.74
& 43.94

%%%  Mink for NPO RMU 0.5
& 3.40
&  36.45
& 73.07
& 31.21\\

\midrule
\bottomrule
\end{tabular}
}
\label{tab: muse}
% \vspace*{-2mm}
\end{center}
\end{table}
\section{Prompt to Extract Keywords}
\label{app: prompt}

\makeatother
\setcounter{table}{0}
\setcounter{equation}{0}

% We use the following prompt to extract the relevant keywords from WMDP-Bio

\begin{prompt}{Prompt to Extract Keywords using LLM-as-a-Judge}\label{prompt:meta}
% \small
\textbf{System}:
\\
\\
You are an expert in chemistry, biology and diseases. I will provide you with a text, and your task is to carefully analyze each word and determine if it is related to chemistry or biology and disease. For every word that is related to chemistry, biology and disease, replace it with an asterisk (*) in the original text while keeping all other words unchanged. Think step by step and ensure accuracy in identifying only chemistry, biology and disease-related terms. Pay close attention to scientific terminology. Return the result in the following format:\\
\{\{ \\
"replaced\_text": "$<$text after replacing$>$",\\
"related\_words": ["word1", "word2", "word3", ...] \\
\}\} \\
Do \textbf{not} write any code. Use your linguistic and scientific knowledge to analyze the text.
\\
\\
\textbf{User}: 
\\
\\
{\color{blue}\{WMDP-Bio forget set\}}
\\
\\
\textbf{Assistant}:
\\
\\
{\color{blue}\{response\}}

\end{prompt}

\section{Additional Details of Keyword Explanation Experiment}
\label{app: keyword_overlap}

\makeatother
\setcounter{table}{0}
\setcounter{equation}{0}

%In addition to the demonstrating then unlearning effectiveness of keyword unlearned models as in Sec.\,\ref{sec: consistency}, we analyse the overlap between the keywords extracted from the full forget set and the \random{}-based coresets. 
In addition to demonstrating the unlearning effectiveness of keyword-based unlearned models in Sec.\,\ref{sec: consistency}, we further analyze the overlap between keywords extracted from the entire forget set (100\%) and those obtained from \random{}-based coresets. This comparison helps assess whether randomly selected coresets reliably capture the keywords in the full set.
For a particular coreset, let the keywords be denoted by $K_c$ and let all the keywords extracted be denoted $K_f$. Then for that coreset, we define the normalized overlap as $\frac{K_c \  \cap \  K_f}{|K_f|}$. As seen in \reffig{fig: overlap}, the overlapping keywords are higher than the fraction of data present in the coreset. 
his suggests that even information-agnostic random selection can yield a surprisingly high ratio of keyword overlap with the full forget set. For instance, a 5\% \random{}-based coreset captures approximately {14\%} of the full set’s keywords. We hypothesize that this amplified presence of high-impact keywords is a key factor enabling effective unlearning, even when using such a small, randomly selected subset.
% \SP{@SL: Please help me conclude here.}
%This potentially points to the reason for success of coreset selected 

%\begin{wrapfigure}{r}{105mm}
\begin{figure}[htb]
\centering
 \includegraphics[width=.4\textwidth]{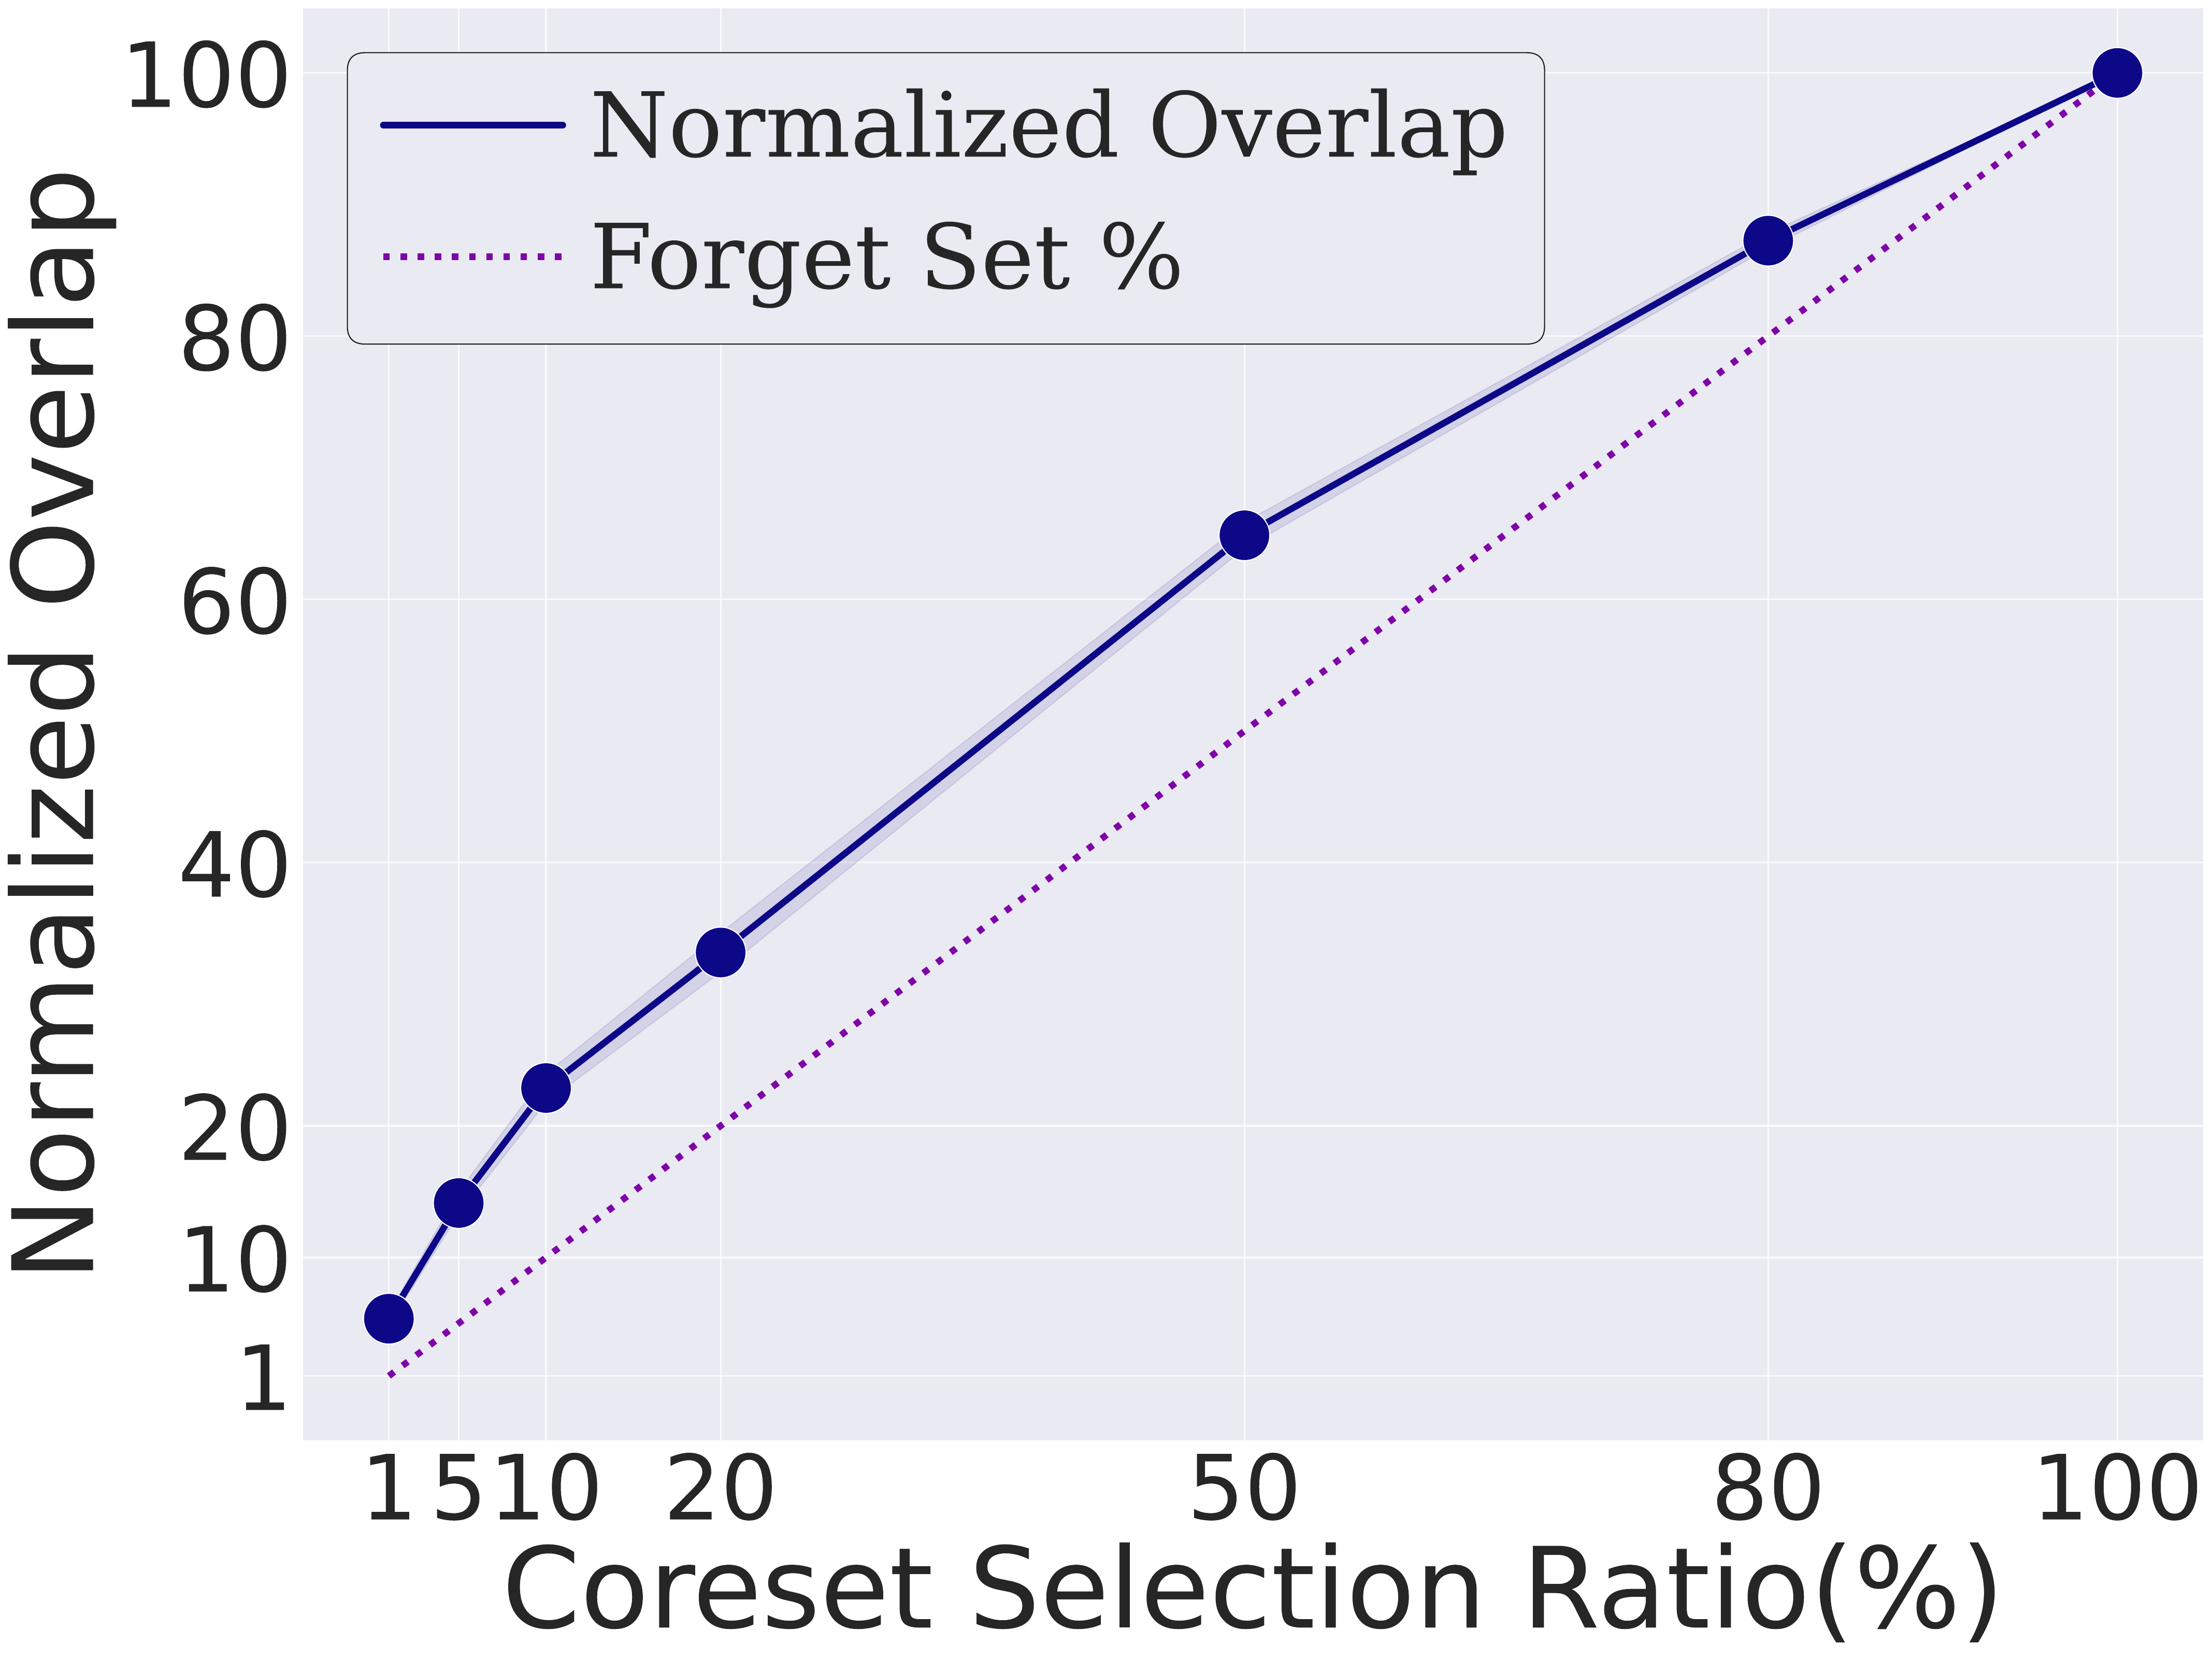}
\vspace*{-2mm}
\caption{\small{
Normalized overlapping ratio (\%) of keywords between \random{}-based coresets and the full forget set for WMDP-Bio. The dotted line represents the percentage of data present in the coreset from the forget set. Results are reported in the form $a \pm 2b$, where $a$ is the mean and $b$ is the standard deviation, computed over 3 independent trials.
}}
  \label{fig: overlap}
  %\vspace*{-6mm}
%\end{wrapfigure}
\end{figure}

% \paragraph{Additional utility evaluation of unlearned LLMs using coresets.}
\section{Additional Utility Evaluation of Unlearned LLMs Using Coresets.}
\label{app: utility}

\makeatother
\setcounter{table}{0}
\setcounter{equation}{0}

As shown by the coreset unlearning performance in standard benchmarks (Sec.\,\ref{sec: consistency}), a surprising finding is that coreset unlearning can achieve lossless UE. This naturally raises the question: Could coreset unlearning offer utility benefits as it negates the influence of fewer forget data points, thereby better preserving the model’s performance on general tasks? However, we did not observe a clear UT advantage in existing benchmarks, likely due to the limited scope of their utility evaluations, \textit{e.g.}, MMLU for WMDP and KnowMem on the retain set for MUSE, which may not fully capture the broader utility landscape of the coreset-unlearned models.

Therefore, we conduct additional utility evaluations of coreset-unlearned models, focusing on two tasks inspired by the emergent abilities of LLMs \citep{wei2022emergent}:
(1) a math addition/subtraction task involving 2–5 digit arithmetic that is orthogonal to the unlearning objective, and
(2) the TruthfulQA task that assesses factual consistency and truthfulness in LLM responses and may be inadvertently affected by unlearning.
In \reffig{fig: additional utility}, we report the zero-shot accuracy of the aforementioned utility metrics for \random{}-based coreset-unlearned models using RMU and NPO on WMDP. RMU consistently maintains strong utility across all evaluations, regardless of the coreset selection ratio. In contrast, NPO shows higher variance; however, we observe that for $n$-digit addition and subtraction, performance may benefit from using a 10\% coreset in the WMDP-Cyber setting.

\begin{figure}[htb]
\centering
\begin{tabular}{ccc}
 %\hspace*{-8mm}
  % \hspace*{-2mm}
 \includegraphics[width=.23\textwidth]{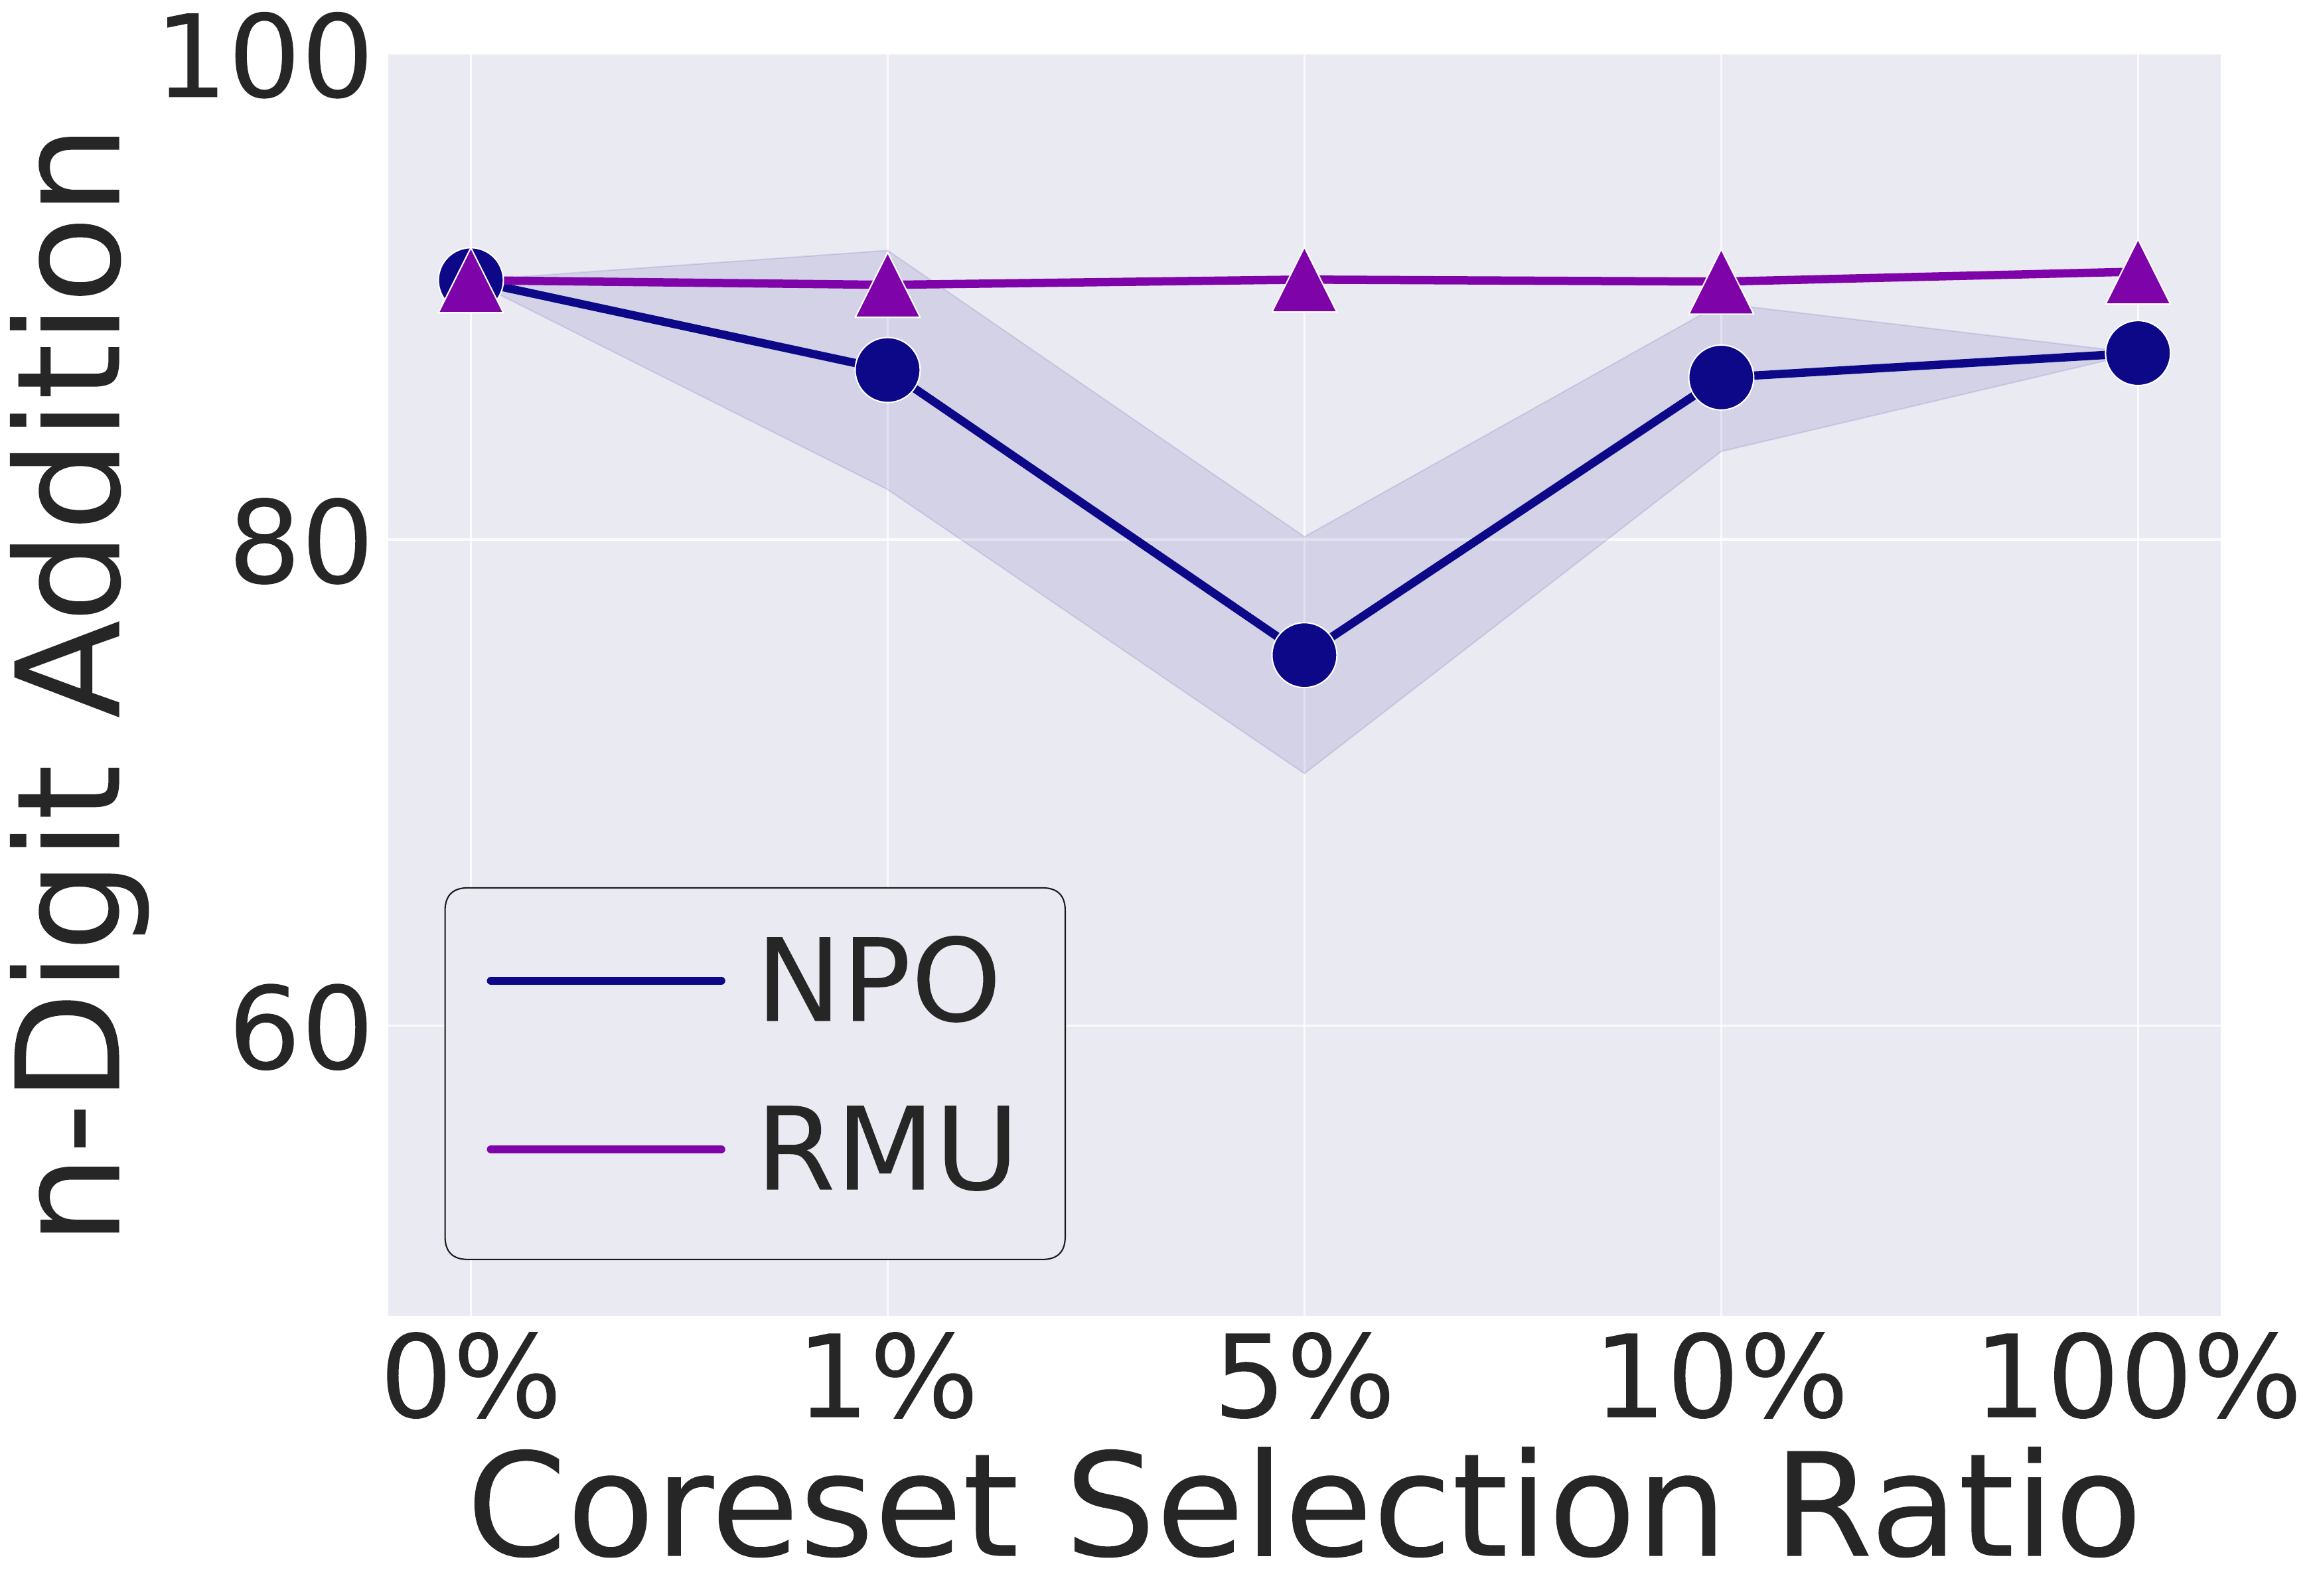}    &  
 \hspace*{-3.9mm}
 \includegraphics[width=.23\textwidth]{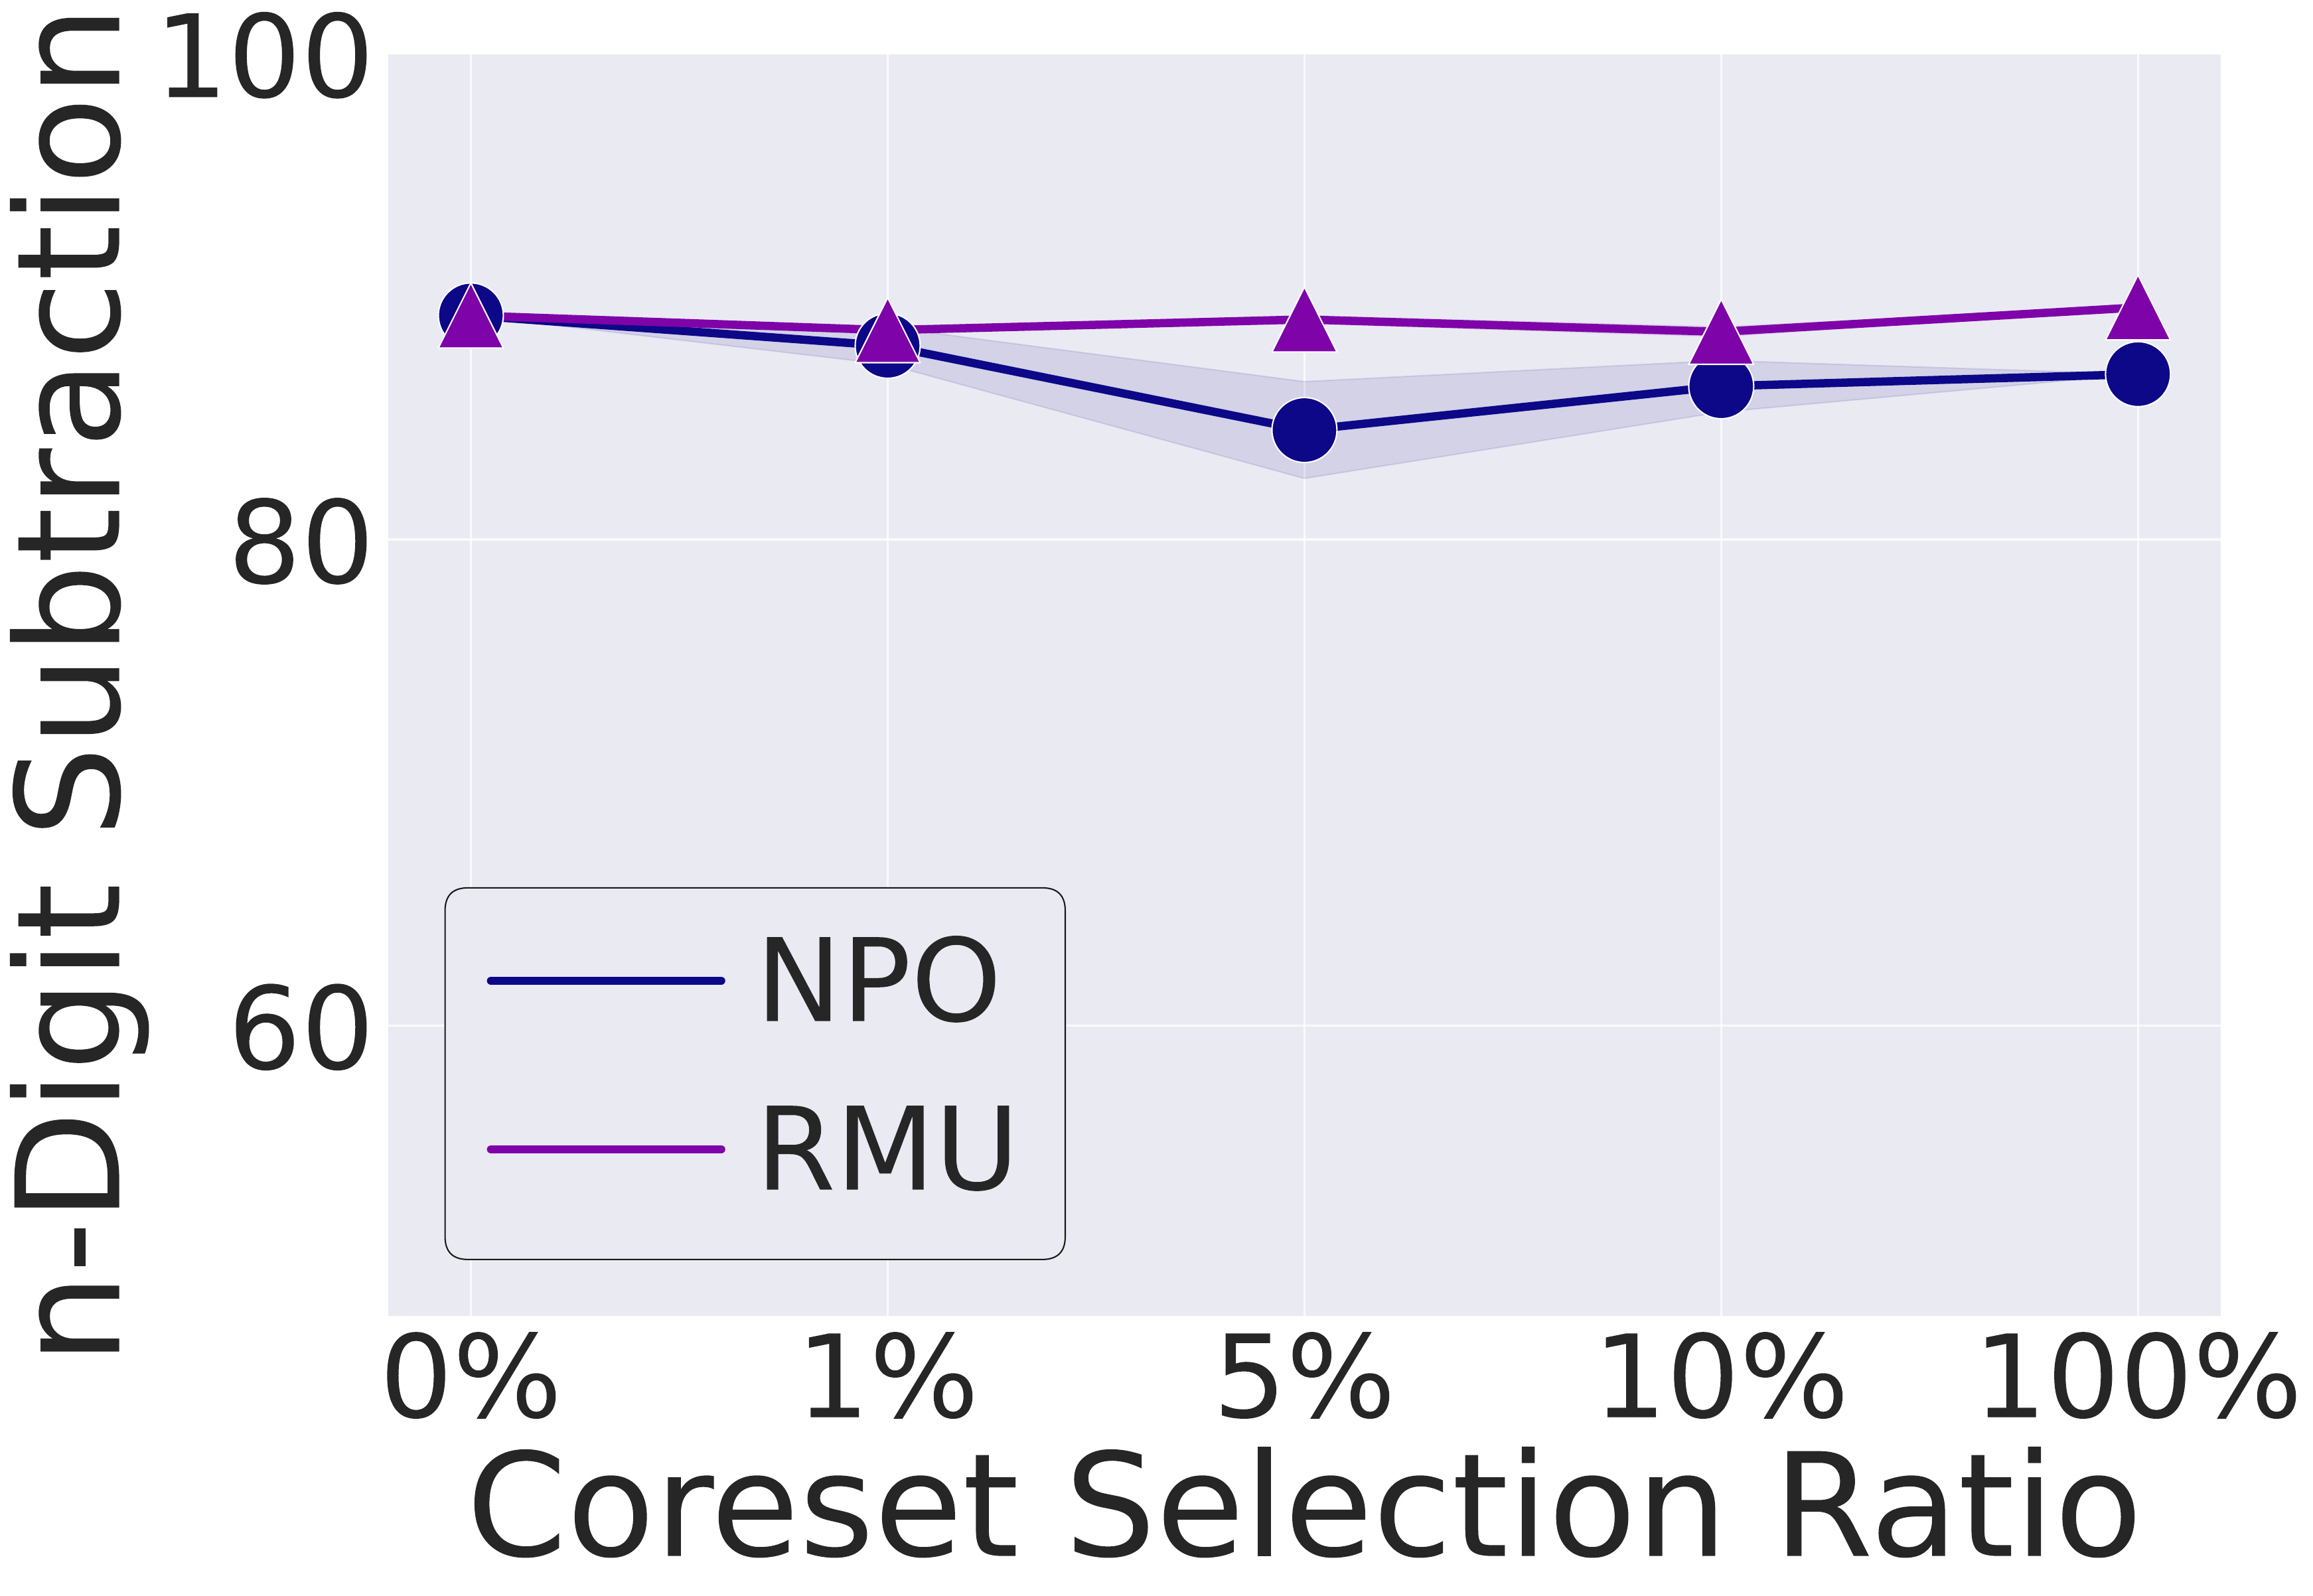} &
 \hspace*{-3.9mm}
 \includegraphics[width=.23\textwidth]{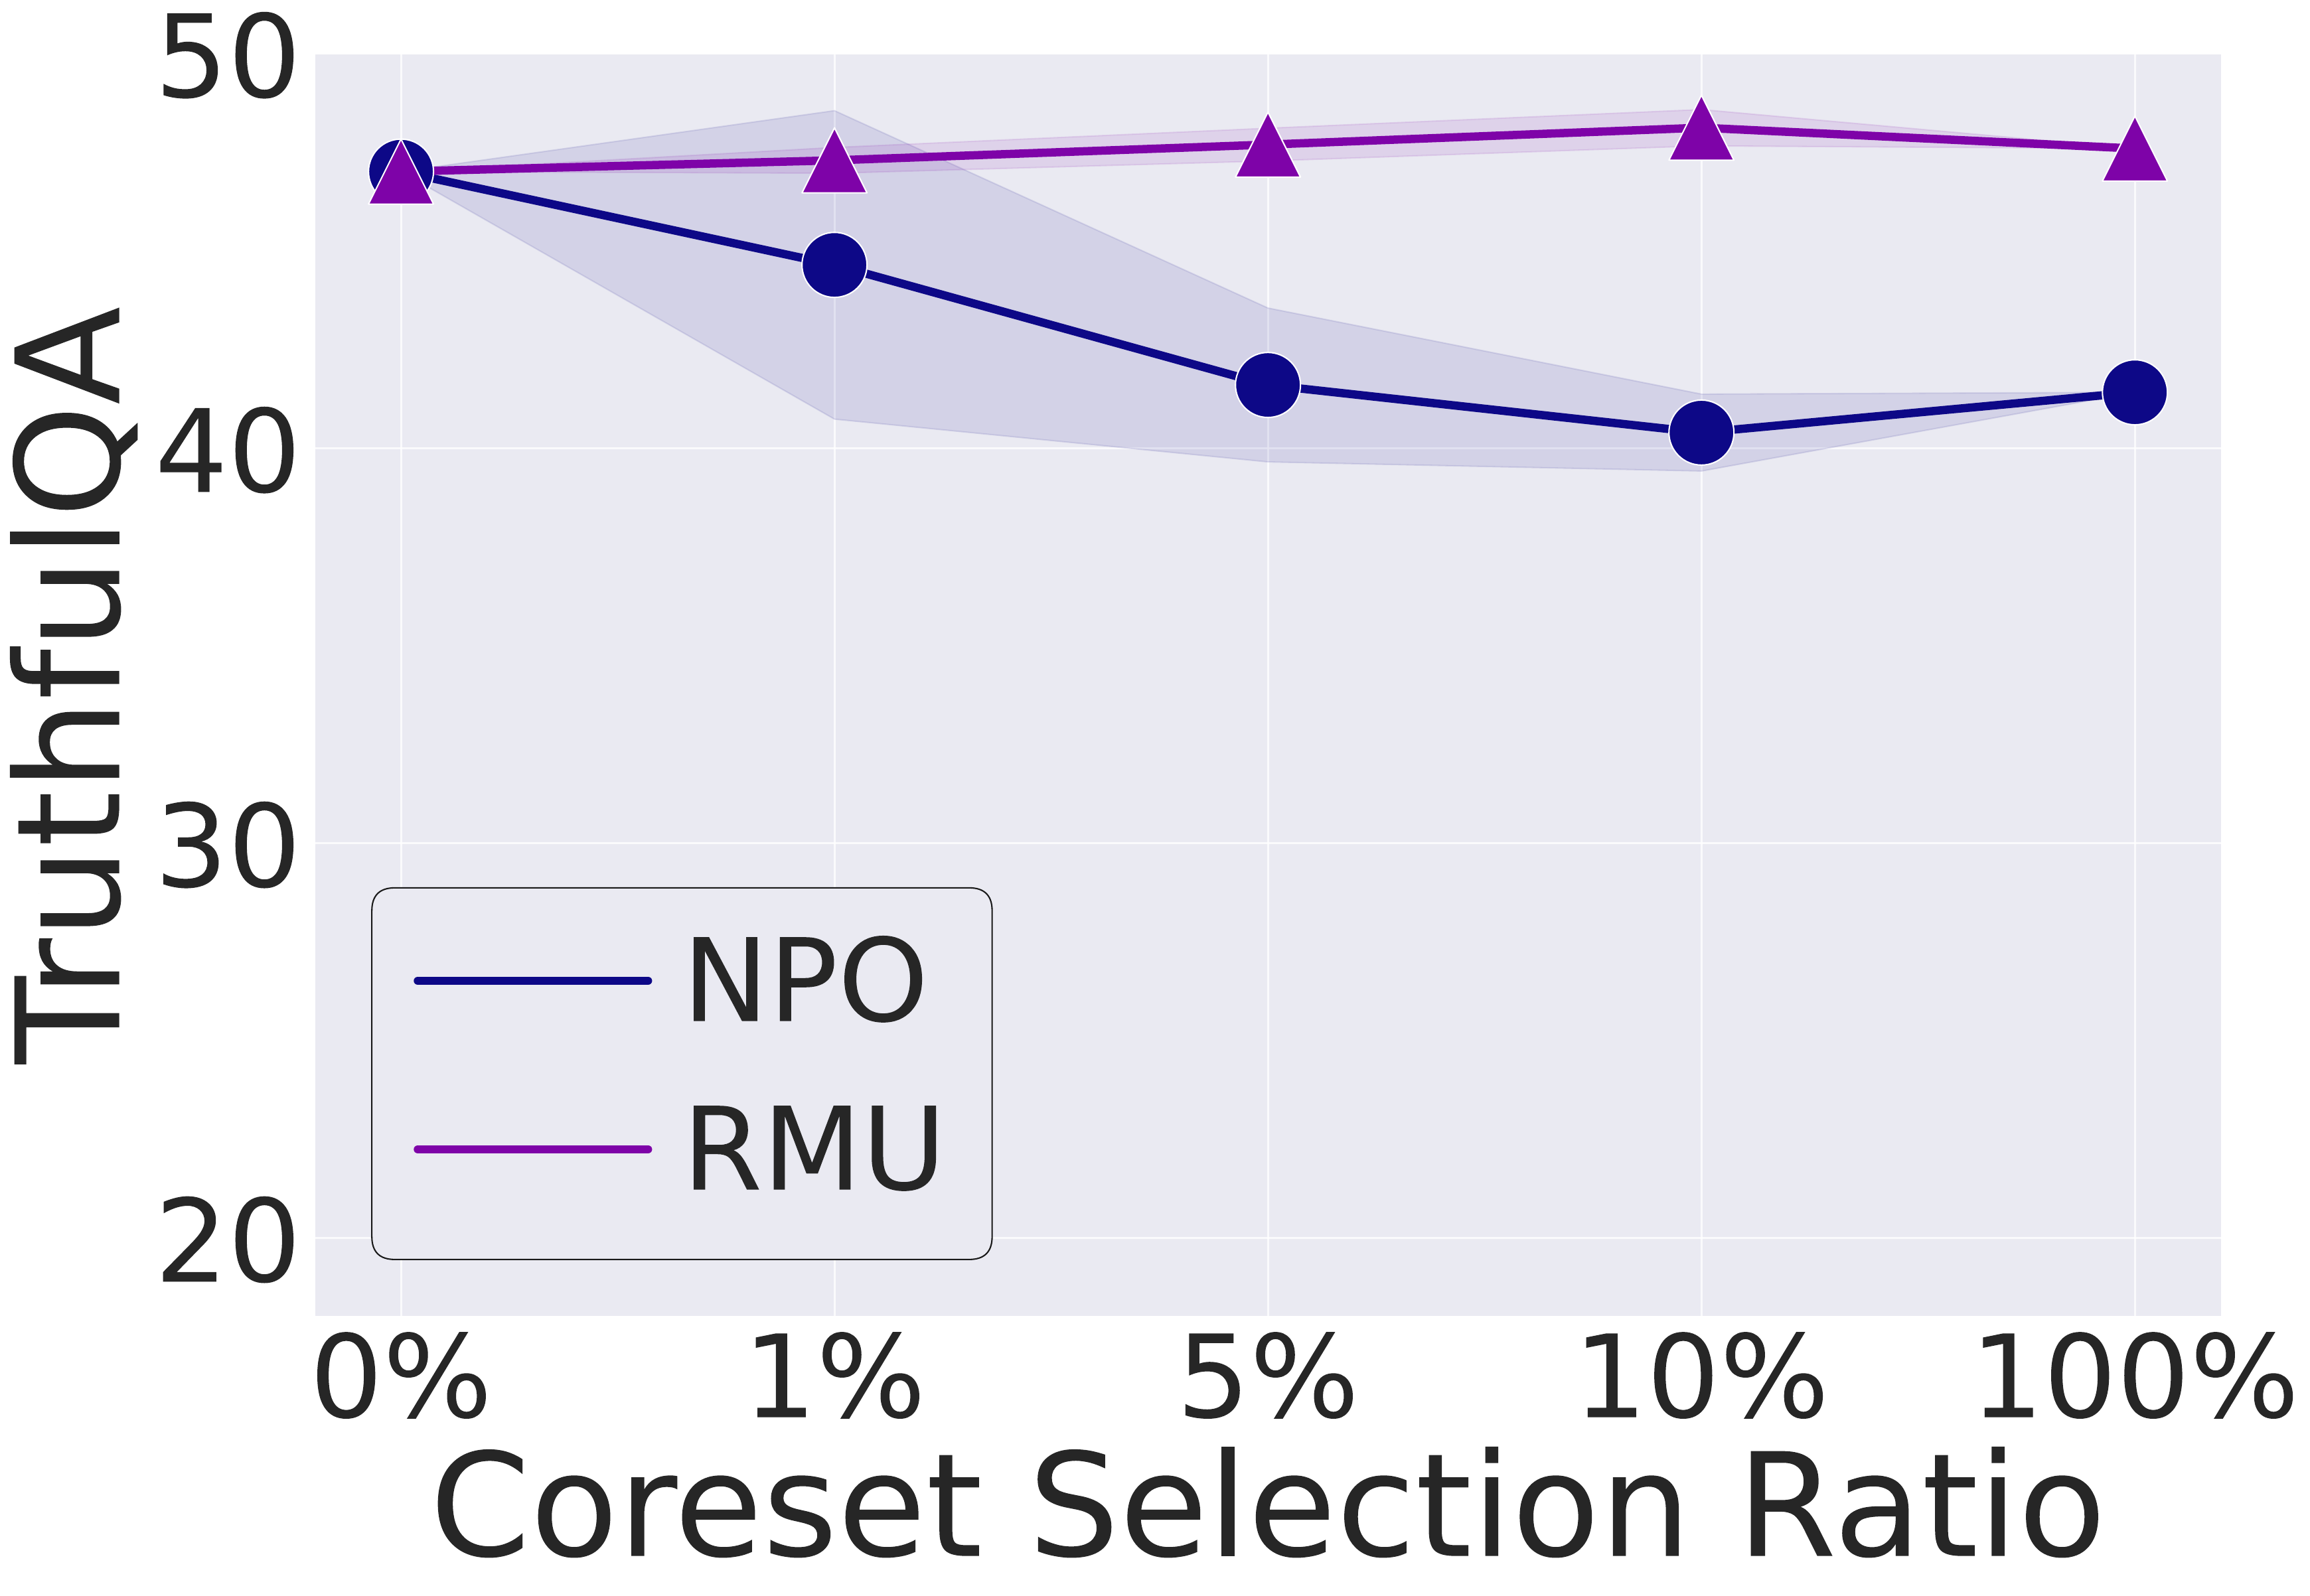}   
 \\
% {\footnotesize{(a) n-Digit Addition, WMDP-Bio}}
% & {\footnotesize{(b) n-Digit Subtraction, WMDP-Bio}}
% & {\footnotesize{(c) Truthful QA, WMDP-Bio}} 
% \\
{\footnotesize{(a) Addition, WMDP-Bio}}
& {\footnotesize{(b) Subtraction, WMDP-Bio}}
& {\footnotesize{(c) TruthfulQA, WMDP-Bio}} 
\\
\includegraphics[width=.23\textwidth]{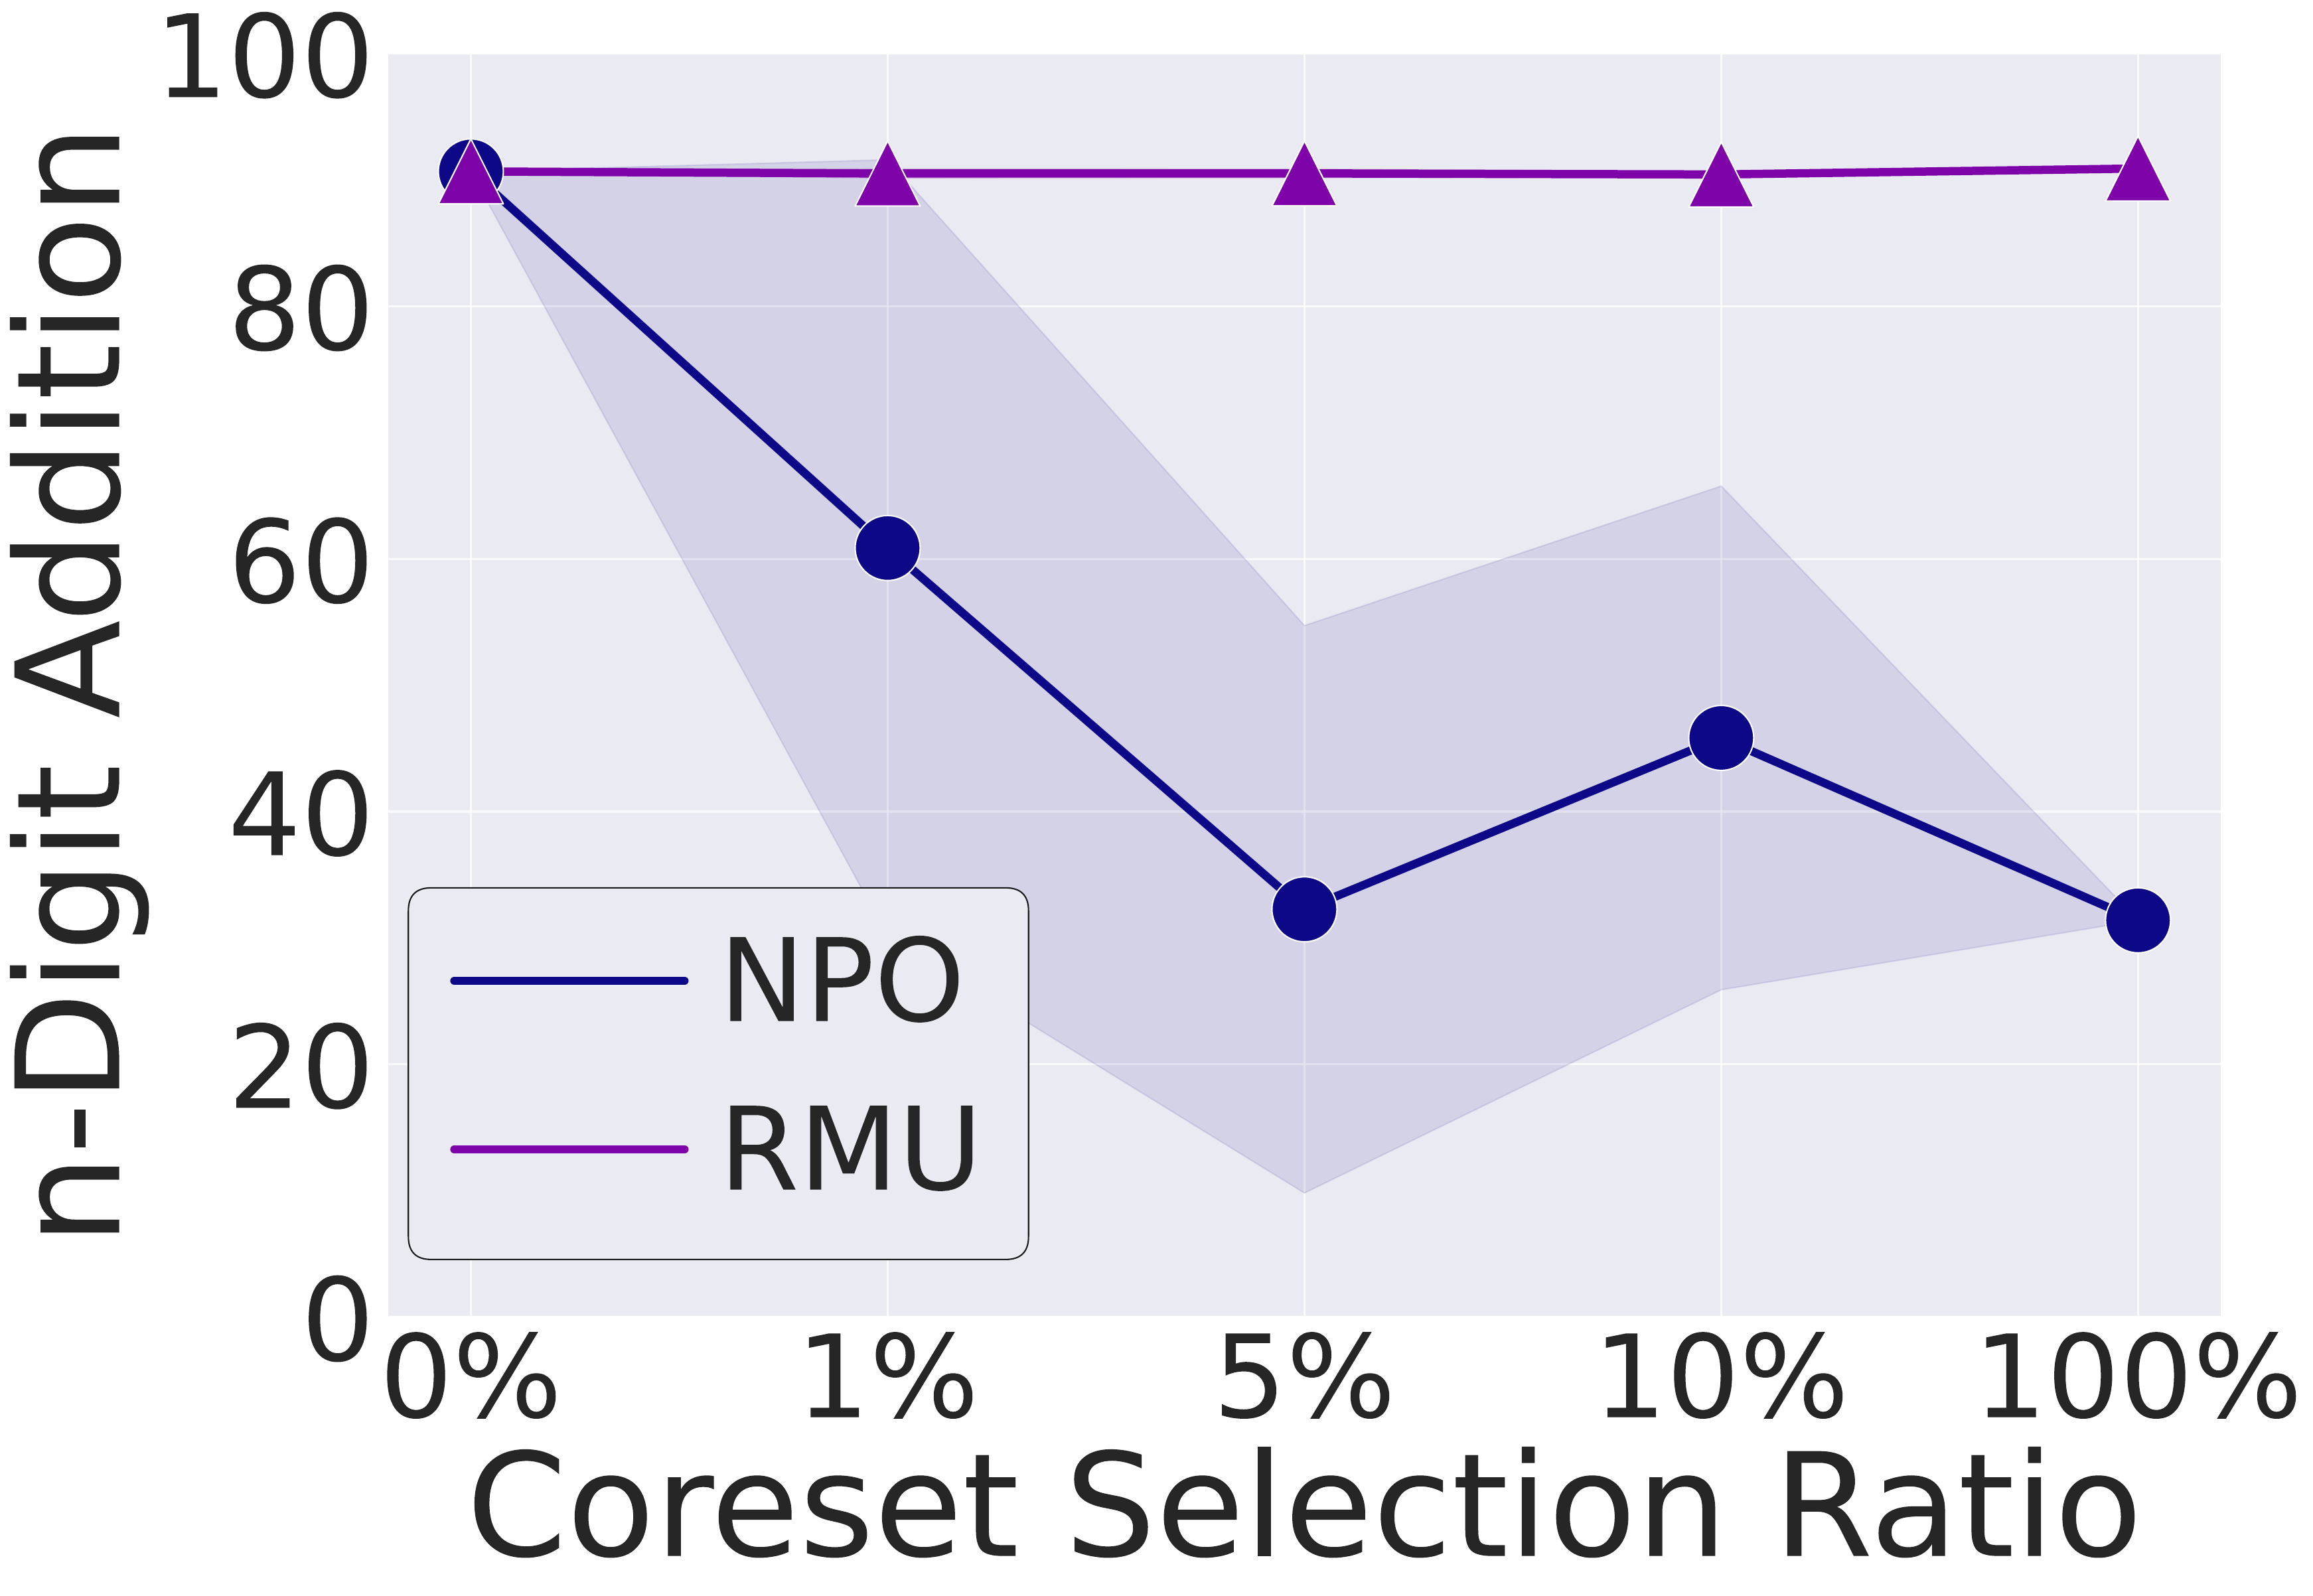}    &  
 \hspace*{-3.9mm}
 \includegraphics[width=.23\textwidth]{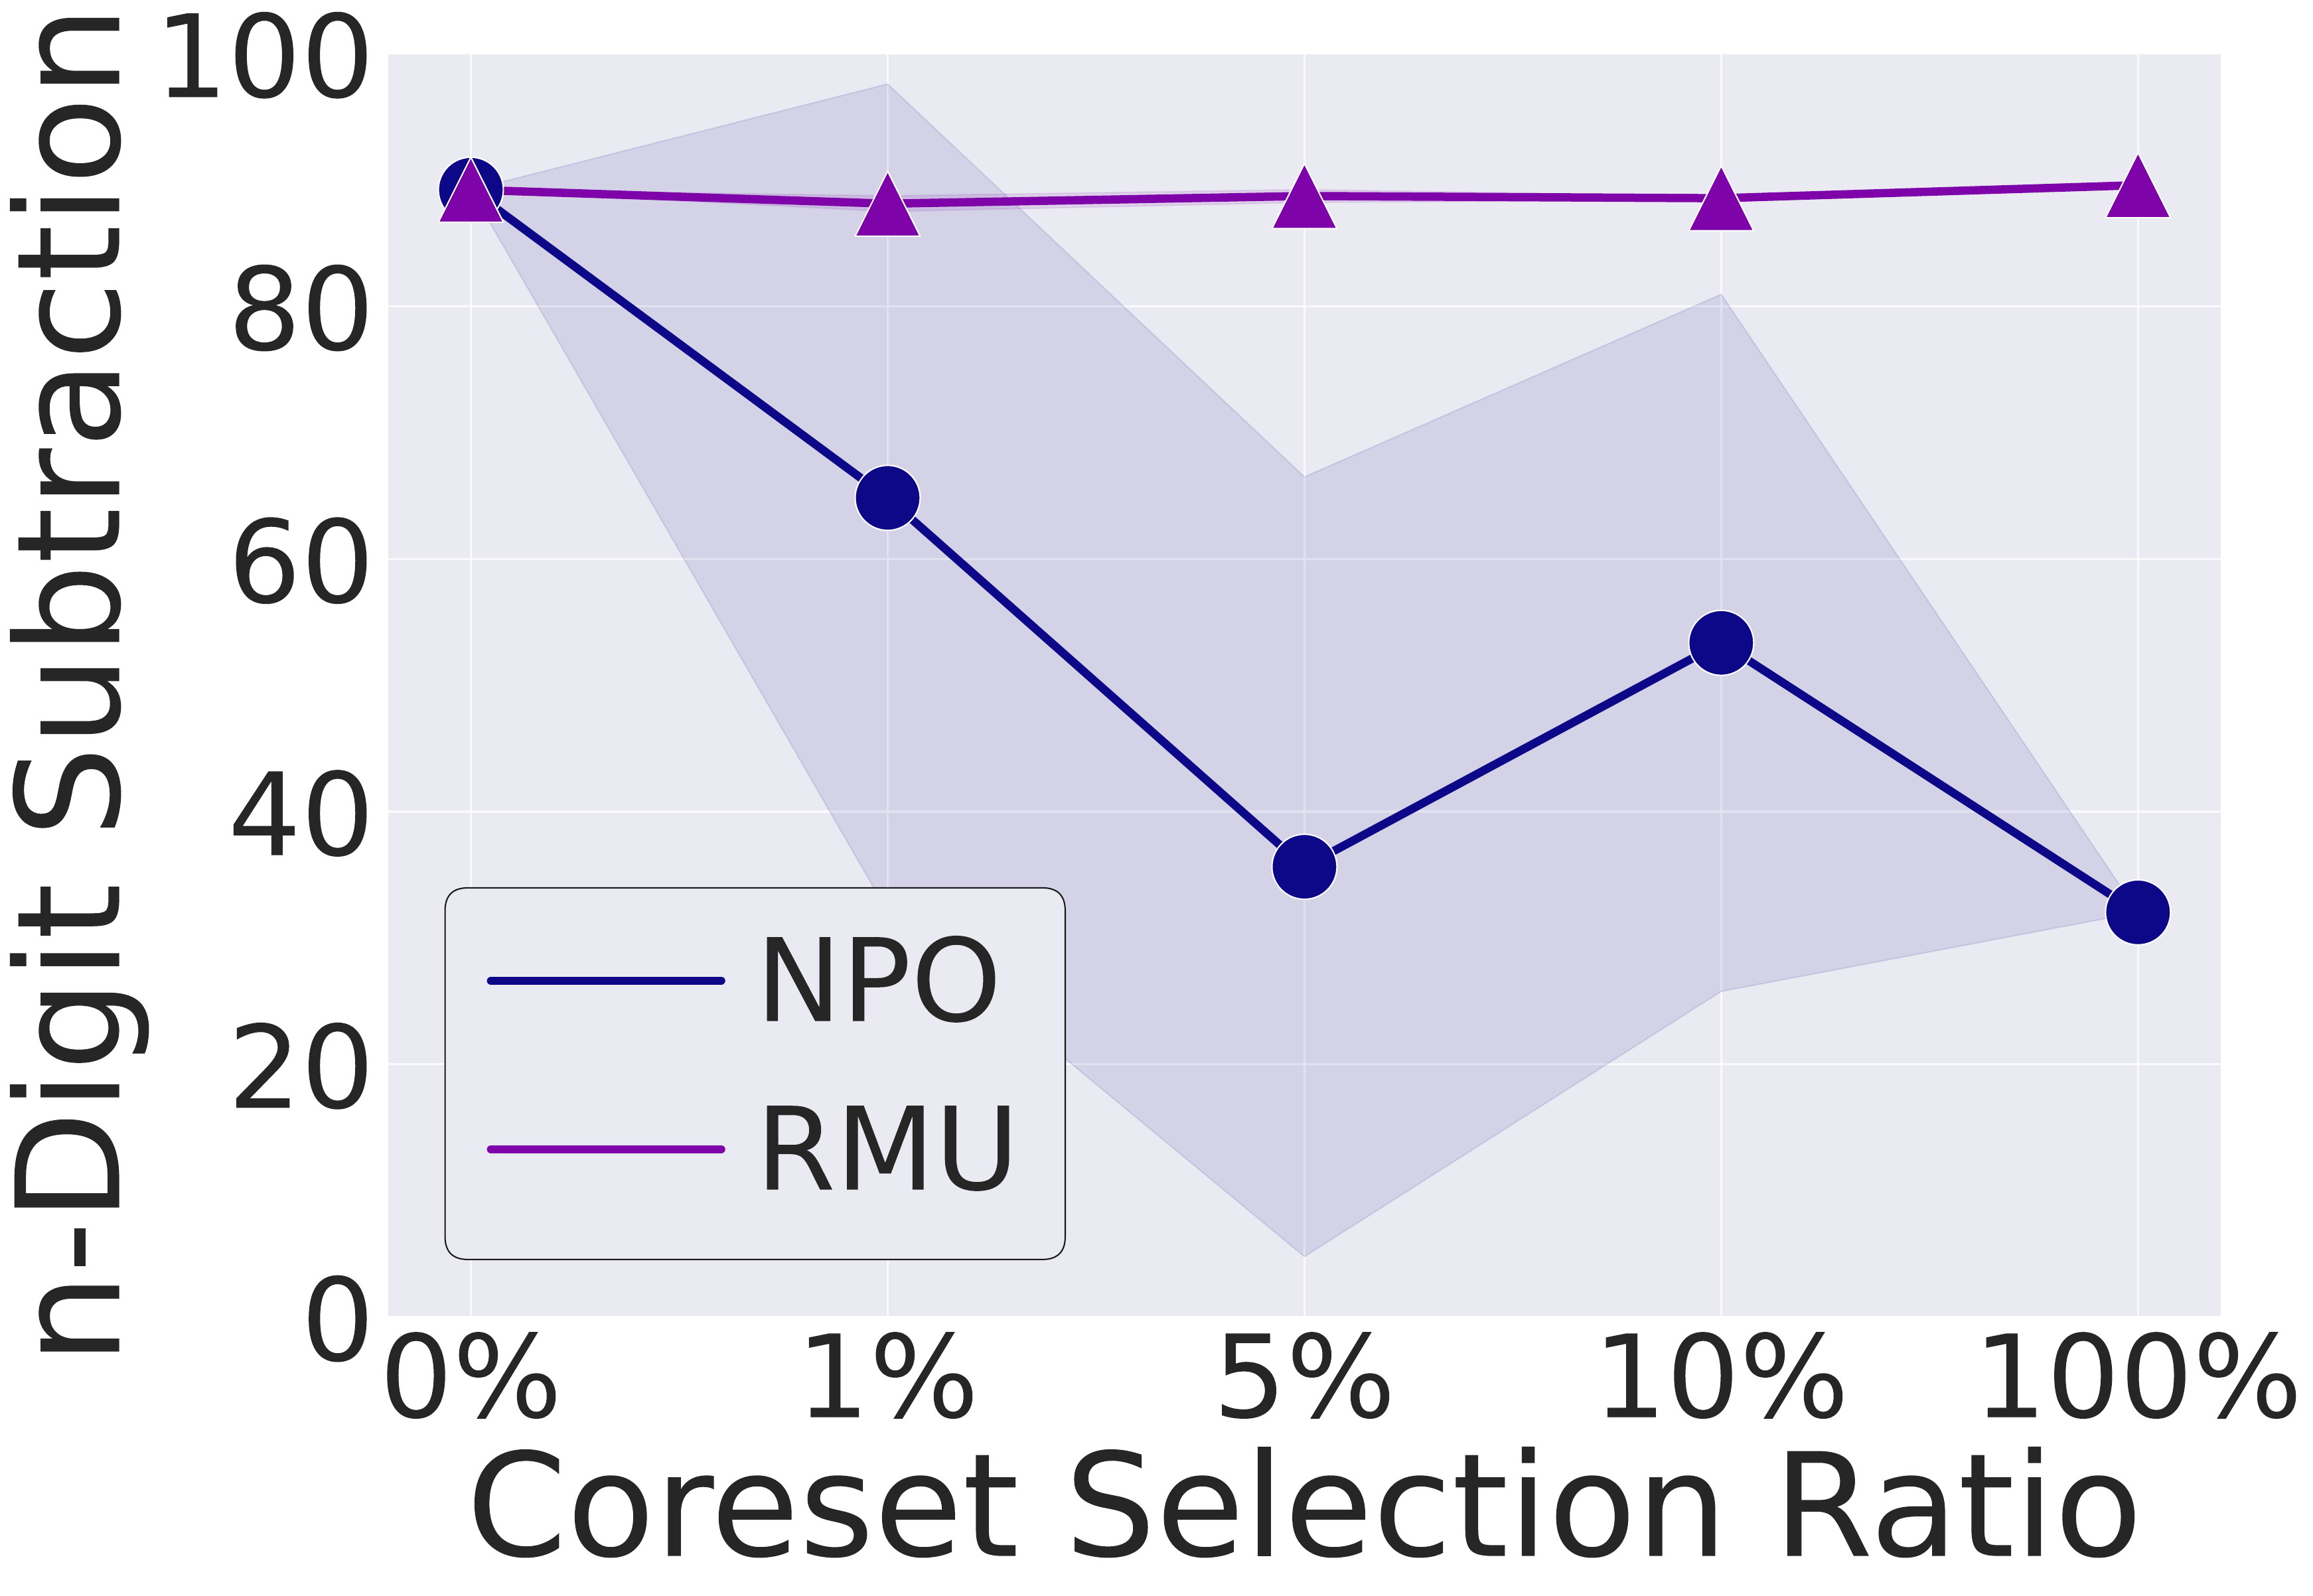} &
 \hspace*{-3.9mm}
 \includegraphics[width=.23\textwidth]{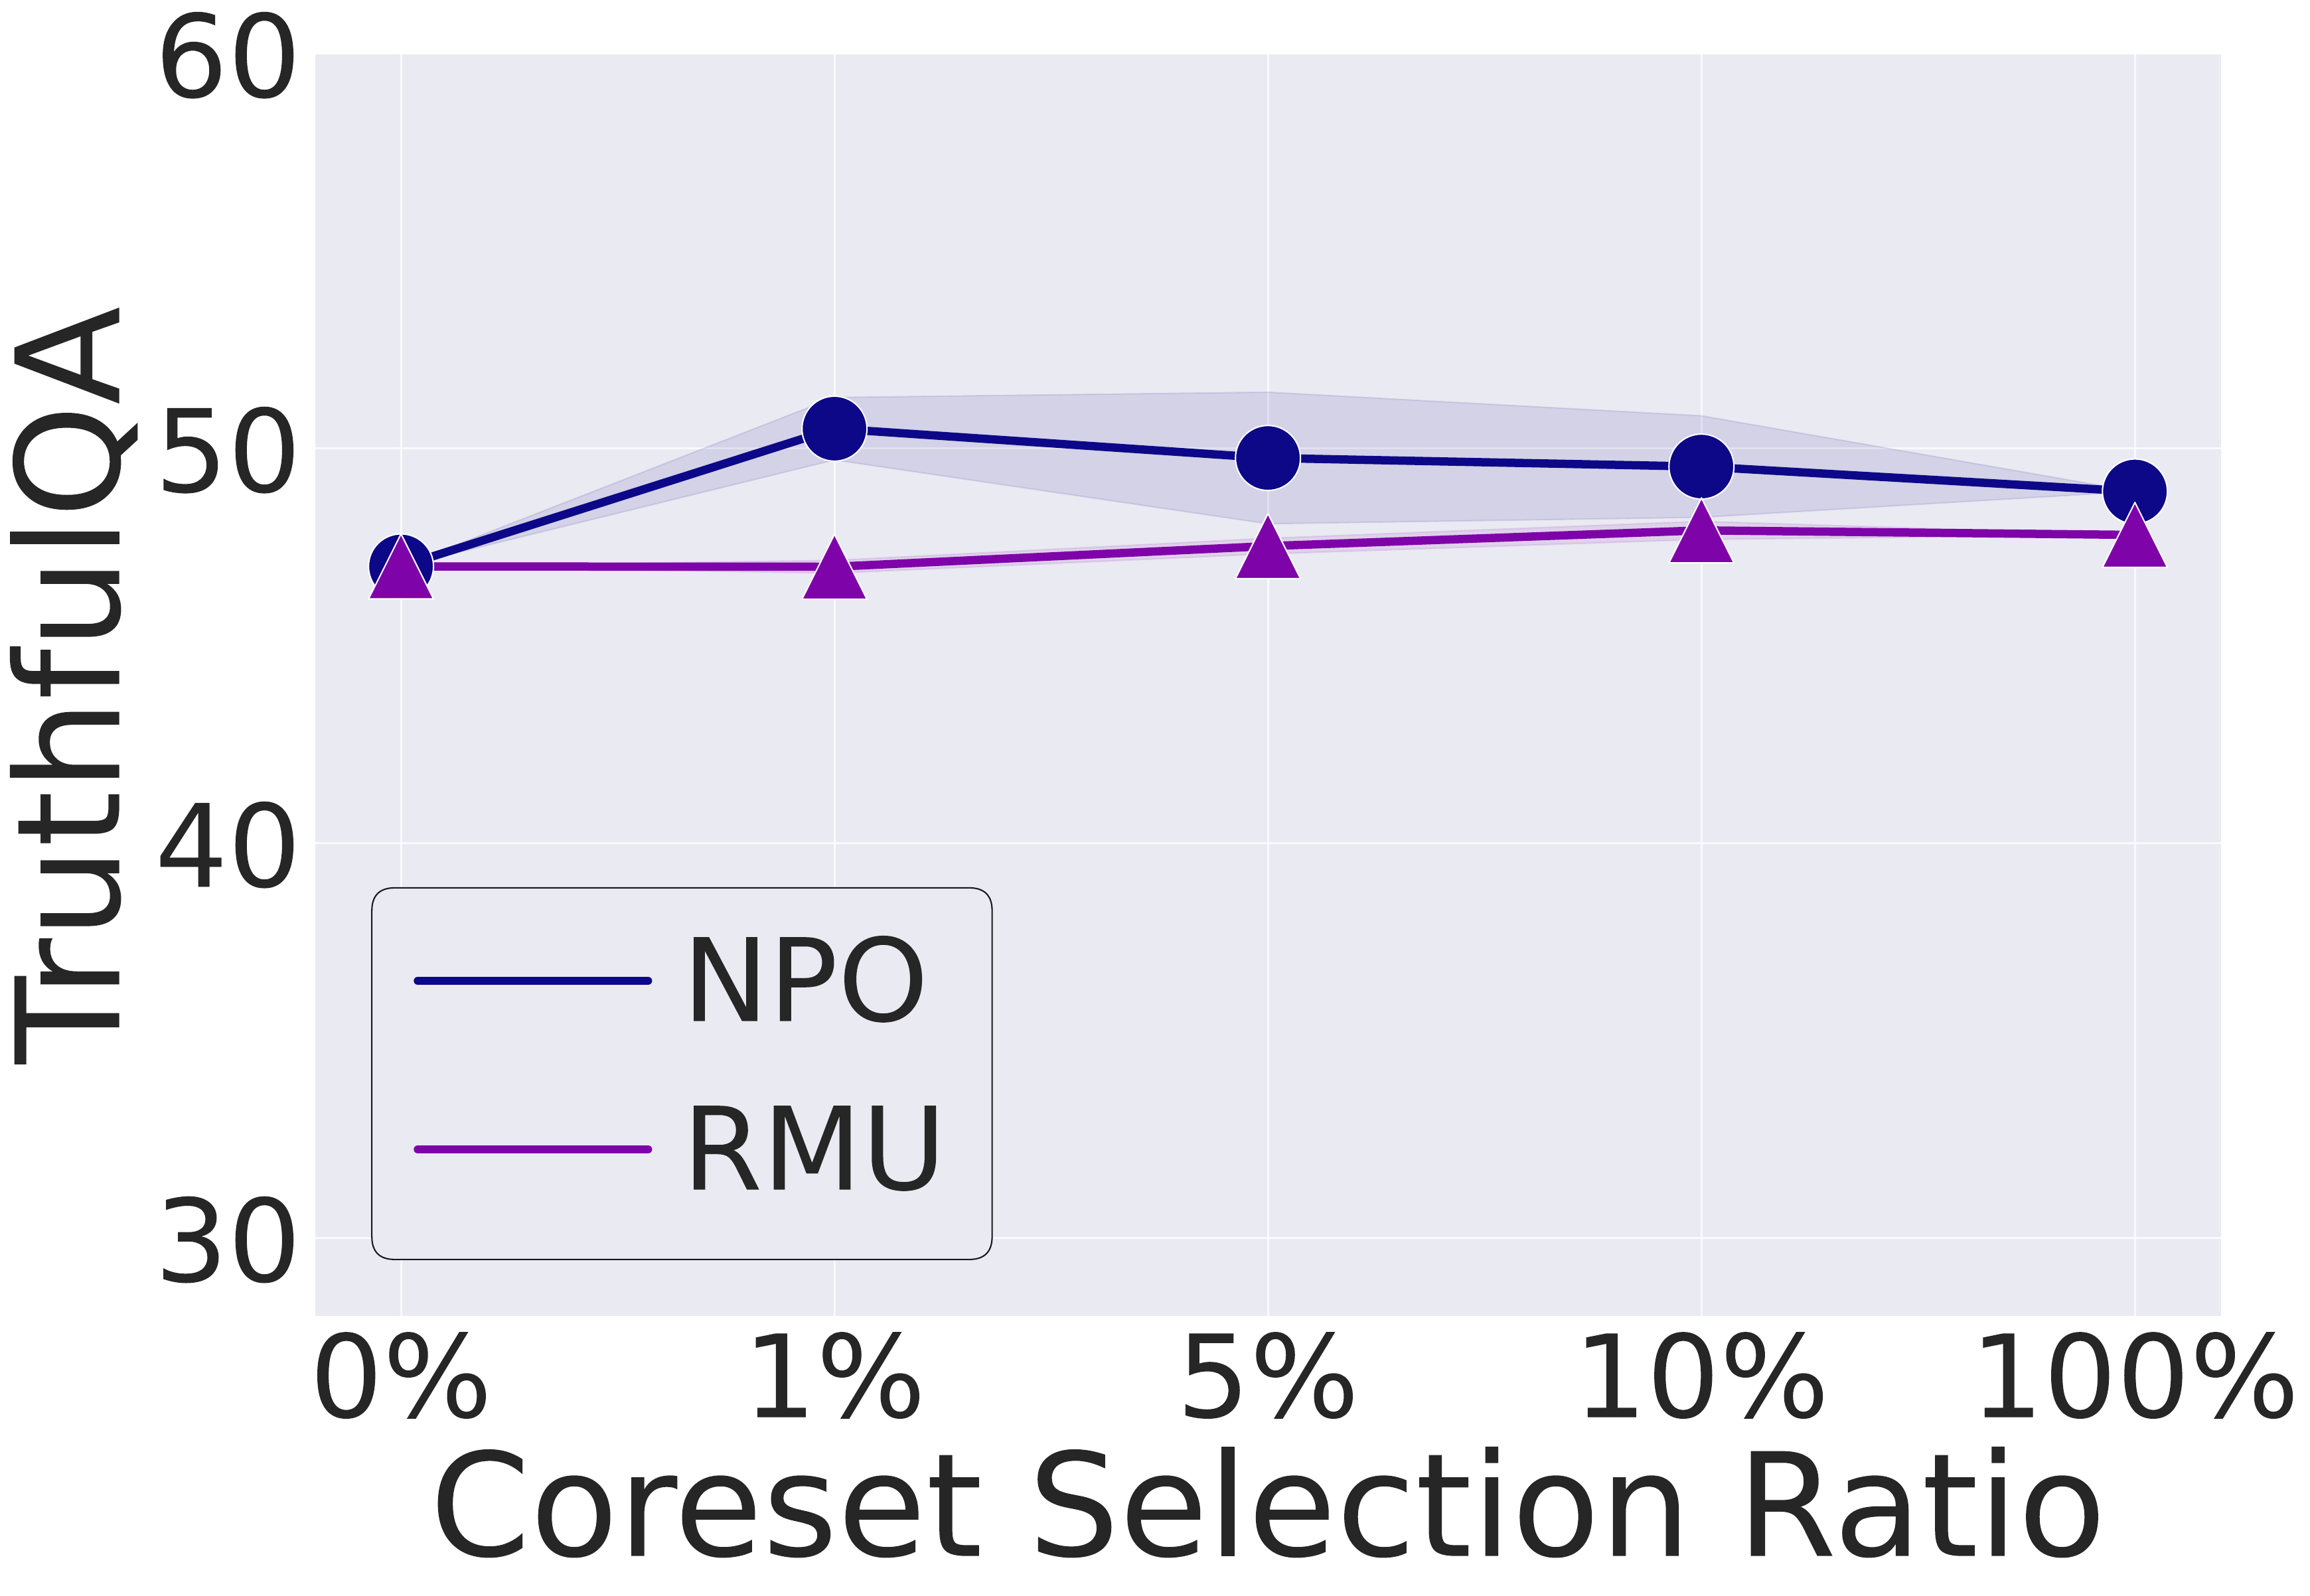} 
  \\
% {\footnotesize{(e) n-Digit Addition, WMDP-Cyber}}
% & {\footnotesize{(f) n-Digit Subtraction, WMDP-Cyber}}
% & {\footnotesize{(g) Truthful QA, WMDP-Cyber}} 
% \\
{\footnotesize{(e) Addition, WMDP-Cyber}}
& {\footnotesize{(f) Subtraction, WMDP-Cyber}}
& {\footnotesize{(g) TruthfulQA, WMDP-Cyber}} 
\\
\end{tabular}
\vspace*{-2mm}
\caption{\small{Additional utility evaluation performance for \random{}-coreset unlearned models using NPO and RMU under  Zephyr-7B-$\beta$. (a)-(d) correspond to the performance of a specific utility evaluation (Addition, Subtraction, Truthful QA) of models unlearned using WMDP-Bio or WMDP-Cyber. Here `Addition' refers to n-digit addition (n=2,3,4,5) and `Subtraction' refers n-digit subtraction (n=2,3,4,5), where the accuracies are averaged over n.
The unlearning task and setting follow the same configuration as  in Fig.\,\ref{fig: random_sufficient}.
}}
  \label{fig: additional utility}
\end{figure}

%\SP{
% In \reffig{fig: additional utility}, we report the zero-shot accuracy of the aforementioned utility metrics for \random{}-based coreset-unlearned models using RMU and NPO on WMDP. RMU consistently maintains strong utility across all evaluations, regardless of the coreset selection ratio. In contrast, NPO shows higher variance; however, we observe that for $n$-digit addition and subtraction, performance may benefit from using a 10\% coreset in the WMDP-Cyber setting.
%At the same time, NPO can degrade utility at 5\% coreset selection ratio. 
%}
% We attribute this to NPO being a divergence-driven method
