# Supplementary material for: LLM Unlearning Reveals a Stronger-Than-Expected Coreset Effect in Current Benchmarks
Source: arXiv:2504.10185 source file (2025-04-16)
Supplement: Supplementary file 2 [file app_coreset_description.tex]

\section{Details of Coreset Selection Methods}
\label{app: coreset_selection}

\makeatother
\setcounter{table}{0}
\setcounter{equation}{0}

In this section, we present additional details of the heuristic data selection methods as presented in Sec.\,\ref{sec: consistency}.
Though these methods were primarily developed for non-LLMs, we adapt them to our unlearning process as detailed below.

\paragraph{\grand{}.} 
The main rationale behind this method \citep{paul2021deep} is that the importance of each sample $z_f$ from the forget set is captured by the expected gradient norm of the loss associated with that sample, where the expectation is taken over the unlearning trajectory. Thus the \grand{} score is given by:
\begin{align}
\begin{array}{l}
  \chi(z_f) =  \mathbb E_{\btheta_t} \| \nabla_{\btheta_t} [\lf(z_f; \btheta_t) + \lambda \lr( z_r; \btheta_t) ] \|_2 \ ; \ \text{where} \ z_f \sim \Df, ~~z_r \sim \Dr
\end{array}
\label{eq:grand}
\end{align}
Here $\lf$ and $\lr$ are specified in \eqref{eq: LLM_MU}, where $\lf$ changes according to the unlearning method as specified before. In our experiments, we consider the trajectory of unlearning for 10 epochs for the purpose of computing the above expectation.
% \SP{I will check if their theorems hold here. I will check and update the above later. But if anyone has time, kindly check.}

\paragraph{Moderate.}   
The moderate coreset selection method \citep{xia2022moderate} was developed in the classification setting where samples were divided into clusters according to their classes. Using a well-trained model, the class center of each class is calculated using the hidden state representations of the penultimate layer of the corresponding samples.
Since our setting does not involve class labels, we cluster the forget samples into four groups using K-means, based on their penultimate-layer representations extracted from the reference (pre-unlearned) model. For each cluster, we compute its centroid and rank the samples by their distance to the respective centroid. To select representative data points, we choose those whose distances are closest to the median within their cluster.

\paragraph{\mink{}.}
The \mink{} method \citep{shi2024detecting} was developed to ascertain whether a given text appears in the original pretraining dataset. We use this metric as a data selection method for unlearning under the notion that data points not encountered during training are less influential in the unlearning process. In fact, in  \citep{shi2024detecting}, the authors demonstrated that the \textsc{Min-K\%} metric can be used as an effective indicator for assessing removal of knowledge after unlearning. 

For a given datapoint $z$, we calculate the log-likelihood of each token and choose a set of top $40\% (\text{K} = 40)$ of tokens with lowest value, called $\text{Min-K\%}(z)$. Then the score for $z$ is calculated as:
\begin{align}
\begin{array}{l}
  \mink{}(z) = \frac{1}{|\text{Min-K\%}(z)|} \sum_{z_i \in \text{Min-K\%}(z)}{ \log p(z_i | z_1, ..., z_{i-1}; \btheta)}
\end{array}
\label{eq:mink}
\end{align}

After computing the above scores for each sample $z$ in $\Df$, we choose samples with the top $\mathrm{p}$ scores to obtain our coresets. 
Thus, if we want to choose a 5\% coreset, then $\mathrm{p} = 0.05\times|\Df|$.
