# Supplementary material for: LLM Unlearning Reveals a Stronger-Than-Expected Coreset Effect in Current Benchmarks
Source: arXiv:2504.10185 source file (2025-04-16)
Supplement: Supplementary file 3 [file app_epochs.tex]

\section{Detailed Unlearning Setup}
\label{app: epochs}

% \setcounter{section}{0}
% \setcounter{figure}{0}
% \makeatletter 

\makeatother
\setcounter{table}{0}
\setcounter{equation}{0}

% Note that this does not use the full forget set and thus
We present the detailed unlearning setups for different settings in \reftab{tab: app_setting}.
It is worth noting that 
the first 600 samples of WMDP-Bio and WMDP-Cyber are used as the \textit{full} forget set following \citep{li2024wmdp}. 
% We perform unlearning for NPO and RMU over these 600 samples with a batch size of 4, consistent with the original setting. 
For NPO, we perform unlearning for 140 steps with a batch size of 4, which is approximately $(140 \times 4 )/600 = 0.93$ epochs.

\begin{table}[htb]
\begin{center}
%\vspace{-2mm}
\caption{\small{Full forget set unlearning settings across different unlearning methods and benchmarks. 
% \SL{[talk to me on coreset setting.]}
%Here WMDP refers to both WMDP-Bio and WMDP-Cyber.
}}
\vspace{2mm}
\label{tab: app_setting}
\resizebox{0.6\textwidth}{!}{
\begin{tabular}{c|c|c|c|c}

\toprule[1pt]
% \midrule

\multicolumn{1}{c|}{\multirow{2}{*}{
\begin{tabular}{c}
   \textbf{Unlearning}
   \\
    \textbf{Benchmark} 
\end{tabular}
}} 
& 
\multicolumn{1}{c|}{\multirow{2}{*}{
\begin{tabular}{c}
   \textbf{Unlearning} \\
     \textbf{Method} 
\end{tabular}
}} 
& 
\multicolumn{1}{c|}{\multirow{2}{*}{
\begin{tabular}{c}
   \textbf{Model} 
\end{tabular}
}}
& 
\multicolumn{1}{c}{\multirow{2}{*}{
\begin{tabular}{c}
   \textbf{Epochs} 
\end{tabular}
}} 
& 
\multicolumn{1}{c}{\multirow{2}{*}{
\begin{tabular}{c}
      \textbf{Learning} \\
     \textbf{Rate} 
\end{tabular}
}}
\\
&&&\\
\midrule
\multicolumn{1}{c|}{\multirow{2}{*}{
\begin{tabular}{c}
  WMDP-Bio/Cyber
\end{tabular}
}} 
& 
RMU
&
\multicolumn{1}{c|}{\multirow{2}{*}{
\begin{tabular}{c}
   Zephyr-7B-$\beta$
\end{tabular}
}}
&
1
&
$5e-5$
\\
& 
NPO
&
&
0.93
&
$7e-6$
\\
\midrule
\multicolumn{1}{c|}{\multirow{2}{*}{
\begin{tabular}{c}
   MUSE-Books
\end{tabular}
}}
&
RMU
&
\multicolumn{1}{c|}{\multirow{2}{*}{
\begin{tabular}{c}
ICLM-7B
\end{tabular}
}}
&
\multicolumn{1}{c|}{\multirow{2}{*}{
\begin{tabular}{c}
1
\end{tabular}
}}
&
$1e-3$
\\
& 
NPO
&
&
&
$1e-5$

\\
\midrule
\multicolumn{1}{c|}{\multirow{2}{*}{
\begin{tabular}{c}
   MUSE-News 
\end{tabular}
}}
&
RMU
&
\multicolumn{1}{c|}{\multirow{2}{*}{
\begin{tabular}{c}
   LLaMA2-7B
\end{tabular}
}}
&
\multicolumn{1}{c}{\multirow{2}{*}{
\begin{tabular}{c}
10
\end{tabular}
}}
&

$1e-3$

\\
& 
NPO
&
&
&
$1e-5$
\\
% \midrule
\bottomrule[1pt]
\end{tabular}
}
% \vspace*{2mm}
\end{center}
\end{table}

Unless otherwise mentioned, we follow the standard hyperparameters in the above benchmarks. For MUSE-Books \citep{shi2024muse}, the reference model ICLM-7B is finetuned on Harry Potter books, while for MUSE-News, the reference model LLaMA2-7B is finetuned on BBC News articles. These reference models are available in the MUSE benchmark.  

 As mentioned in Sec.\,\ref{sec: problemstmnt}, the coreset effect emerges with a higher number of unlearning epochs. In \reftab{tab: app_setting_coreset}, we present the epoch numbers for each coreset setting. All other unlearning settings are the same as the full forget set unlearning.

\begin{table}[htb]
\begin{center}
%\vspace{-2mm}
\caption{\small{Coreset unlearning settings across different unlearning methods and benchmarks. 
% \SL{[talk to me on coreset setting.]}
%Here WMDP refers to both WMDP-Bio and WMDP-Cyber.
}}
\vspace{2mm}
\label{tab: app_setting_coreset}
\resizebox{0.6\textwidth}{!}{
\begin{tabular}{c|c|c|c}

\toprule[1pt]
% \midrule

\multicolumn{1}{c|}{\multirow{2}{*}{
\begin{tabular}{c}
   \textbf{Unlearning}
   \\
    \textbf{Benchmark} 
\end{tabular}
}} 
& 
\multicolumn{1}{c|}{\multirow{2}{*}{
\begin{tabular}{c}
   \textbf{Unlearning} \\
     \textbf{Method} 
\end{tabular}
}} 
& 
\multicolumn{1}{c|}{\multirow{2}{*}{
\begin{tabular}{c}
   \textbf{Coreset} \\
     \textbf{Ratio} 
\end{tabular}
}}
& 
\multicolumn{1}{c}{\multirow{2}{*}{
\begin{tabular}{c}
   \textbf{Epochs} 
\end{tabular}
}} 
% & 
% \multicolumn{1}{c}{\multirow{2}{*}{
% \begin{tabular}{c}
%       \textbf{Learning} \\
%      \textbf{Rate} 
% \end{tabular}
% }}
\\
&&&\\
\midrule
\multicolumn{1}{c|}{\multirow{3}{*}{
\begin{tabular}{c}
  WMDP-Bio/Cyber
\end{tabular}
}} 
& 
\multicolumn{1}{c|}{\multirow{3}{*}{
\begin{tabular}{c}
  RMU
\end{tabular}
}} 
&
10\%
&
10
% &
% $5e-5$
\\
& 
&
5\%
&
20
% &
% $7e-6$
\\
&&
1\%
&
100
\\
\midrule

\multicolumn{1}{c|}{\multirow{3}{*}{
\begin{tabular}{c}
  WMDP-Bio/Cyber
\end{tabular}
}} 
& 
\multicolumn{1}{c|}{\multirow{3}{*}{
\begin{tabular}{c}
  NPO
\end{tabular}
}} 
&
10\%
&
9.33
% &
% $5e-5$
\\
& 
&
5\%
&
18.67
% &
% $7e-6$
\\
&&
1\%
&
93.33
\\
\midrule

\multicolumn{1}{c|}{\multirow{2}{*}{
\begin{tabular}{c}
   MUSE-Books
\end{tabular}
}}
&
\multicolumn{1}{c|}{\multirow{2}{*}{
\begin{tabular}{c}
   RMU
\end{tabular}
}}
&
10\%
&
10
% &
% $1e-3$
\\
& 
&
5\%
&
20
\\
\midrule

\multicolumn{1}{c|}{\multirow{2}{*}{
\begin{tabular}{c}
   MUSE-Books
\end{tabular}
}}
&
\multicolumn{1}{c|}{\multirow{2}{*}{
\begin{tabular}{c}
   NPO
\end{tabular}
}}
&
10\%
&
7
% &
% $1e-3$
\\
& 
&
5\%
&
8
\\
\midrule

\multicolumn{1}{c|}{\multirow{2}{*}{
\begin{tabular}{c}
   MUSE-News
\end{tabular}
}}
&
\multicolumn{1}{c|}{\multirow{2}{*}{
\begin{tabular}{c}
   RMU
\end{tabular}
}}
&
10\%
&
100
% &
% $1e-3$
\\
& 
&
5\%
&
200
\\
\midrule

\multicolumn{1}{c|}{\multirow{2}{*}{
\begin{tabular}{c}
   MUSE-News
\end{tabular}
}}
&
\multicolumn{1}{c|}{\multirow{2}{*}{
\begin{tabular}{c}
   NPO
\end{tabular}
}}
&
10\%
&
5
% &
% $1e-3$
\\
& 
&
5\%
&
12
\\
% \midrule
\bottomrule[1pt]
\end{tabular}
}
% \vspace*{2mm}
\end{center}
\end{table}
