# Supplementary material for: LLM Unlearning Reveals a Stronger-Than-Expected Coreset Effect in Current Benchmarks
Source: arXiv:2504.10185 source file (2025-04-16)
Supplement: Supplementary file 4 [file app_keywordeval.tex]

\section{Queries depicting keywords through definitional Failure}
\label{app: keyword_eval}

\input{Tables/keyword_eval_appendix}
