# Supplementary material for: LLM Unlearning Reveals a Stronger-Than-Expected Coreset Effect in Current Benchmarks
Source: arXiv:2504.10185 source file (2025-04-16)
Supplement: Supplementary file 5 [file app_muse_table.tex]

\section{Coreset Unlearning Performance on MUSE}
\label{app: muse_consistent}
\vspace*{-24mm}

\reftab{tab: muse} presents the coreset unlearning performance ofor MUSE across different coreset selection methods. Here we observe that performance of \random{}-based coresets are highly comparable to the full forget set performance, while also strongly outperforming the full forget set in many instances. 
For example, we observe a significant utility (UT) improvement for MUSE-Books using RMU for coresets as seen in Table \ref{tab: muse}, col.6. In fact, for \moderate-based 10\% coreset we see $\sim 12\%$ improvement in utility over the full forget set.

Additionally, we observe that for MUSE-News, the heuristic based 5\% coreset selection methods have UE (Knowmem) similar to that of the full forget set (as evidenced by Table \ref{tab: muse}, col.3). However, this is worse than the average performance of \random{}-based selection. This coupled with the high variance of the performance \random{}-based coresets points us to the fact that coreset selection is a non-trivial problem for such cases.
Nevertheless, the performance of \random{}-based coreset supports our strong coreset observation even at 5\% coreset selection regime.

\makeatother
\setcounter{table}{0}
\setcounter{equation}{0}

\begin{table}[htb]
\begin{center}
% \vspace{-2mm}
\caption{\small{Coreset-based unlearning performance (UE and UT, consistent with Fig. 2) using RMU and NPO on MUSE evaluated using LLaMA2-7B on News and ICLM-7B on Books. The table is presented in the same format as \reftab{tab: wmdp-bio}. Here `Retrain' refers to a model finetuned only on MUSE excluding the forget set.
} 
}
\vspace*{2mm}
\resizebox{\textwidth}{!}{
\begin{tabular}{c|c|ccc|c|ccc|c}
\toprule[1pt]
\midrule

\multicolumn{1}{c|}{\multirow{4.5}{*}{
\begin{tabular}{c}
   \textbf{Coreset} \\
     \textbf{Ratio}
\end{tabular}
}} 
&\multicolumn{1}{c|}{\multirow{4.5}{*}{
\begin{tabular}{c}
     \textbf{Unlearning} \\
     \textbf{Method}
\end{tabular}
}} 
& \multicolumn{4}{c|}{\textbf{RMU}} 
&  \multicolumn{4}{c}{\textbf{NPO}} \\
\cmidrule{3-10}
&& \multicolumn{3}{c|}{\textbf{UE}} 
& \multicolumn{1}{c|}{\textbf{UT}} 
& \multicolumn{3}{c|}{\textbf{UE}} 
& \multicolumn{1}{c}{\textbf{UT}} \\
\cmidrule{3-10}
&& \begin{tabular}{c}
   \textbf{VerbMem} \\
      ($\downarrow$) 
\end{tabular}
& \begin{tabular}{c}
   \textbf{KnowMem} \\
      ($\downarrow$) 
\end{tabular}
& \begin{tabular}{c}
   \textbf{PrivLeak} \\
      ($\rightarrow$ 0)
\end{tabular} 
& \begin{tabular}{c}
   \textbf{KnowMem} \\
      ($\uparrow$) 
\end{tabular}
& \begin{tabular}{c}
   \textbf{VerbMem} \\
      ($\downarrow$) 
\end{tabular}
& \begin{tabular}{c}
   \textbf{KnowMem} \\
      ($\downarrow$) 
\end{tabular}
& \begin{tabular}{c}
   \textbf{PrivLeak} \\
      ($\rightarrow$ 0)
\end{tabular} 
& \begin{tabular}{c}
   \textbf{KnowMem} \\
      ($\uparrow$) 
\end{tabular}
\\ 
\midrule
\multicolumn{10}{c}{\textbf{MUSE-Books}}\\
\midrule
0\% & No unlearning &
99.56  & 58.32  & -56.32   & 67.01
&
99.56  & 58.32  & -56.32   & 67.01
 \\
\midrule
0\% & Retrain &
14.30 & 28.90 & 0.00   & 74.50 
&
14.30 & 28.90 & 0.00   & 74.50 
 \\
\midrule
100\% & Full forget Set
& 5.38 %$_{\pm{0.17}}$ 
& 18.72 %$_{\pm{13.49}}$ 
&  -16.98 %$_{\pm{10.41}}$ 
& 40.34 %$ %_{\pm{24.50}}$  
& 0.00 %$ %_{\pm{0.00}}$ 
& 0.00 %$_{\pm{0.00}}$ 
&  -31.02 %$_{\pm{1.04}}$ 
& 31.33 %$_{\pm{3.67}}$ 
\\
\midrule
\multirow{4}{*}{
\begin{tabular}{c}
   10\% 
\end{tabular}
}
& \random{}
& 4.34$_{\pm{1.40}}$ 
& 23.86$_{\pm{10.79}}$ 
&  -12.79$_{\pm{4.86}}$ 
& 56.67$_{\pm{7.29}}$  
& 0.00$_{\pm{0.00}}$ 
& 0.00$_{\pm{0.00}}$ 
&  -27.09$_{\pm{2.22}}$ 
& 29.12$_{\pm{3.36}}$\\
&\grand{}
& 4.96
& 21.69
& 5.07
& 57.11
& 0.00
& 0.00
&  -25.28
& 37.54\\
& \moderate{}
& 5.72
& 9.02
& -19.84
& 33.44
& 0.00
& 0.00
& -28.42
& 36.55\\
%%%  Mink for NPO 0.5
& \mink{}
& 7.53
& 20.12
& -29.17
& 56.43
& 0.00
& 0.00
& -0.24
& 33.21 \\
\midrule
\multirow{4}{*}{
\begin{tabular}{c}
   5\% 
\end{tabular}
}
%%%  random for RMU 0.5
& \random{}
& 4.01$_{\pm{1.58}}$ 
& 19.37$_{\pm{6.75}}$ 
&  -18.61$_{\pm{1.88}}$ 
& 54.62$_{\pm{5.54}}$  

%%%  random for NPO 0.5
& 0.00$_{\pm{0.00}}$ 
& 3.48$_{\pm{0.56}}$ 
&  -8.97$_{\pm{8.03}}$ 
& 36.19$_{\pm{1.35}}$\\
&\grand{}
%%%  grand for RMU 0.5
& 5.69
& 28.00
& -37.66
& 59.21

%%%  grand for NPO 0.5
& 0.00
& 3.77
&  -15.71
& 40.15 \\  
& \moderate{}
%%%  Moderate for RMU 0.5
& 4.75
& 7.08
& -18.02
& 33.92

%%%  Moderate for NPO 0.5
& 0.00
& 3.35
&  -5.63
& 36.93\\ 
%%%  Mink for RMU 0.5
& \mink{}
& 4.20
& 37.48
& -0.12
& 67.76

%%%  Mink for NPO RMU 0.5
& 0.00
&  4.33
& -32.90
& 39.18\\

%%% MUSE NEWS
\midrule
\multicolumn{10}{c}{\textbf{MUSE-News}}\\
\midrule
0\% & No unlearning &
58.29  & 62.93  & -98.71    & 54.31
&
58.29  & 62.93  & -98.71    & 54.31
 \\
\midrule
0\% & Retrain &
20.75 & 33.32 & 0.00    & 53.79
&
20.75 & 33.32 & 0.00    & 53.79
\\
 \midrule
100\% & Full forget set
%%%  Random for RMU 1
& 21.00 
& 54.68 
&  1.80 
& 44.75 

%%%  Random for NPO 1
& 0.00 
& 47.96 
&  107.40 
& 37.86 
\\
\midrule
\multirow{4}{*}{
\begin{tabular}{c}
   10\% 
\end{tabular}
}
& \random{}
%%%  Random for RMU 0.1
& 29.97$_{\pm{2.50}}$ 
& 18.85$_{\pm{21.99}}$ 
&  -38.87$_{\pm{2.78}}$ 
& 50.23$_{\pm{1.67}}$  

%%%  Random for NPO 0.1
& 20.54$_{\pm{1.71}}$ 
& 42.30$_{\pm{1.26}}$ 
&  -99.58$_{\pm{0.14}}$ 
& 38.54$_{\pm{0.61}}$\\
&\grand{}
& 28.85
& 40.50
& -45.84
& 49.50
& 21.35
& 41.97
& -99.71
& 38.59
\\
& \moderate{}
& 32.62
& 38.40
& -36.44
& 52.77
& 19.26
& 42.46
& -99.78
& 37.99
\\
%%%  Mink for NPO 0.5
& \mink{}
& 31.67
& 2.02
& -15.95
& 50.14
& 23.59
& 43.85
& -98.14
& 40.66 \\
\midrule
\multirow{4}{*}{
\begin{tabular}{c}
   5\% 
\end{tabular}
}
%%%  random for RMU 0.5
& \random{}
& 20.15$_{\pm{7.50}}$ 
& 12.95$_{\pm{17.17}}$ 
&  -16.42$_{\pm{18.70}}$ 
& 40.93$_{\pm{4.32}}$

%%%  random for NPO 0.5
& 7.36$_{\pm{0.79}}$ 
& 34.28$_{\pm{1.92}}$ 
&  -76.38$_{\pm{7.46}}$ 
& 32.75$_{\pm{1.75}}$ \\
&\grand{}
%%%  grand for RMU 0.5
& 24.15
& 50.26
& -33.27
& 47.11

%%%  grand for NPO 0.5
& 3.51
& 32.71
& -1.85
& 31.65 \\  
& \moderate{}
%%%  Moderate for RMU 0.5
& 19.37
& 52.21
& -8.53
& 47.00

%%%  Moderate for NPO 0.5
& 3.19
& 38.24
& 16.50
& 35.57 \\ 
%%%  Mink for RMU 0.5
& \mink{}
& 28.83
& 49.21
& -33.74
& 43.94

%%%  Mink for NPO RMU 0.5
& 3.40
&  36.45
& 73.07
& 31.21\\

\midrule
\bottomrule
\end{tabular}
}
\label{tab: muse}
% \vspace*{-2mm}
\end{center}
\end{table}
