# Supplementary material for: LLM Unlearning Reveals a Stronger-Than-Expected Coreset Effect in Current Benchmarks
Source: arXiv:2504.10185 source file (2025-04-16)
Supplement: Supplementary file 6 [file app_npormu.tex]

\section{Details of NPO and RMU}
\label{app: npormu}

\makeatother
\setcounter{table}{0}
\setcounter{equation}{0}

In this section, we provide details explaining the two main unlearning methods we consider in this paper.

\paragraph{Negative Preference Optimization (NPO).}

NPO \citep{zhang2024negative} reduces the model’s preference for the forget set $\Df$ by treating it analogously to negative responses in preference optimization, but omitting the positive response term. This yields the following loss function, which has been shown to achieve lower divergence rates compared to various other unlearning approaches:
\begin{align}
  & \ell_{\mathrm{NPO}}(\boldsymbol{\theta}) =  \mathbb E_{(x,y) \in \Df} \underbrace{\left [    - \frac{2}{\beta} \log \sigma  \left ( - \beta \log \left ( \frac{\pi_{\btheta} (y | x) }{\pi_{\mathrm{ref}} (y | x)}\right ) \right ) 
    \right ]}_{\lf \  \text{specified in}  \ \eqref{eq: LLM_MU}}
\label{eq:NPO}
\end{align}
where $\sigma (t) = 1/(1+e^{-t})$ is the sigmoid function, $\beta > 0 $ is a hyperparameter. Minimizing the above forget loss drives  the model to be unlearned $\pi_{\btheta}$ \textit{away} from the reference model $\pi_{\mathrm{ref}}$ for the samples from the forget set. In NPO, the retain loss $\lr$ is simply the prediction loss \textit{i.e.} the cross entropy loss between $x$ and $y$, which are obtained from $\Dr$.

\paragraph{Representation Misdirection Unlearning (RMU).}
RMU \citep{li2024wmdp} seeks to degrade the model's internal representations for the forget set, thereby reducing its ability to recall or generate undesired knowledge. Specifically, it aligns the hidden state activations of the unlearned model at a given layer $l$ (denoted $\pi_{\btheta}^l$) with a random unit vector $\mathrm{u}$, where each component of $\mathrm{u}$ is sampled independently and uniformly from $[0,1)$. In contrast to NPO, RMU also includes a retain loss that ensures the model’s representations on the retain dataset remain consistent with those of the reference (pre-unlearned) model. Considering $z_f$ and $z_r$ to be samples from the forget and retain set respectively,this is formalized as follows:
% \SL{[In the above, $z_f$ and $z_r$ were not defined.]}
%
% RMU \citep{li2024wmdp} which aims to degrade the representation of the unlearned model for the forget set. This degradation is mainly done by making the hidden state activations of the unlearned model at some layer $l$ (denoted by $\pi_{\btheta}^l$) to be similar to a random unit vector $\mathrm{u}$, where each value is independently and uniformly sampled from $[0,1)$.
% Unlike NPO, the retain loss here enforces alignment of the unlearned model representation with that of the reference model for the retain dataset. This is obtained in the following way:
\begin{align}
  & \ell_{\mathrm{RMU}}(\boldsymbol{\theta}) =  
  \mathbb E_{z_f \in \Df} \underbrace{\left [ \frac{1}{\mathrm{L_f}}\sum_{\text{token} \ t\in z_f} \|  \pi_{\btheta}^l (t) - c \cdot \mathrm{u}\|_2^2
    \right ]}_{\lf \  \text{specified in}  \ \eqref{eq: LLM_MU}} + \lambda
  \mathbb E_{z_r \in \Dr} \underbrace{\left [ \frac{1}{\mathrm{L_r}}\sum_{\text{token} \ t\in z_r} \|  \pi_{\btheta}^l (t) -\pi_{\mathrm{ref}}^l (t)\|_2^2
    \right ]}_{\lr \  \text{specified in}  \ \eqref{eq: LLM_MU}}
\label{eq:RMU}
\end{align}
where $\mathrm{L_f}$, $\mathrm{L_r}$ are the number of tokens in $z_f$, $z_r$ respectively and  $c$ controls the strength of $\mathbf u$.
