# Supplementary material for: LLM Unlearning Reveals a Stronger-Than-Expected Coreset Effect in Current Benchmarks
Source: arXiv:2504.10185 source file (2025-04-16)
Supplement: Supplementary file 7 [file app_o1prompt.tex]

\section{Prompt to Extract Keywords}
\label{app: prompt}

\makeatother
\setcounter{table}{0}
\setcounter{equation}{0}

% We use the following prompt to extract the relevant keywords from WMDP-Bio

\begin{prompt}{Prompt to Extract Keywords using LLM-as-a-Judge}\label{prompt:meta}
% \small
\textbf{System}:
\\
\\
You are an expert in chemistry, biology and diseases. I will provide you with a text, and your task is to carefully analyze each word and determine if it is related to chemistry or biology and disease. For every word that is related to chemistry, biology and disease, replace it with an asterisk (*) in the original text while keeping all other words unchanged. Think step by step and ensure accuracy in identifying only chemistry, biology and disease-related terms. Pay close attention to scientific terminology. Return the result in the following format:\\
\{\{ \\
"replaced\_text": "$<$text after replacing$>$",\\
"related\_words": ["word1", "word2", "word3", ...] \\
\}\} \\
Do \textbf{not} write any code. Use your linguistic and scientific knowledge to analyze the text.
\\
\\
\textbf{User}: 
\\
\\
{\color{blue}\{WMDP-Bio forget set\}}
\\
\\
\textbf{Assistant}:
\\
\\
{\color{blue}\{response\}}

\end{prompt}
