# Supplementary material for: LLM Unlearning Reveals a Stronger-Than-Expected Coreset Effect in Current Benchmarks
Source: arXiv:2504.10185 source file (2025-04-16)
Supplement: Supplementary file 8 [file app_overlap.tex]

\section{Additional Details of Keyword Explanation Experiment}
\label{app: keyword_overlap}

\makeatother
\setcounter{table}{0}
\setcounter{equation}{0}

%In addition to the demonstrating then unlearning effectiveness of keyword unlearned models as in Sec.\,\ref{sec: consistency}, we analyse the overlap between the keywords extracted from the full forget set and the \random{}-based coresets. 
In addition to demonstrating the unlearning effectiveness of keyword-based unlearned models in Sec.\,\ref{sec: consistency}, we further analyze the overlap between keywords extracted from the entire forget set (100\%) and those obtained from \random{}-based coresets. This comparison helps assess whether randomly selected coresets reliably capture the keywords in the full set.
For a particular coreset, let the keywords be denoted by $K_c$ and let all the keywords extracted be denoted $K_f$. Then for that coreset, we define the normalized overlap as $\frac{K_c \  \cap \  K_f}{|K_f|}$. As seen in \reffig{fig: overlap}, the overlapping keywords are higher than the fraction of data present in the coreset. 
his suggests that even information-agnostic random selection can yield a surprisingly high ratio of keyword overlap with the full forget set. For instance, a 5\% \random{}-based coreset captures approximately {14\%} of the full set’s keywords. We hypothesize that this amplified presence of high-impact keywords is a key factor enabling effective unlearning, even when using such a small, randomly selected subset.
% \SP{@SL: Please help me conclude here.}
%This potentially points to the reason for success of coreset selected 

%\begin{wrapfigure}{r}{105mm}
\begin{figure}[htb]
\centering
 \includegraphics[width=.4\textwidth]{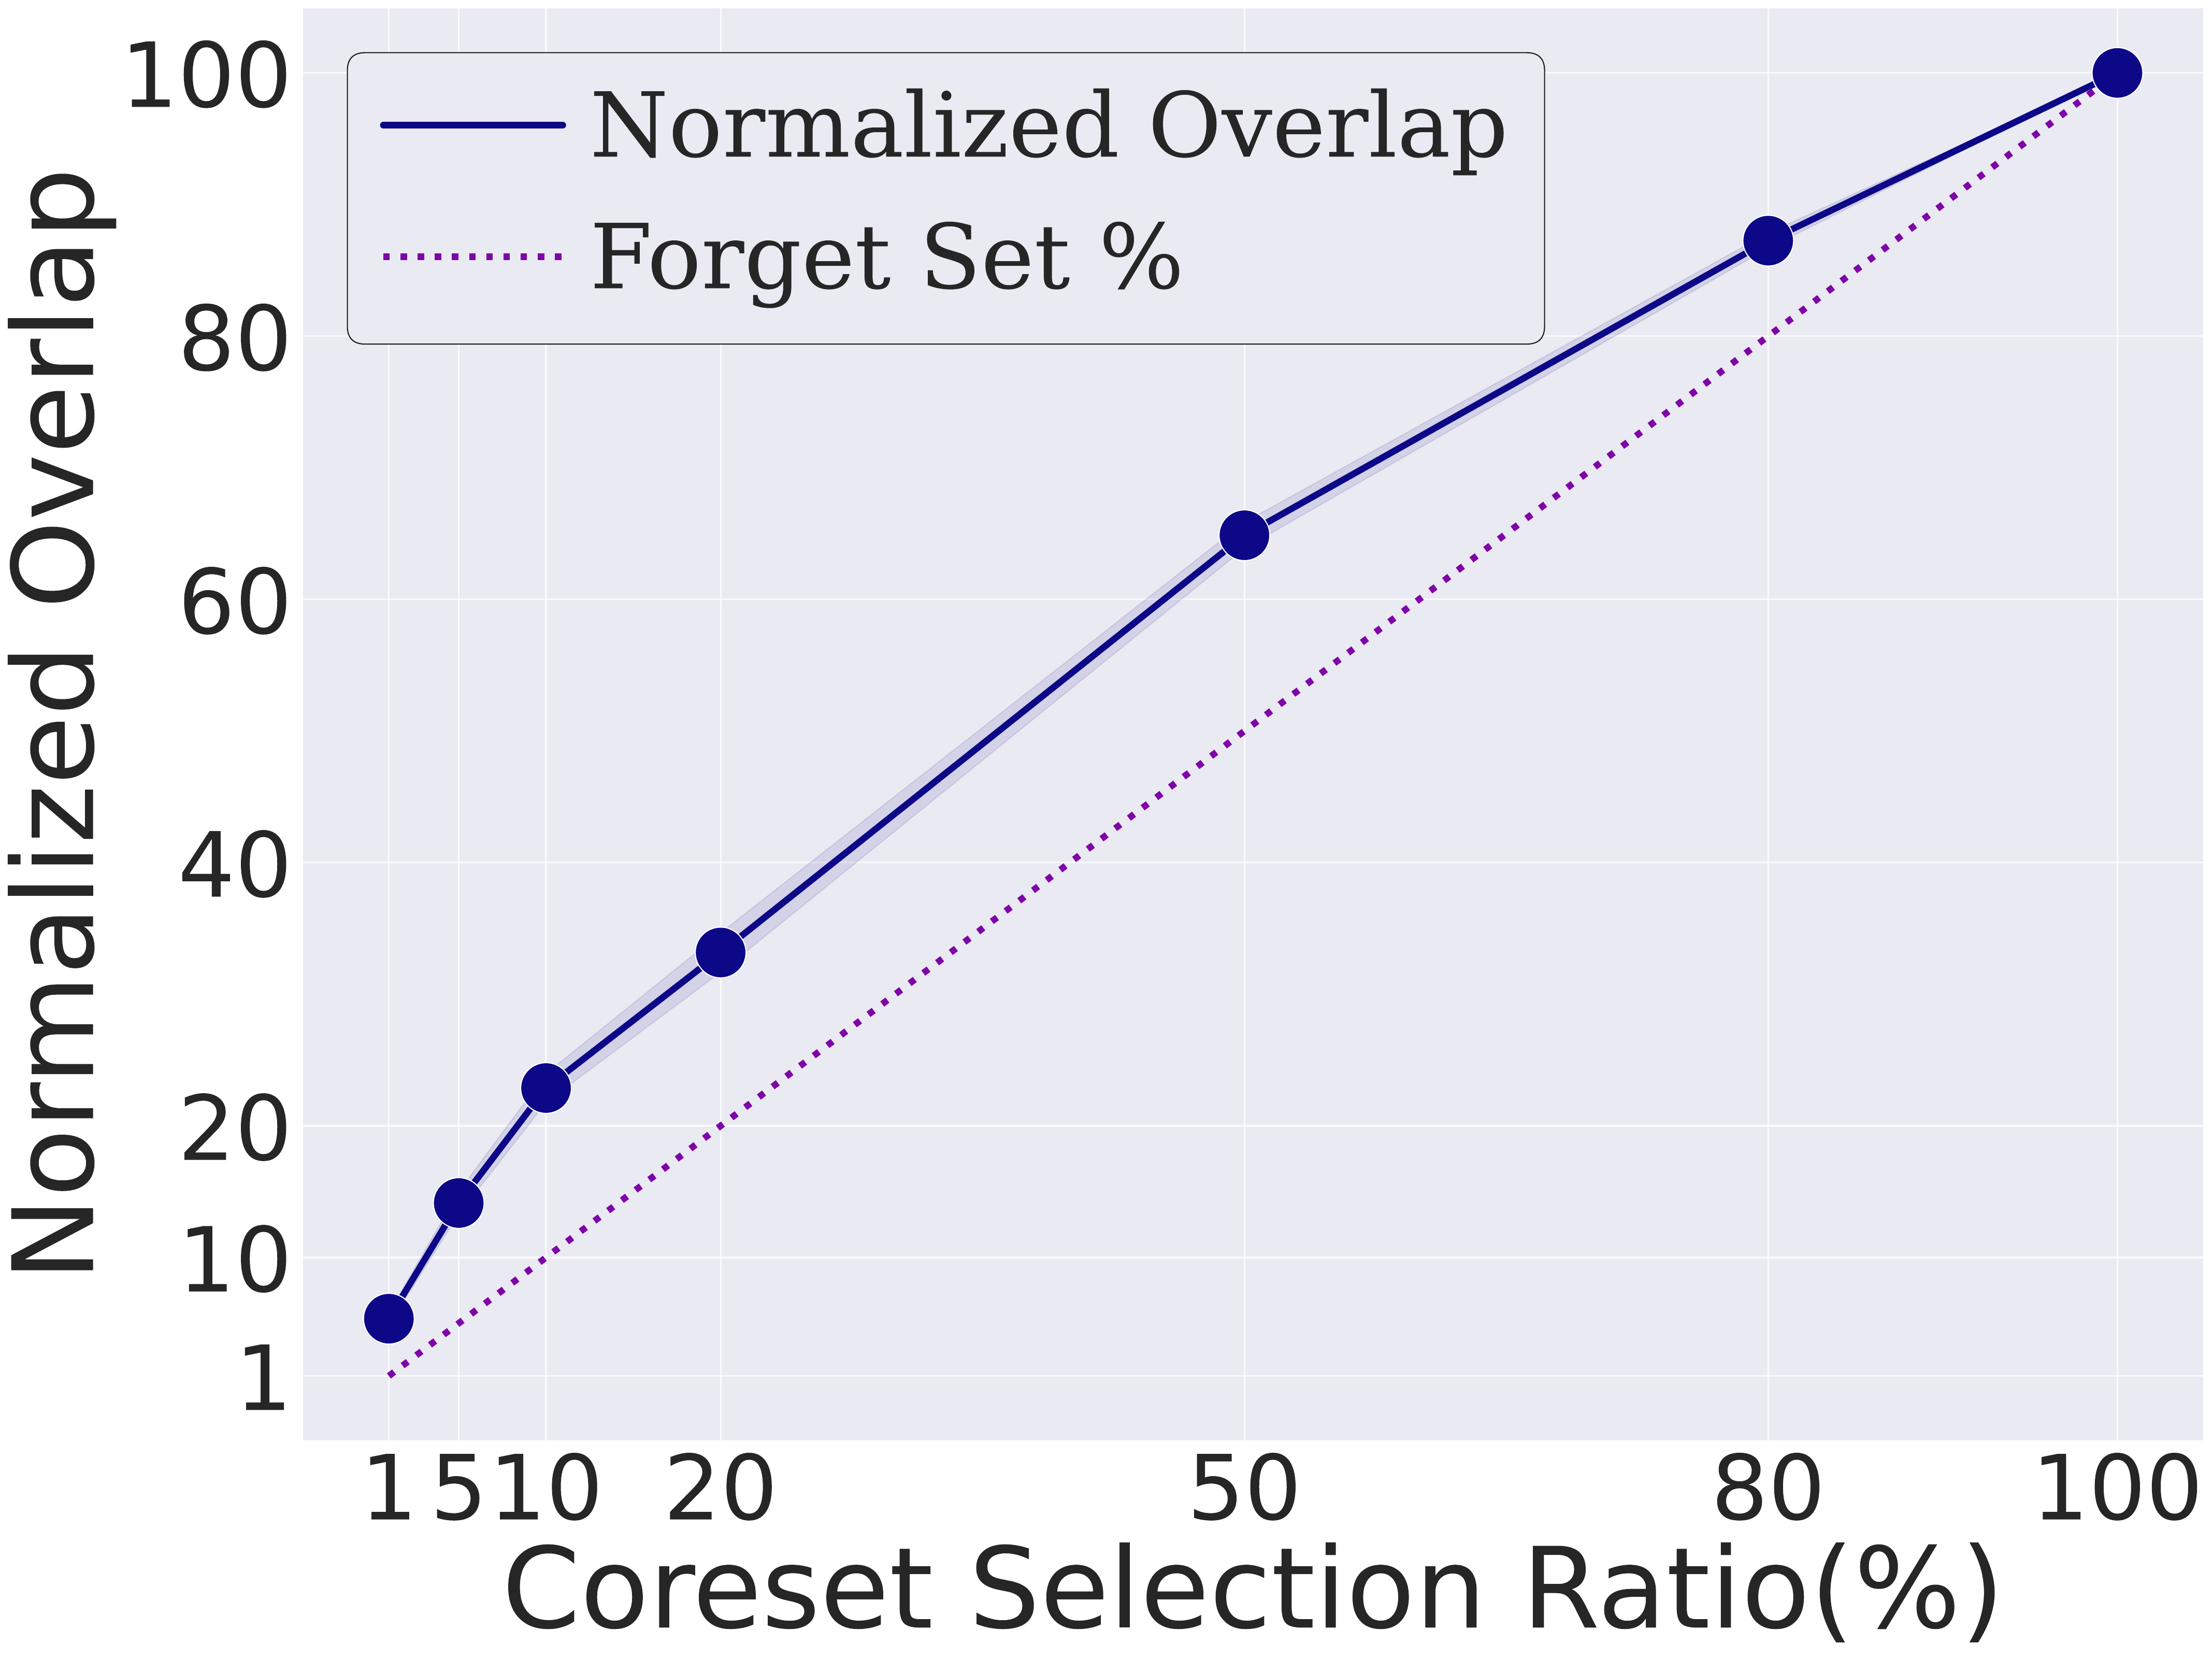}
\vspace*{-2mm}
\caption{\small{
Normalized overlapping ratio (\%) of keywords between \random{}-based coresets and the full forget set for WMDP-Bio. The dotted line represents the percentage of data present in the coreset from the forget set. Results are reported in the form $a \pm 2b$, where $a$ is the mean and $b$ is the standard deviation, computed over 3 independent trials.
}}
  \label{fig: overlap}
  %\vspace*{-6mm}
%\end{wrapfigure}
\end{figure}
