# Supplementary material for: LLM Unlearning Reveals a Stronger-Than-Expected Coreset Effect in Current Benchmarks
Source: arXiv:2504.10185 source file (2025-04-16)
Supplement: Supplementary file 9 [file app_utility.tex]

% \paragraph{Additional utility evaluation of unlearned LLMs using coresets.}
\section{Additional Utility Evaluation of Unlearned LLMs Using Coresets.}
\label{app: utility}

\makeatother
\setcounter{table}{0}
\setcounter{equation}{0}

As shown by the coreset unlearning performance in standard benchmarks (Sec.\,\ref{sec: consistency}), a surprising finding is that coreset unlearning can achieve lossless UE. This naturally raises the question: Could coreset unlearning offer utility benefits as it negates the influence of fewer forget data points, thereby better preserving the model’s performance on general tasks? However, we did not observe a clear UT advantage in existing benchmarks, likely due to the limited scope of their utility evaluations, \textit{e.g.}, MMLU for WMDP and KnowMem on the retain set for MUSE, which may not fully capture the broader utility landscape of the coreset-unlearned models.

Therefore, we conduct additional utility evaluations of coreset-unlearned models, focusing on two tasks inspired by the emergent abilities of LLMs \citep{wei2022emergent}:
(1) a math addition/subtraction task involving 2–5 digit arithmetic that is orthogonal to the unlearning objective, and
(2) the TruthfulQA task that assesses factual consistency and truthfulness in LLM responses and may be inadvertently affected by unlearning.
In \reffig{fig: additional utility}, we report the zero-shot accuracy of the aforementioned utility metrics for \random{}-based coreset-unlearned models using RMU and NPO on WMDP. RMU consistently maintains strong utility across all evaluations, regardless of the coreset selection ratio. In contrast, NPO shows higher variance; however, we observe that for $n$-digit addition and subtraction, performance may benefit from using a 10\% coreset in the WMDP-Cyber setting.

\begin{figure}[htb]
\centering
\begin{tabular}{ccc}
 %\hspace*{-8mm}
  % \hspace*{-2mm}
 \includegraphics[width=.23\textwidth]{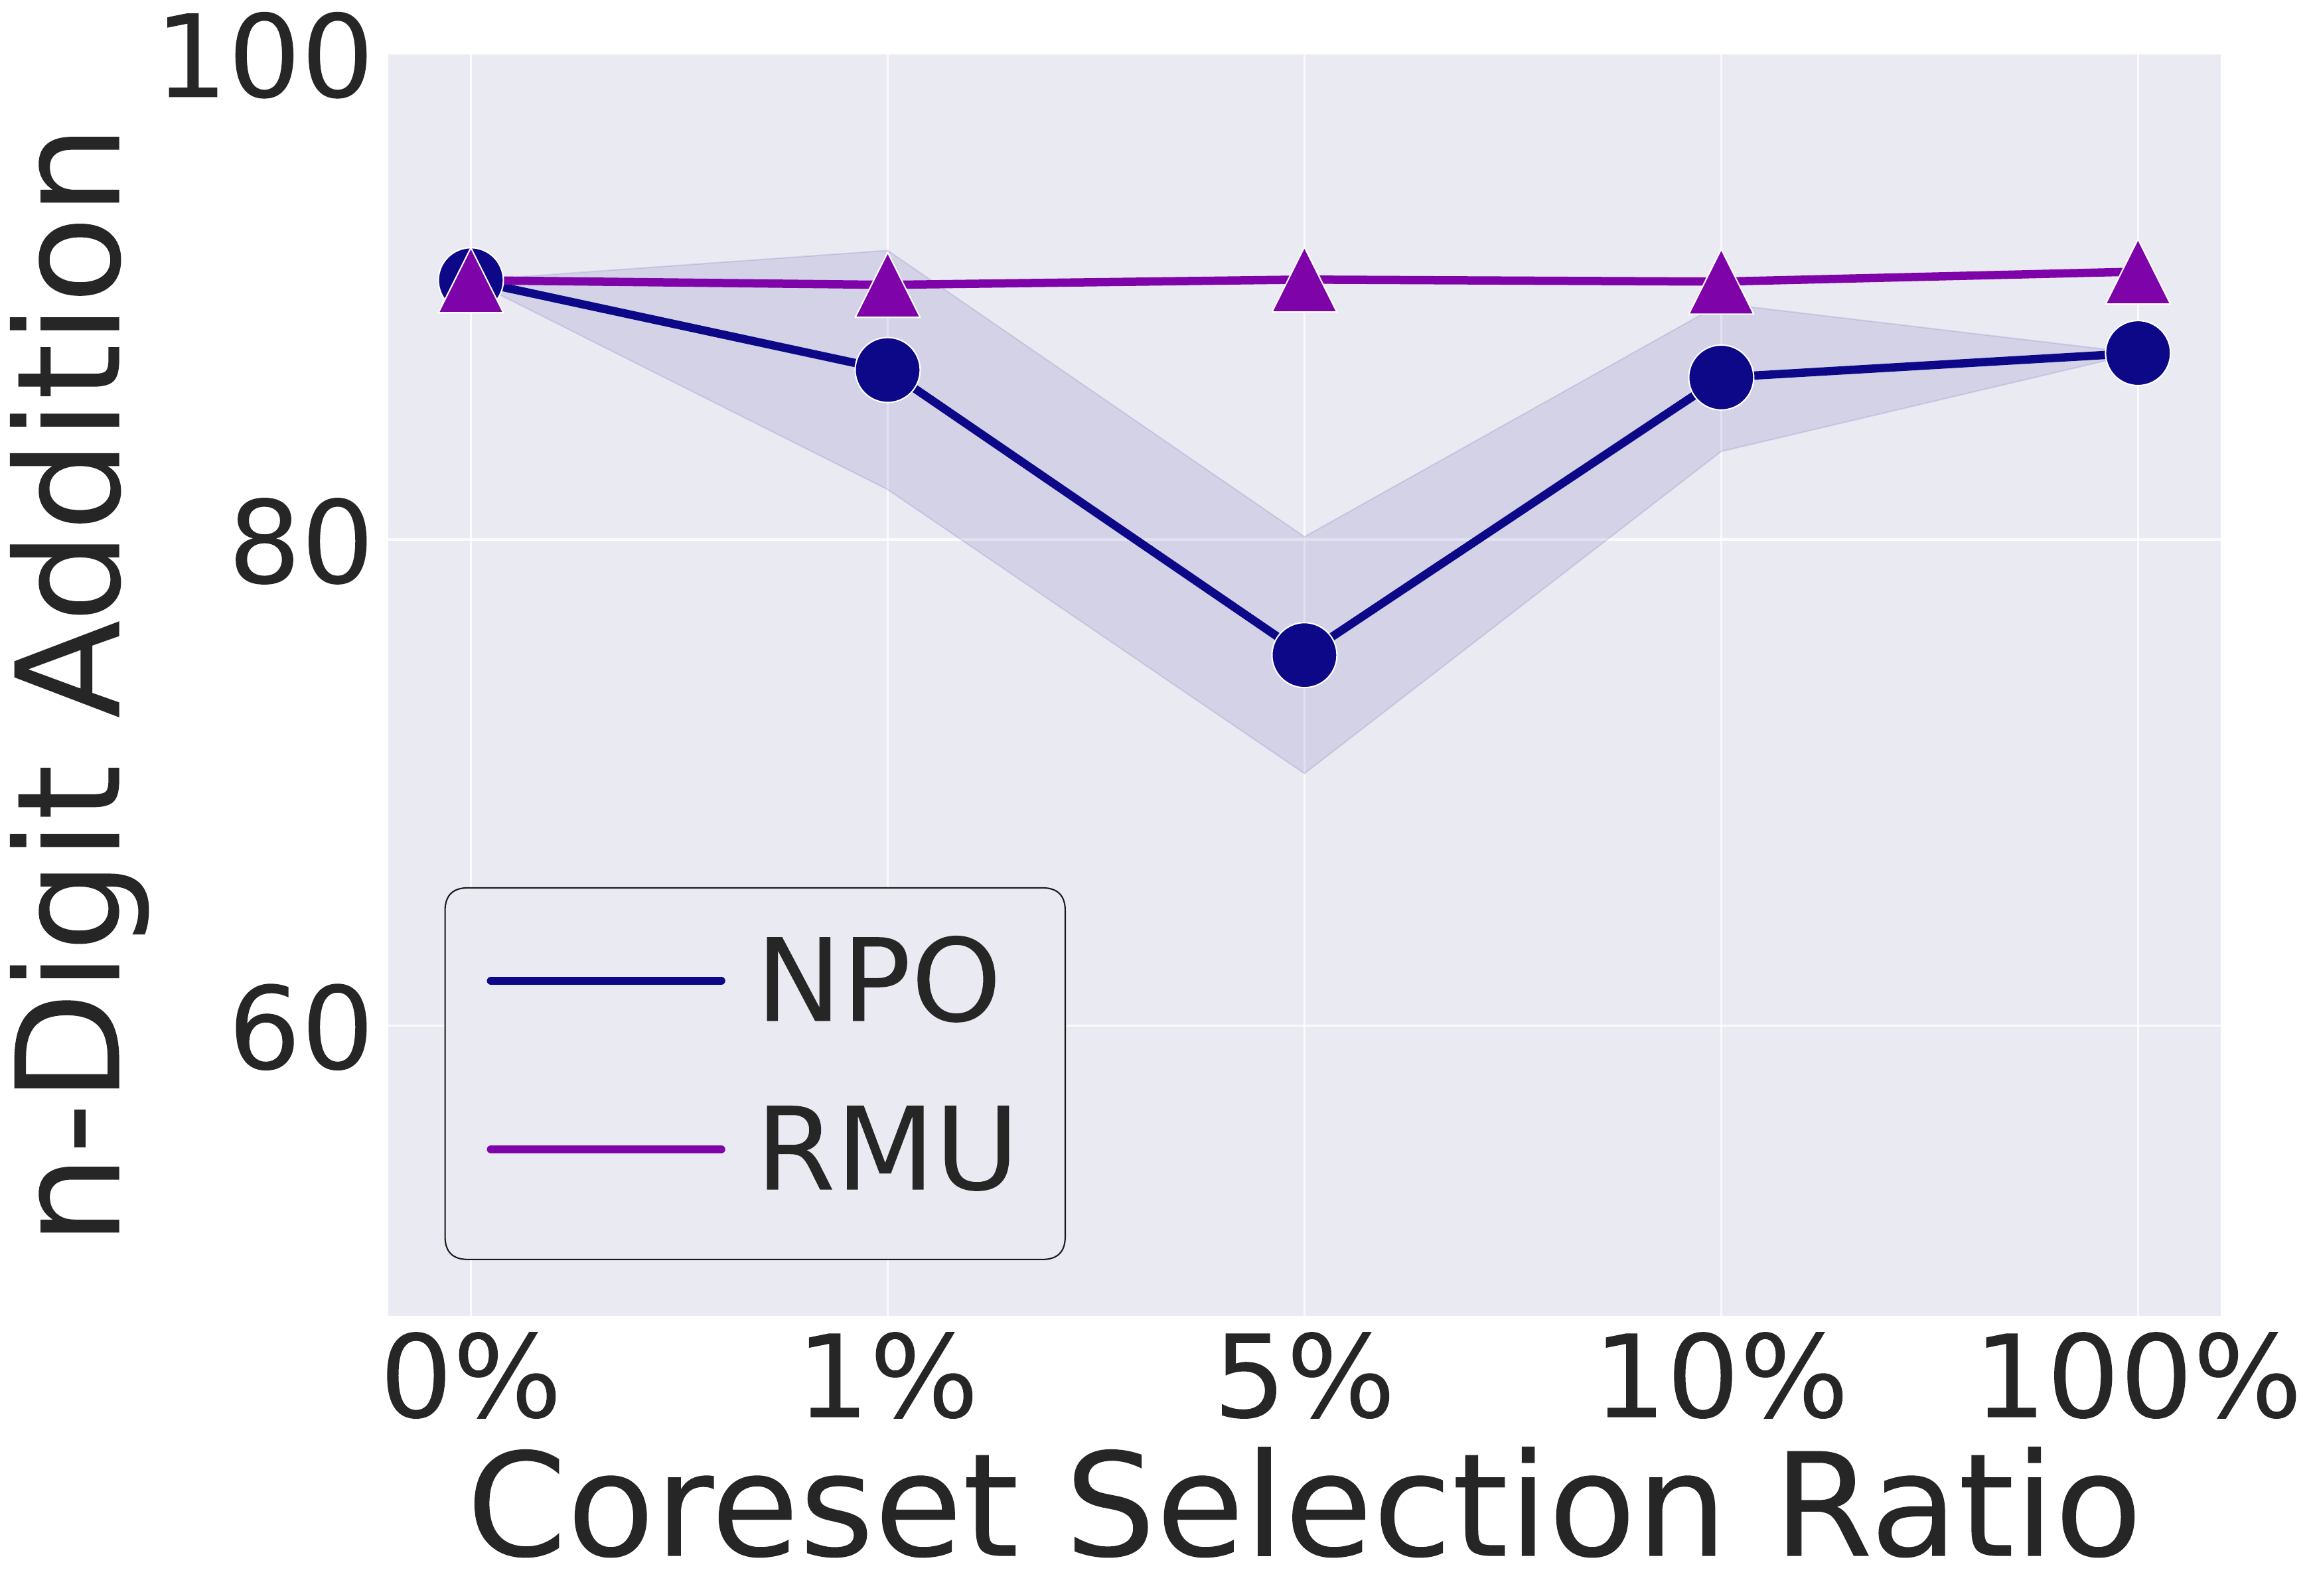}    &  
 \hspace*{-3.9mm}
 \includegraphics[width=.23\textwidth]{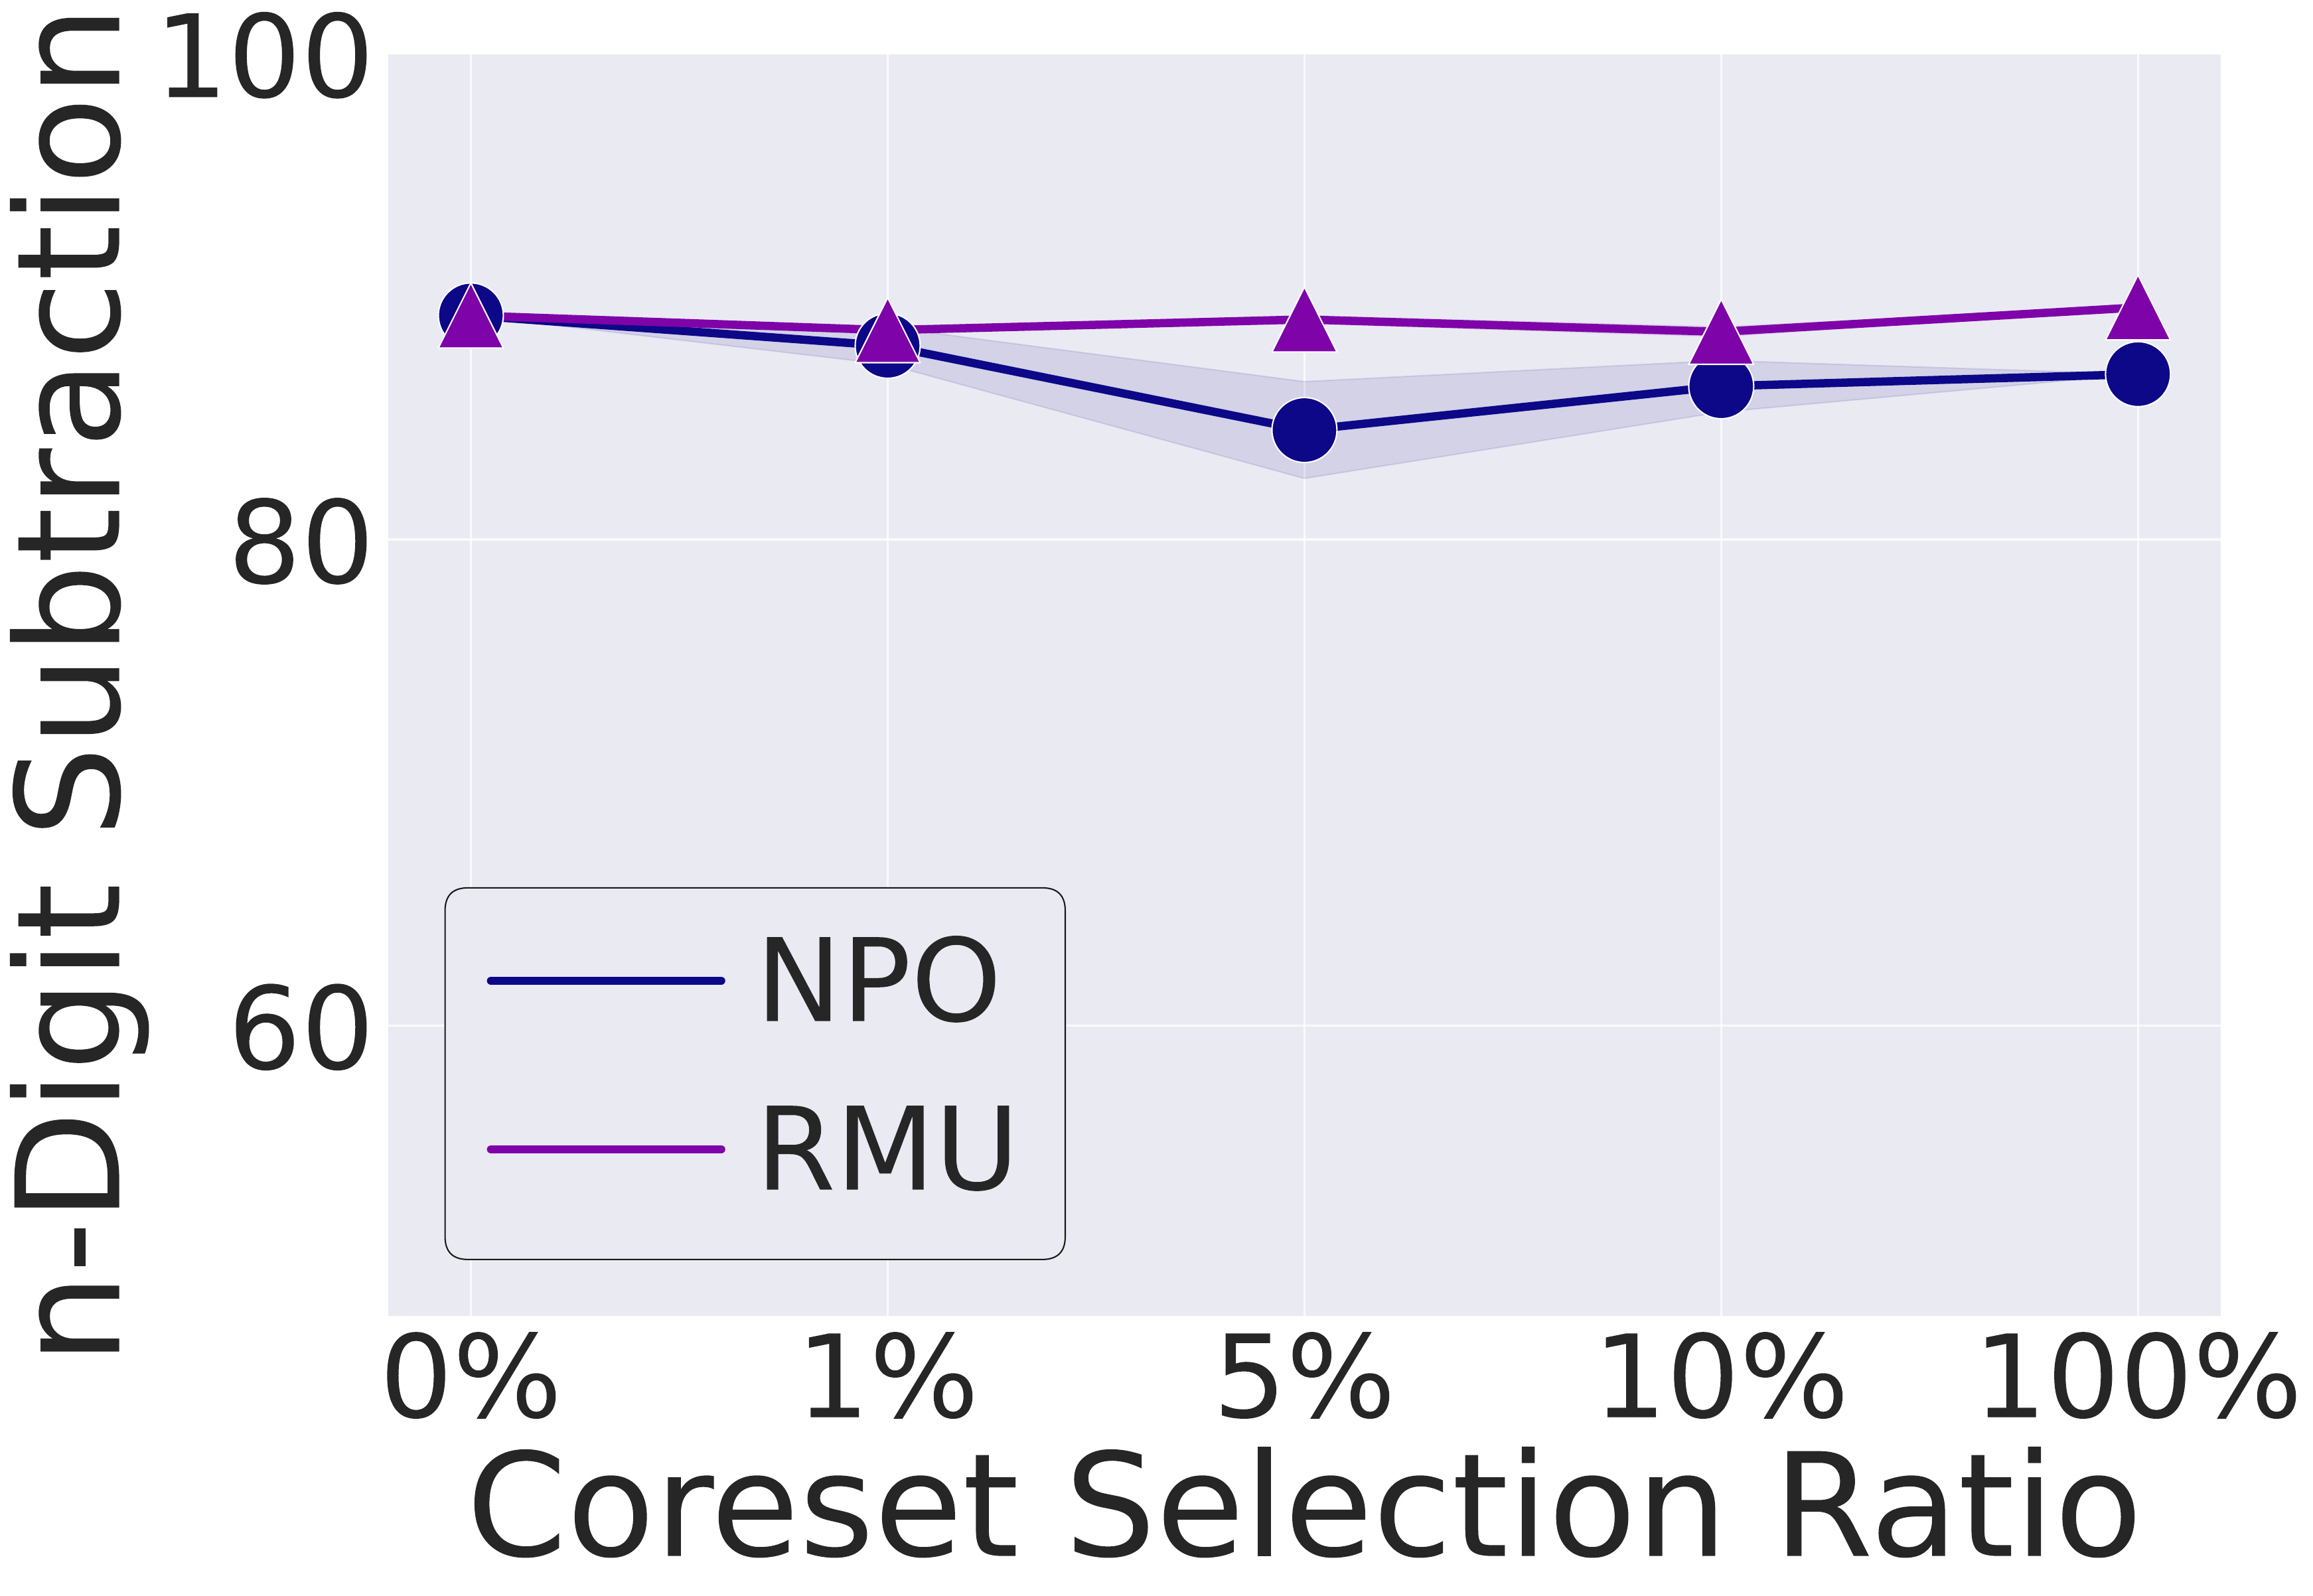} &
 \hspace*{-3.9mm}
 \includegraphics[width=.23\textwidth]{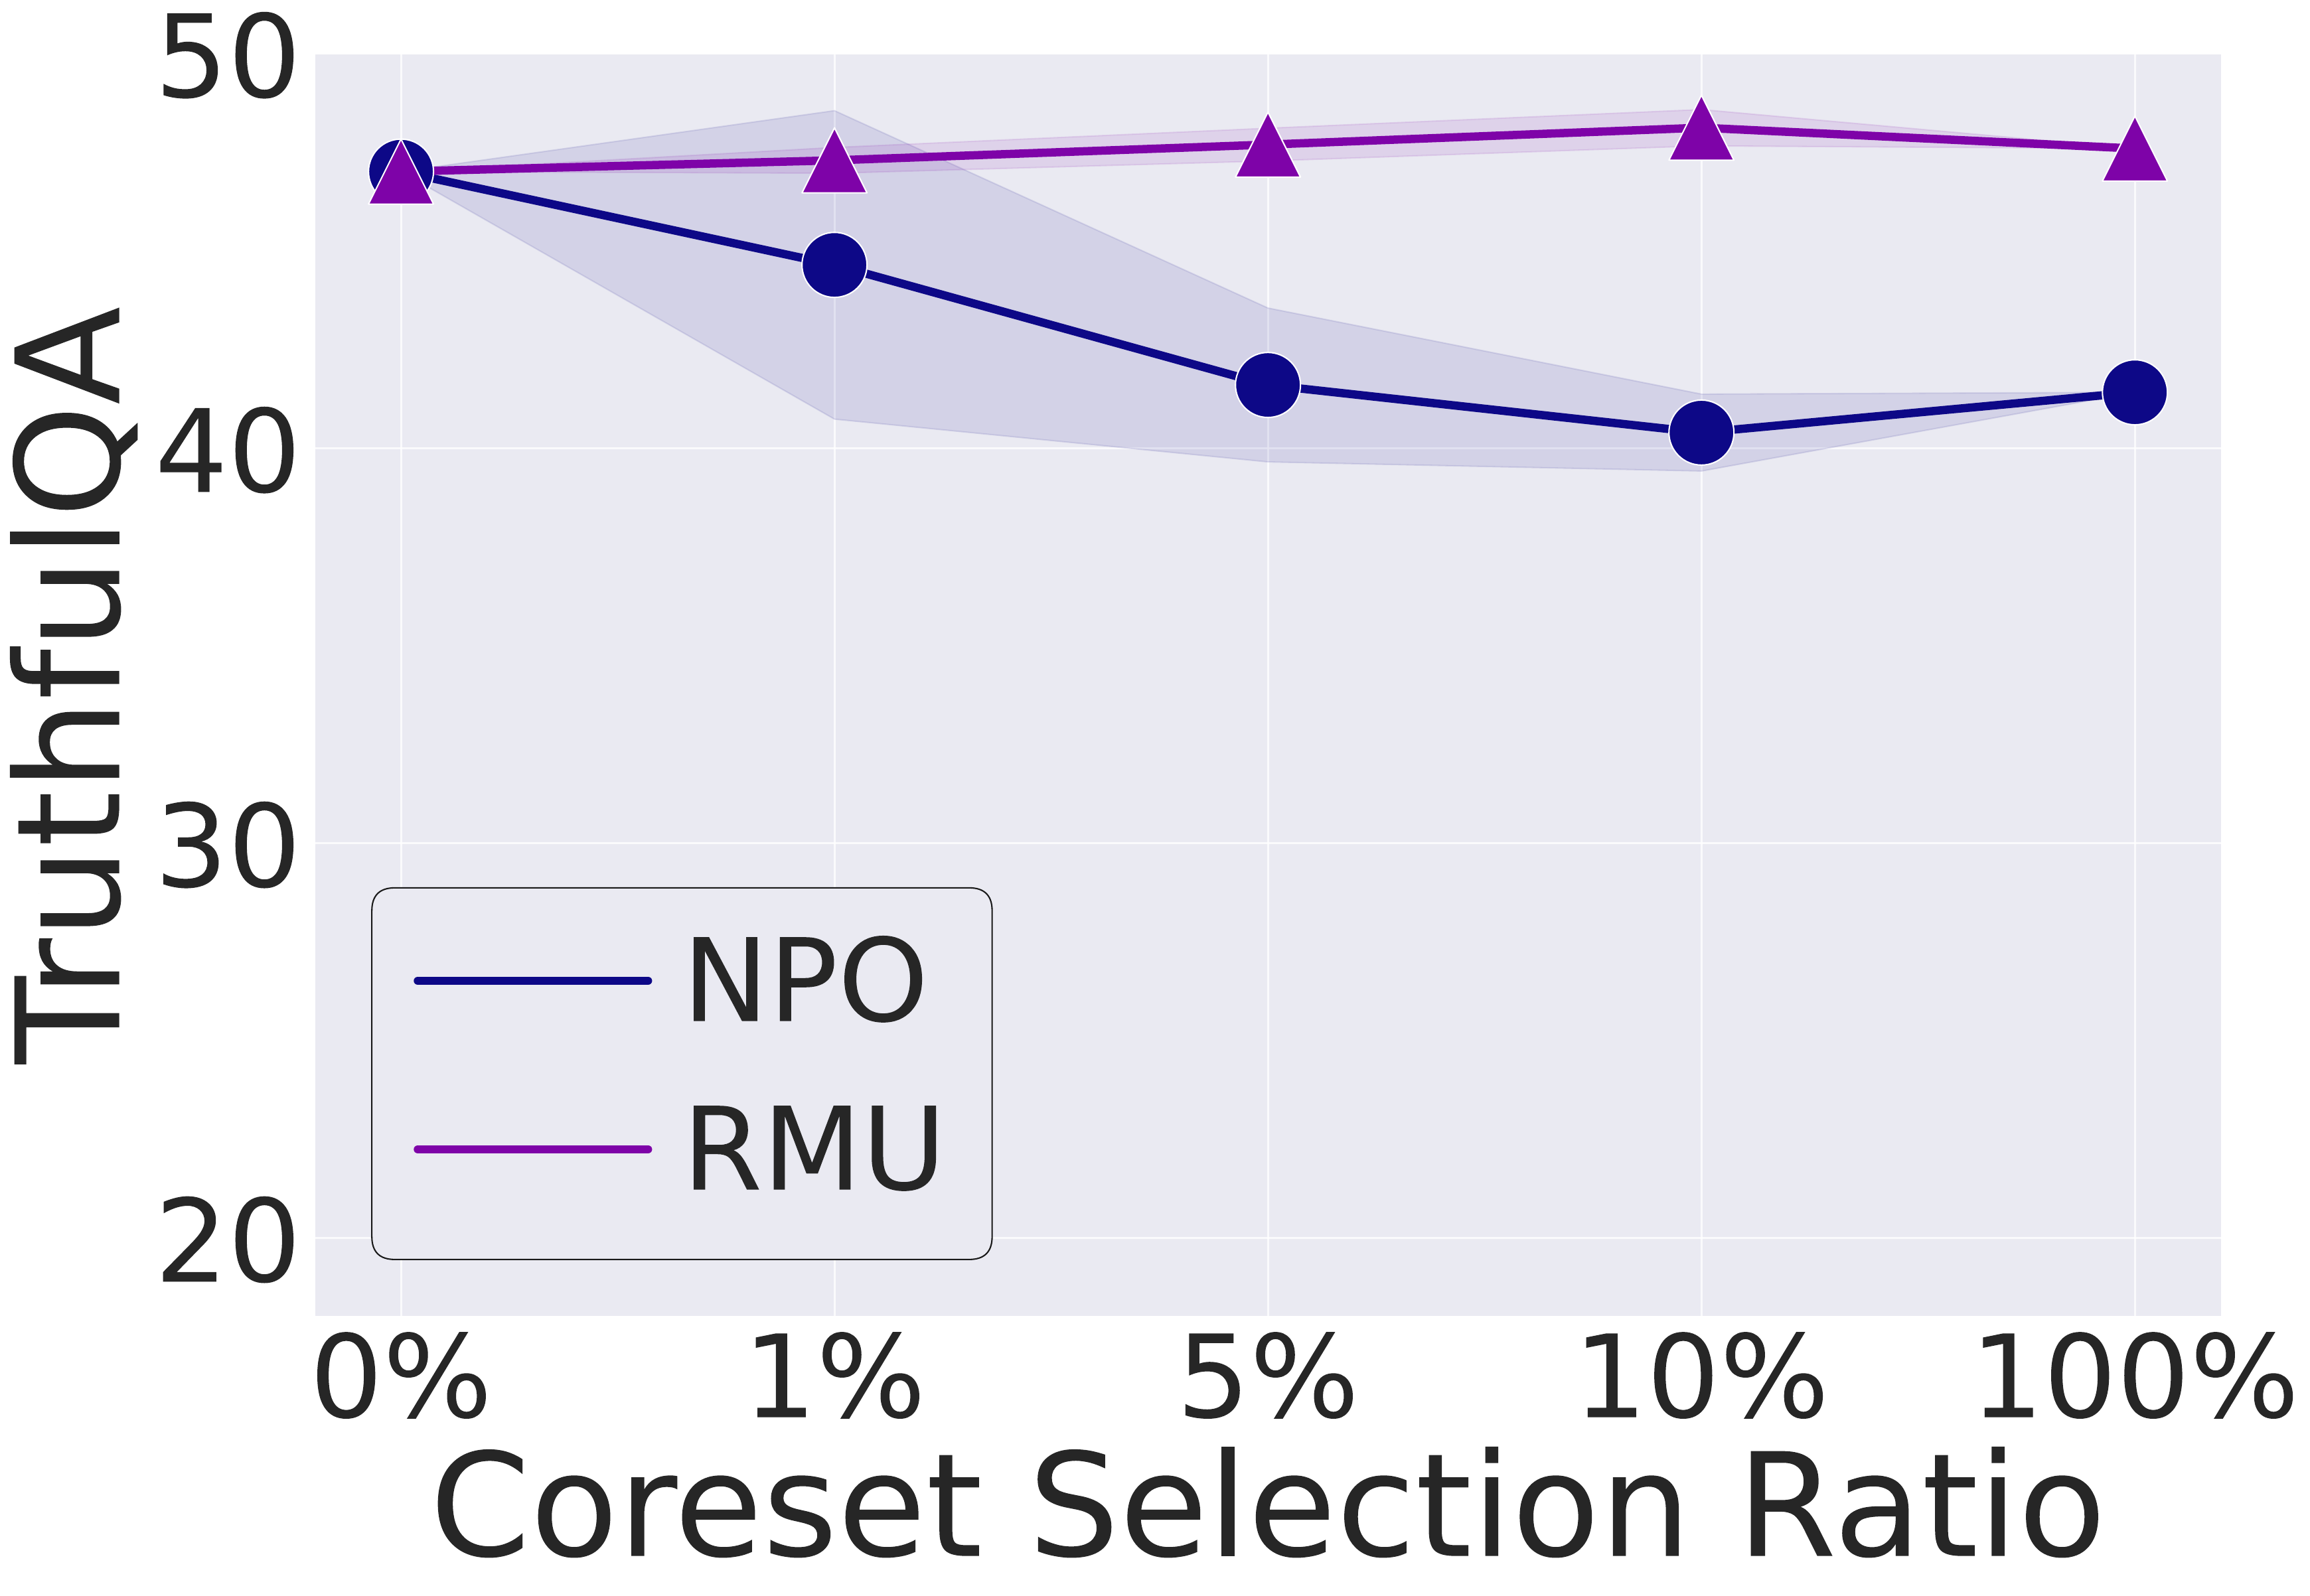}   
 \\
% {\footnotesize{(a) n-Digit Addition, WMDP-Bio}}
% & {\footnotesize{(b) n-Digit Subtraction, WMDP-Bio}}
% & {\footnotesize{(c) Truthful QA, WMDP-Bio}} 
% \\
{\footnotesize{(a) Addition, WMDP-Bio}}
& {\footnotesize{(b) Subtraction, WMDP-Bio}}
& {\footnotesize{(c) TruthfulQA, WMDP-Bio}} 
\\
\includegraphics[width=.23\textwidth]{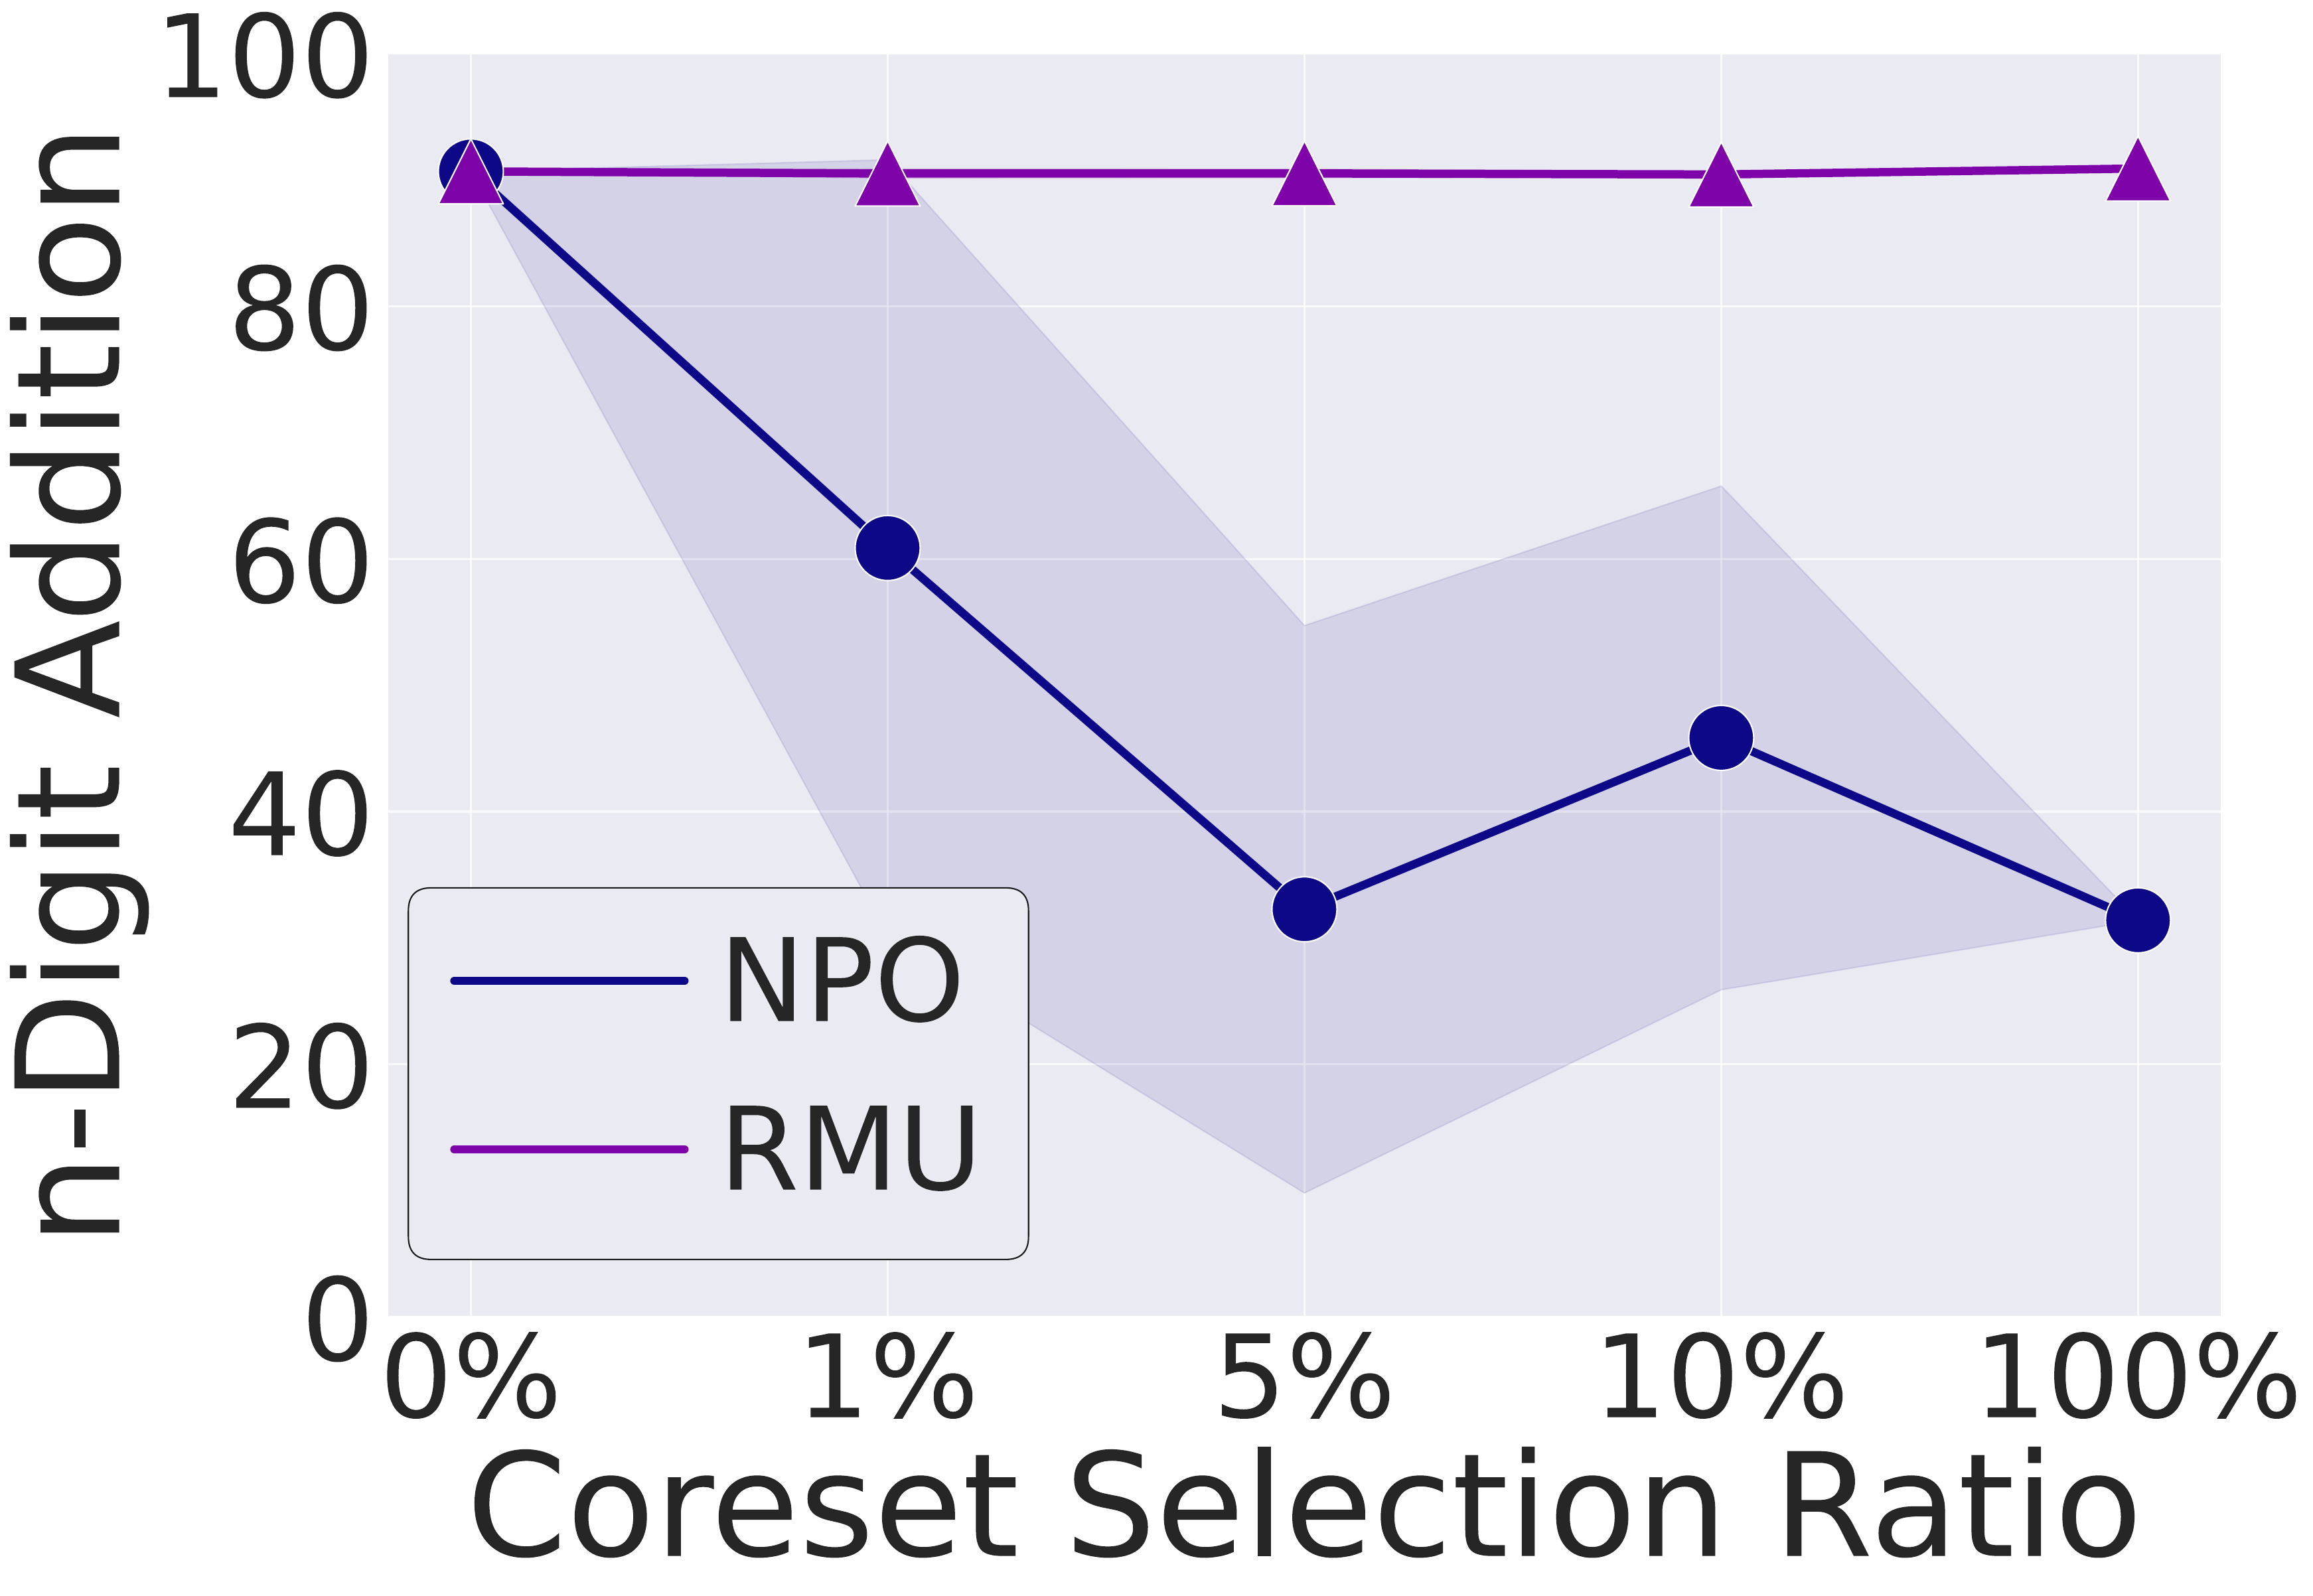}    &  
 \hspace*{-3.9mm}
 \includegraphics[width=.23\textwidth]{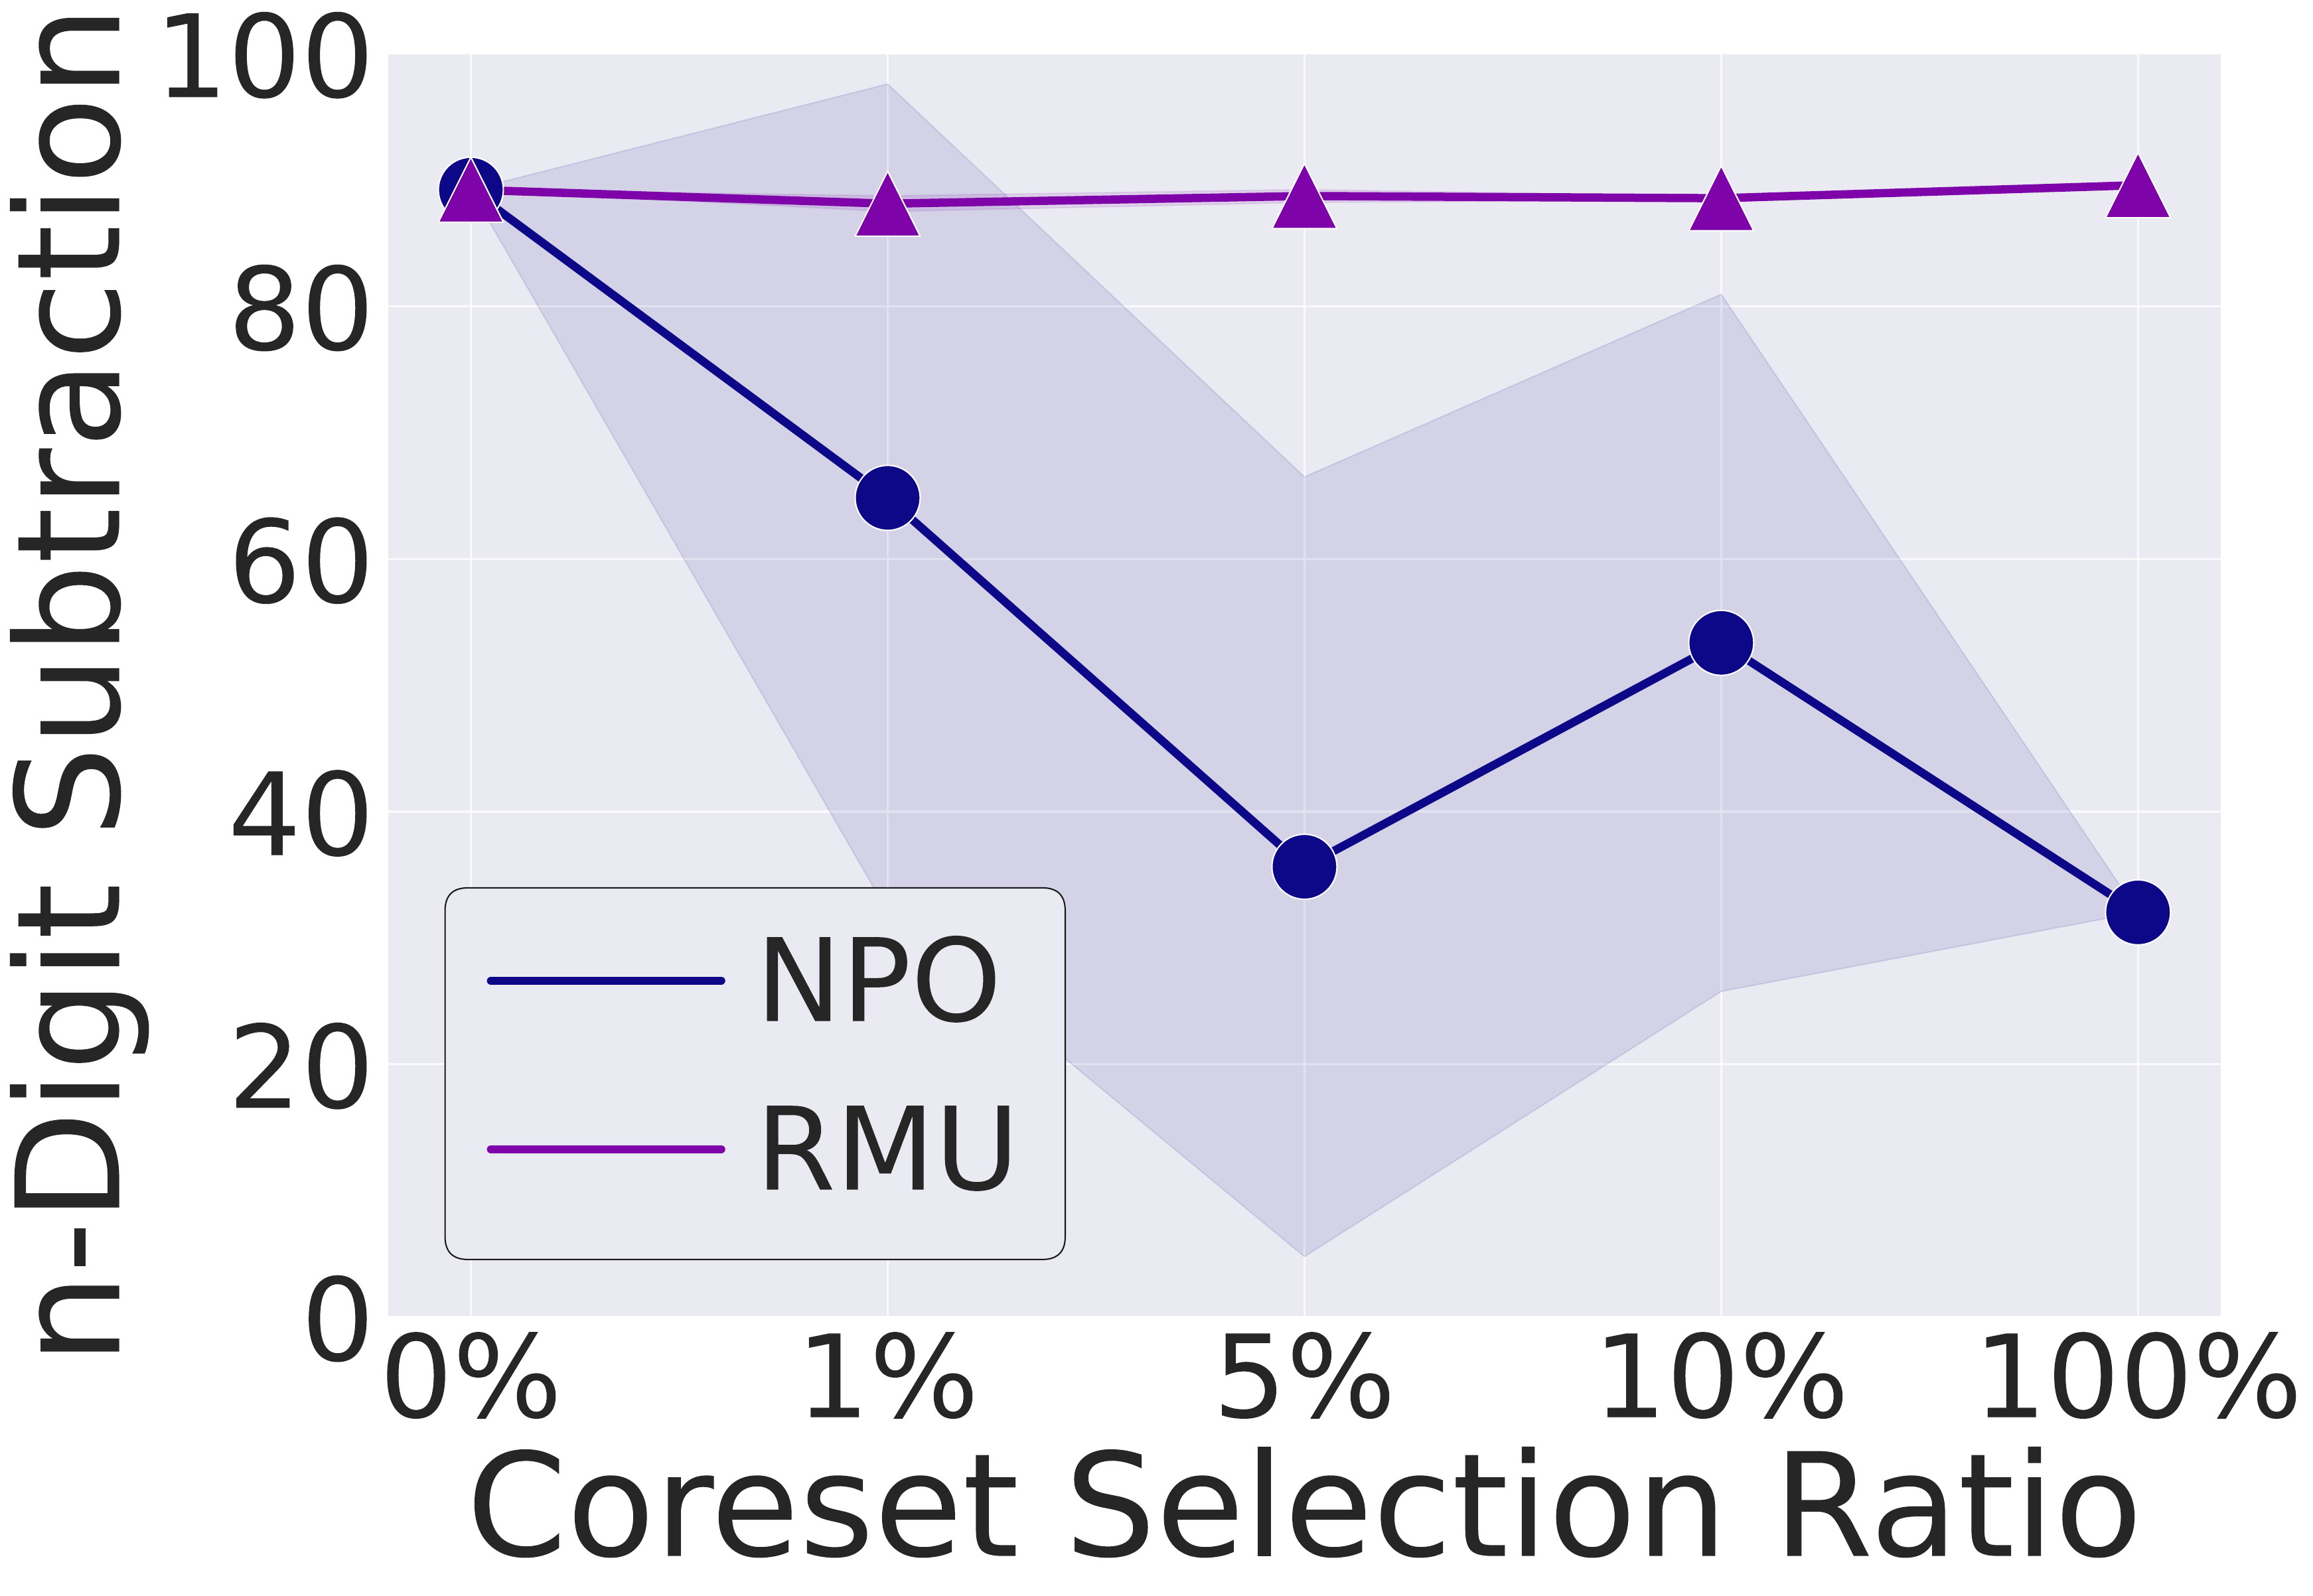} &
 \hspace*{-3.9mm}
 \includegraphics[width=.23\textwidth]{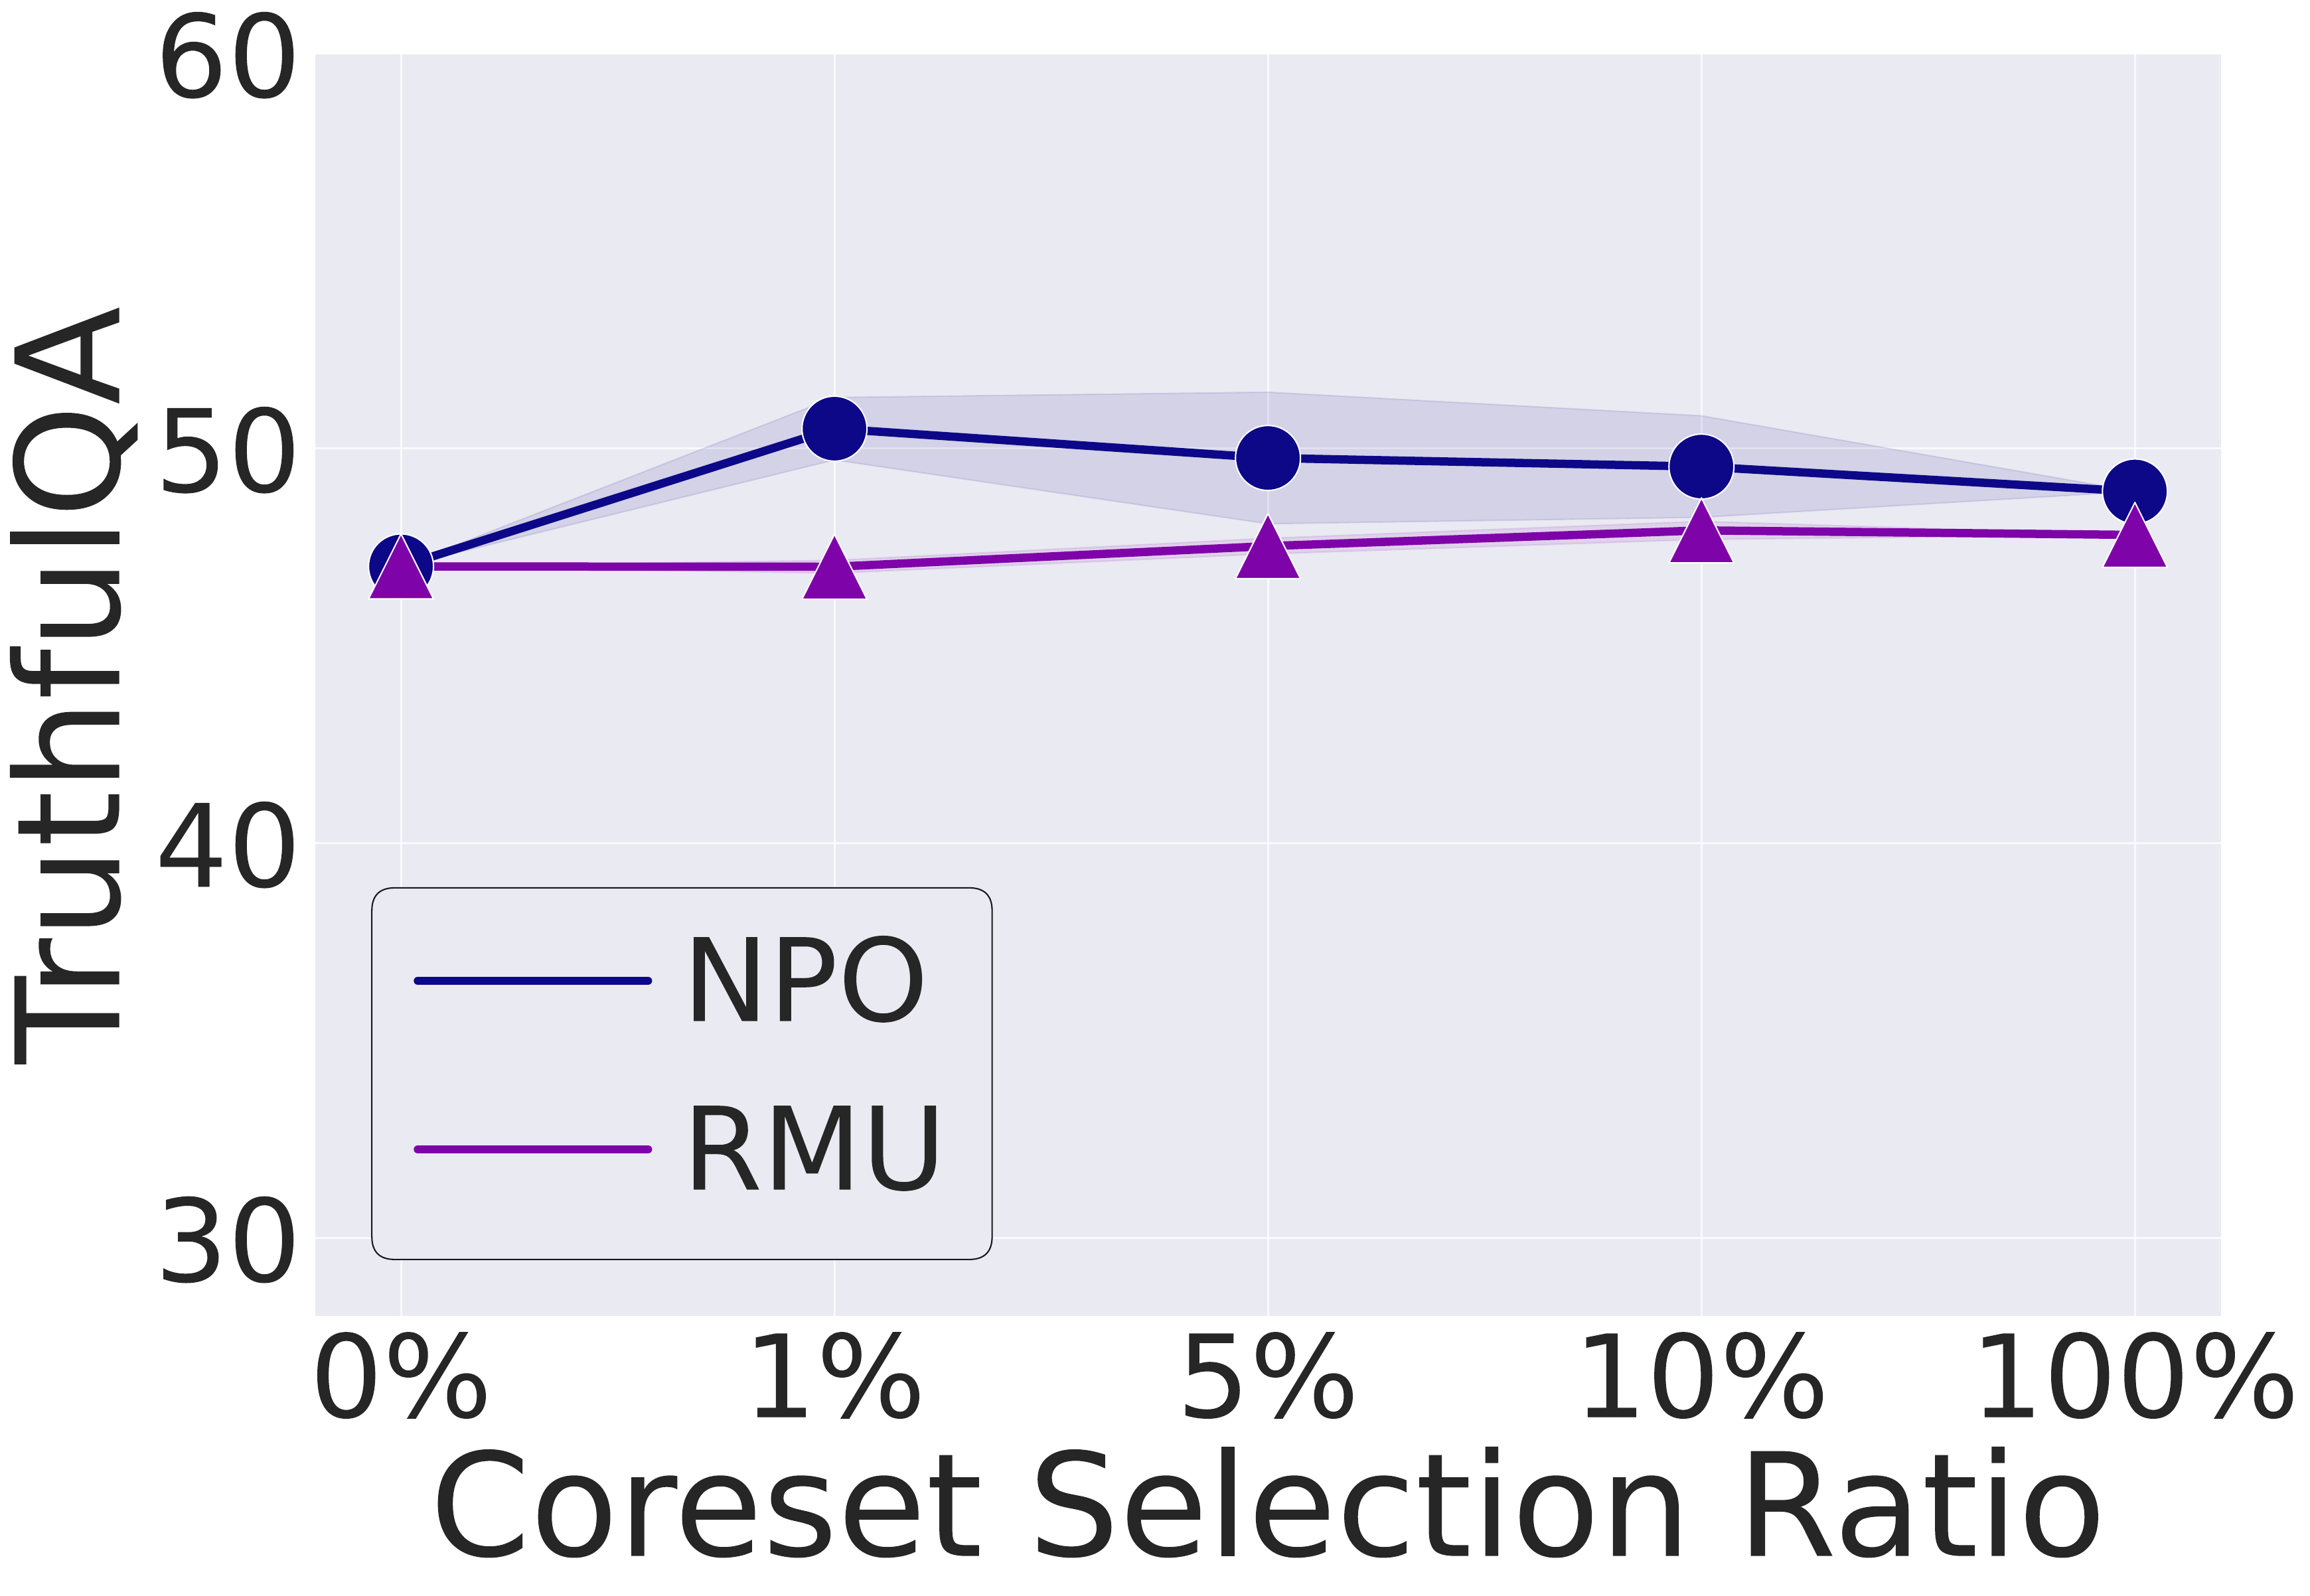} 
  \\
% {\footnotesize{(e) n-Digit Addition, WMDP-Cyber}}
% & {\footnotesize{(f) n-Digit Subtraction, WMDP-Cyber}}
% & {\footnotesize{(g) Truthful QA, WMDP-Cyber}} 
% \\
{\footnotesize{(e) Addition, WMDP-Cyber}}
& {\footnotesize{(f) Subtraction, WMDP-Cyber}}
& {\footnotesize{(g) TruthfulQA, WMDP-Cyber}} 
\\
\end{tabular}
\vspace*{-2mm}
\caption{\small{Additional utility evaluation performance for \random{}-coreset unlearned models using NPO and RMU under  Zephyr-7B-$\beta$. (a)-(d) correspond to the performance of a specific utility evaluation (Addition, Subtraction, Truthful QA) of models unlearned using WMDP-Bio or WMDP-Cyber. Here `Addition' refers to n-digit addition (n=2,3,4,5) and `Subtraction' refers n-digit subtraction (n=2,3,4,5), where the accuracies are averaged over n.
The unlearning task and setting follow the same configuration as  in Fig.\,\ref{fig: random_sufficient}.
}}
  \label{fig: additional utility}
\end{figure}

%\SP{
% In \reffig{fig: additional utility}, we report the zero-shot accuracy of the aforementioned utility metrics for \random{}-based coreset-unlearned models using RMU and NPO on WMDP. RMU consistently maintains strong utility across all evaluations, regardless of the coreset selection ratio. In contrast, NPO shows higher variance; however, we observe that for $n$-digit addition and subtraction, performance may benefit from using a 10\% coreset in the WMDP-Cyber setting.
%At the same time, NPO can degrade utility at 5\% coreset selection ratio. 
%}
% We attribute this to NPO being a divergence-driven method
